# Supplementary material for: Nuclear matrix elements for neutrinoless double beta decays and spin-dipole giant resonances
Source: arXiv:2202.00361 source file (2022-02-14)
Supplement: Supplementary file 1 [file 7_appendix.tex]

% appendix about theories and methods

\appendix
\section{Additional Discussions and Future Directions}
\label{sec:discussion_future_appdx}
\subsection{Discussions on HAO and its Limitations}
\label{sec:discussion_limitation_appdx}
\textbf{Discussions on HAO  and future implications.} It is widely received that it is difficult to give a proper definition of unnoticeability for graphs (More details are also given in Appendix~\ref{sec:threat_model_reason_appdx}).
Based on earliest unnoticeability constraints on degree distribution changes~\citep{nettack,metattack},
empirical observations that graph adversarial attacks may change some feature statistics and connect dissimilar neighbors are identified,
and leveraged as heuristics to develop robust GNNs~\citep{advsample_deepinsights,gnn_svd,gnnguard,prognn}.
Though empirically effective, however, few of them provide theoretical explanations or relate this phenomenon to unnoticeability.
In this work, starting from the comparison of GMA and GIA, we identified GIA would lead to severe damage to the original homophily.
Furthermore, the relatively high flexibility of GIA amplifies the destruction and finally results in the break of homophily unnoticeability.
The main reason for this phenomenon is mainly because of the poorly defined unnoticeability in graph adversarial attack.
Without a proper definition, the developed attacks tend to the shortcut to incur damage instead of capturing the true underlying vulnerability of GNNs.
Consequently, using these attacks to evaluate robustness of GNNs will bring unreliable results thus hindering the development of trustworthy GNNs.

To be more specific, due to the poor unnoticeability constraint for graph adversarial learning, the developed attacks tend to leverage the shortcuts to greatly destroy the original homophily, which leads to the break of unnoticeability. Thus, using homophily defenders can easily defend these seemingly powerful attacks, even with a simple design, which however brings us unreliable conclusions about the robustness of homophily defenders.
Essentially, HAO penalizes GIA attacks that take the shortcuts, and retain their unnoticeability in terms of homophily.
Thus, HAO mitigates the shortcut issue of GIA attacks, urges the attacks to capture the underlying vulnerability of GNNs
and brings us a more reliable evaluation result, from which we know simple homophily defenders are essentially not robust GNNs.

In addition, the proposed realization of unnoticeability check for adversarial attacks provides another approach to instantiate the unnoticeability. Especially for the domains that we can hardly leverage inductive bias from human, we can still try to identify their homophily, or the underlying rationales/causality of the data generation process, e.g., grammar correctness, fluency and semantics for natural languages, to instantiate the unnoticeability constraint with the help of external examiners. Since people are likely to be more sensitive to quantitative numbers like accuracy, those external examiners can be conveniently leveraged to the corresponding benchmark or leaderboards to further benefit the community.

\textbf{Limitations of HAO and future implications.} Since HAO are mostly developed to preserve the homophily unnoticeability, it counters the greedy strategy of attacks without HAO that destroys the homophily to incur more damage.
Therefore, it will inevitably reduce the damage of the attacks without HAO against vanilla GNNs.
As observed from the experiments, we find HAO essentially trades the attack performance when against vanilla GNNs for the performance when against homophily defenders.
As Fig.~\ref{fig:ablation_hao_coe} shows, the trade-off effects can be further amplified with a large coefficient lambda in HAO.
As also shown by Fig.~\ref{fig:ablation_node_budgets} and Fig.~\ref{fig:ablation_edge_budgets}, when against vanilla GNNs, compared with GIA without HAO, GIA with HAO show fewer threats.
In certain cases, the trade-off might generate the performance of attacks.
Thus, it calls for more tailored optimization methods to solve for better injection matrix and node features in the future. Moreover, the trade-off effects also reflect the importance of homophily to the performance of node classifications and the utility of homophily unnoticeability, where we believe future theoretical works can further study this phenomenon and reveal the underlying causality for node classification or even more other downstream tasks. Thus, we can develop more robust and trustworthy neural graph models that do not depend on spurious correlations to perform the task.

In addition, as homophilous graph is the most common class of graph benchmarks for node classification~\citep{cora,citeseer,ogb,grb}, our discussions are mostly focused on this specific class of graphs.
However, when applying HAO to other classes of graphs such as non-attributed graphs, a direct adaption of HAO may not work.
Nevertheless, if the underlying information for making correct predictions still resemble the homophily property,
for example, in a non-attributed graph, nodes with similar structures tend to have similar labels,
it is still promising to introduce the node features with node embeddings, derive a new definition of homophily and apply HAO.
Moreover, recently disassortative graphs appear to be interesting to the community~\citep{geom_gcn,beyond_homophily},
which exhibit heterophily property that neighbors tend to have dissimilar labels, in contrast to homophily.
We conduct an investigation on this specific class of graphs and detailed results are given in Table~\ref{tab:eval_non_targeted_nonhomo_appdx},
from which we surprisingly find HAO still maintains the advance when incorporating various GIA attacks.
The reason might be that GNNs and GIA with HAO can still implicitly learn the homophily such as similarity between class label distributions~\citep{is_homophily_necessity}, even without explicit definitions.
To summarize, we believe future extension of HAO to other classes of graphs is another interesting direction.

Besides, the discussions in this paper are only considered the relationship between adversarial robustness and homophily.
However, label noises are another widely existing threats that are deserved to be paid attention to~\citep{label_noise_reweight,coteaching,sigua,label_noise_survey}.
Essentially, our discussions in Appendix~\ref{sec:Memorization Effects of GNNs}
are also closely related to the vulnerability of GNNs to label noises, where GNNs can still achieve
near perfect fitting to the datasets with full label noises. Thus, it is desirable to broader the attention
and discussion to include the label noises when developing trustworthy GNNs.

\subsection{More Future Directions}
\label{sec:future_direction_appdx}

Besides the future implications inspired from the limitations of HAO, we believe there are also many promising future works that could be built upon HAO.

\textbf{Rethinking the definition of unnoticeability in adversarial robustness.}
Though the study of adversarial robustness was initially developed around the deep learning models on image classification~\citep{intriguing,fgsm,pgd},
images and classification are far from the only data and the task we want to build neural networks for.
Deep learning models are widely applied to other types of data, such as natural languages and graphs,
where human inductive bias can hardly be leveraged to elaborate a proper definition of unnoticeability.
Moreover, for more complicated tasks involving implicit reasoning, even in the domain of images,
the original definition of unnoticeability, i.e., L-p norm, may not be sufficient to
secure all shortcuts that can be leveraged by adversaries.
How to establish and justify a proper definition of unnoticeability in these domains and tasks,
is critical for developing trustworthy deep learning models.


\textbf{Applications to other downstream tasks.}
Given the wide applications of GNNs, we believe the studies on the robustness of GNNs should be extended to other downstream tasks, such as link predictions and graph clustering.
Specifically, when with a different task objective, it is interesting to find whether the underlying task still depend on the homophily property and
how the different optimization objectives affect the attack optimization trajectory.


\textbf{Attack with small budgets.}
In real-life scenarios, the budgets of the adversary may be limited to a small number.
It is interesting to study how to maximize the damage given limited budgets and its interplay between homophily.
For example, how to locate the most vulnerable targets. We show an initial example through ATDGIA.

\textbf{Mix-up attack of GMA and GIA.}
In real-life scenarios, both GMA and GIA could happen while with different budget limits.
It is interesting to see whether and how they could be combined to conduct more powerful attacks.

\textbf{Injection for defense.}
Actually, not only attackers can inject extra nodes, defenders can also inject some nodes to
promote the robustness of the networks. For example, according the Proposition.~\ref{thm:gia_cer_robo},
nodes with higher degrees, higher MLP decision margin and higher homophily tend more unlikely to be attacked.
Hence, defenders may directly inject some nodes the promote the above properties of vulnerable nodes.

\textbf{Attacks on more complicated and deep GNNs.}
Most existing graph adversarial works focus on analyzing linearized GNNs and apply the discoveries to more complex cases.
However, with the development of deep learning and GNNs, some models with complicated structures fail to fit those theories. For example, methods developed by studying linearized GNNs can hardly adapt to GNNs with normalizations as also revealed from our experiments. Then they can even more hardly be adapted to more complex models such as Transformers. On the other hand, most graph adversarial studies only focus on relatively shallow GNNs. Different from other deep learning models, as GNNs go deep, besides more parameters, they also require an exponentially growing number of neighbors as inputs. How the number of layers would affect their robustness and the threats of attacks remain unexplored.
From both theoretical and empirical perspectives, we believe it is very interesting to study the interplay between the number of GNN layers and homophily, in terms of adversarial robustness and threats, and how to leverage the discoveries to probe the weakness of complicated models.

\textbf{Reinforcement Learning based GIA.}
Reinforcement learning based approaches are shown to exhibit promising performances in previous mixed settings~\citep{rls2v,nipa}.
Though we exclude them for the efforts needed to adapt them to our setting, we believe it is promising and interesting to
incorporate reinforcement learning to develop more tailored injection strategies and vulnerable nodes selection.
Meanwhile, it is also interesting to explore how to leverage the idea of SeqGIA proposed in Sec.~\ref{sec:gia_hao} to reduce the computation overhead of
reinforcement learning approaches and enhance their scalability.


\section{More Details and Reasons about the Graph Adversarial Attack Setting}
\label{sec:adv_setting_appdx}
We provide more details about the perturbation constraints
and the threat model used in Sec.~\ref{sec:adv_setting}.

\subsection{Perturbation Constraints}
Following previous works~\citep{nettack,tdgia}, Graph adversarial attacks can be characterized into graph modification attacks and graph injection attacks by their perturbation constraints.
Moreover, we adopt standardization methods (i.e., arctan transformation) following Graph Robustness Benchmark~\citep{grb} on input features $X$.

\textbf{Graph Modification Attack (GMA).} GMA generates $\gG'$ by modifying the graph structure $A$ and the node features $X$ of the original graph $\gG$. The most widely adopted constraints in GMA is to limit the number of perturbations on $A$ and $X$, denoted by $\triangle_A$ and $\triangle_X$, respectively, as:
\begin{equation}
	\label{eq:gma_cons}
	\triangle_A+\triangle_X\leq \triangle\in\sZ, \norm{A'-A}_0 \leq \triangle_A\in \sZ, \norm{X'-X}_\infty \leq \epsilon \in \R,
\end{equation}
where the perturbation on $X$ is bounded by $\epsilon$ via L-p norm, since we are using continuous features.


\textbf{Graph Injection Attack (GIA).} Differently, GIA generates $\gG'$ by injecting a set of malicious nodes $V_{\text{atk}}$ as:
\begin{equation}
	X'=\begin{bmatrix}
		\ X\hfill        \\
		\ X_{\text{atk}} \\
	\end{bmatrix},
	A'=\begin{bmatrix}
		\ A\hfill          & A_{\text{atk}} \\
		\ A_{\text{atk}}^T & O_{\text{atk}} \\
	\end{bmatrix},
\end{equation}
where $X_{\text{atk}}$ is the features of the injected nodes, $O_{\text{atk}}$ is the adjacency matrix among injected nodes, and $A_{\text{atk}}$ is the adjacency matrix between the injected nodes and the original nodes. Let $d_u$ denote the degree of node $u$, the constraints in GIA are:
\begin{equation}
	\label{eq:gia_cons}
	|V_{\text{atk}}| \leq \triangle\in\sZ, \ 1\leq d_u\leq b\in\sZ,
	X_{u} \in \mathcal{D}_X \subseteq \R^d,
	\forall u\in V_{\text{atk}},
\end{equation}
where the number and degrees of the injected nodes are limited, $\mathcal{D}_X=\{C\in\R^d,\min(X)\cdot\mathbf{1}\leq C\leq \max(X)\cdot\mathbf{1} \}$ where $\min(X)$ and $\max(X)$ are the minimum and maximum entries in $X$ respectively.
In other words, each entry of the injected node features are bounded within the minimal entry and maximal entry of the original node feature matrix, following previous setting~\citep{tdgia}.

\subsection{Threat Model}
\label{sec:threat_model_appdx}
We adopt a unified setting which is also used by Graph Robustness Benchmark~\citep{grb},
that is evasion, inductive, and black-box. Next we will elaborate more details and reasons for adopting the setting.

\subsubsection{Details of the Threat Model}
\label{sec:threat_model_detail_appdx}
\textbf{Evasion.} The attack only happens at test time, which means that defenders are able to obtain the original clean graph $\gG_{\text{train}}$ for training, while testing on a perturbed graph $\gG'$.
The reasons for adopting the evasion setting is as shown in Appendix~\ref{sec:threat_model_reason_appdx}.

\textbf{Inductive.} The training and testing of GNNs is performed in an inductive manner. Specifically, $f_\theta$ is trained on the (sub) training graph $\gG_{\text{train}}$, which is consist of
the training nodes with their labels and the edges among training nodes. While during testing, the model will access the whole graph $\gG_{\text{test}}=\gG$ for inferring the labels of test nodes.
In particular, $\gG$ is consist of all of the nodes and the edges, including $\gG_{\text{train}}$, the test nodes, the edges among test nodes and the edges between training nodes and the test nodes.
In contrast, if the training and testing is performed in a transductive manner, the model can access the whole graph during both training and testing, i.e., $\gG_{\text{train}}=\gG_{\text{test}}=\gG$.
Since we adopt the evasion setting where the adversary may modify the $\gG_{\text{test}}$ during testing,
the GNN has to be learned in an inductive manner. More reasons are as elaborated in Appendix~\ref{sec:threat_model_reason_appdx}.

\textbf{Black-box.} The adversary has no information about the target model, but the adversary may obtain the graph and training labels to train a surrogate model for generating perturbed graph $\gG'$.

Combining all of the above, conducting effective attacks raises special challenges to adversaries, since defenders can adopt the information extracted from training graph $\gG_{\text{train}}$ to learn  more robust hidden representations~\citep{robustgcn}, or learn to drop noisy edges~\citep{advsample_deepinsights,gnnguard,prognn}, or even perform adversarial training~\citep{laten_adv,dyadv} which is known as one of the strongest defense mechanisms in the domain of images~\citep{fgsm,pgd}.

\subsubsection{Discussions about the Threat Model}
\label{sec:threat_model_reason_appdx}
Different from images where we can adopt the inductive bias from human vision system to use numerical constraints, i.e., L-p norm, to bound the perturbation range~\citep{fgsm,pgd}, we cannot use similar numerical constraints to define the unnoticeability for graphs, as they are \textit{weakly correlated} to the information required for node classification. For example, previous work~\citep{nettack} tries to use node degree distribution changes as the unnoticeability constraints. However, given the same degree distribution, we can shuffle the node features to generate multiple graphs with completely different semantic meanings, which disables the functionality of unnoticeability.

Because of the difficulty to properly define the unnoticeability for graphs, adopting a poisoning setting in graph adversarial attack will enlarge the gap between research and practice. Specifically, poisoning attacks require an appropriate definition of unnoticeability so that the defenders are able to distinguish highly poisoned data from unnoticeable poisoned data and the original data. Otherwise, attackers can always leverage some underlying shortcuts implied by the poorly defined unnoticeability, i.e., homophily in our case, to perform the attacks, since the defenders are blind to these shortcuts. On the other hand, leveraging shortcuts may generate data which is unlikely to appear in real-world applications. For example, in a citation network, medical papers are unlikely to cite or be cited by linguistic papers while the attacks may modify the graphs or inject malicious nodes to make medical papers cite or be cited by lots of linguistic papers, which is apparently impractical. Using these attacks to evaluate the robustness of GNNs may bring unreliable conclusions, i.e., homophily defenders in our case, which will greatly hinders the development of the trustworthy GNNs.

Moreover, under a poor unnoticeability definition, without the presence of the original data, defenders have no idea about to what extent the data is poisoned and whether the original labels remain the correspondence. Furthermore, it is well-known that neural networks have universal approximation power~\citep{mlp_approx}, thus can easily overfit the training set~\citep{dl_book}, or even \textit{memorize} the labels appeared during training~\citep{memorization}. As a generalization from deep learning models to graphs, GNNs tend to exhibit similar behaviors, which is shown empirically in our experiments (See Appendix \ref{sec:Memorization Effects of GNNs} for details). Thus, even trained on a highly poisoned graph, GNNs may still converge to 100\% training accuracy, even though the correspondence between the data and the underlying labels might be totally corrupted. In this case, defenders can hardly distinguish whether the training graph is perturbed hence unlikely to make any effective defenses. Besides, studying the robustness of GNNs trained from such highly poisoned graphs seems to be impractical, since real world trainers are unlikely to use such highly poisoned data to train GNNs.

While in an evasion setting, the defenders are able to use the training graph to tell whether the incoming data is heavily perturbed and make some effective defenses, even simply leveraging some feature statistics~\citep{advsample_deepinsights,prognn}. Notably, A recent benchmark~\citep{grb} also has similar positions. Thus, we will focus on the evasion setting in this paper.


Given the evasion setting, GNNs can only perform inductive learning where the test nodes and edges are not visible during training. The reason is that, transductive learning (i.e., the whole graph except test labels is available), requires the training graph and test graph to be the same. However, it can not be satisfied as the adversary will modify the test graph, i.e., changing some nodes or edges during GMA attack, or injecting new malicious nodes during GIA attack. Additionally, inductive learning has many practical scenarios. For example, in an academic network, the graph grows larger and larger day by day as new papers are published and added to the original network. GNN models must be inductive to be applied to such evolving graphs.


\subsection{Memorization Effects of Graph Neural Networks}
\label{sec:Memorization Effects of GNNs}
\begin{figure}[h]
	\centering
	\begin{subfigure}[b]{0.32\textwidth}
		\centering
		\includegraphics[width=\textwidth]{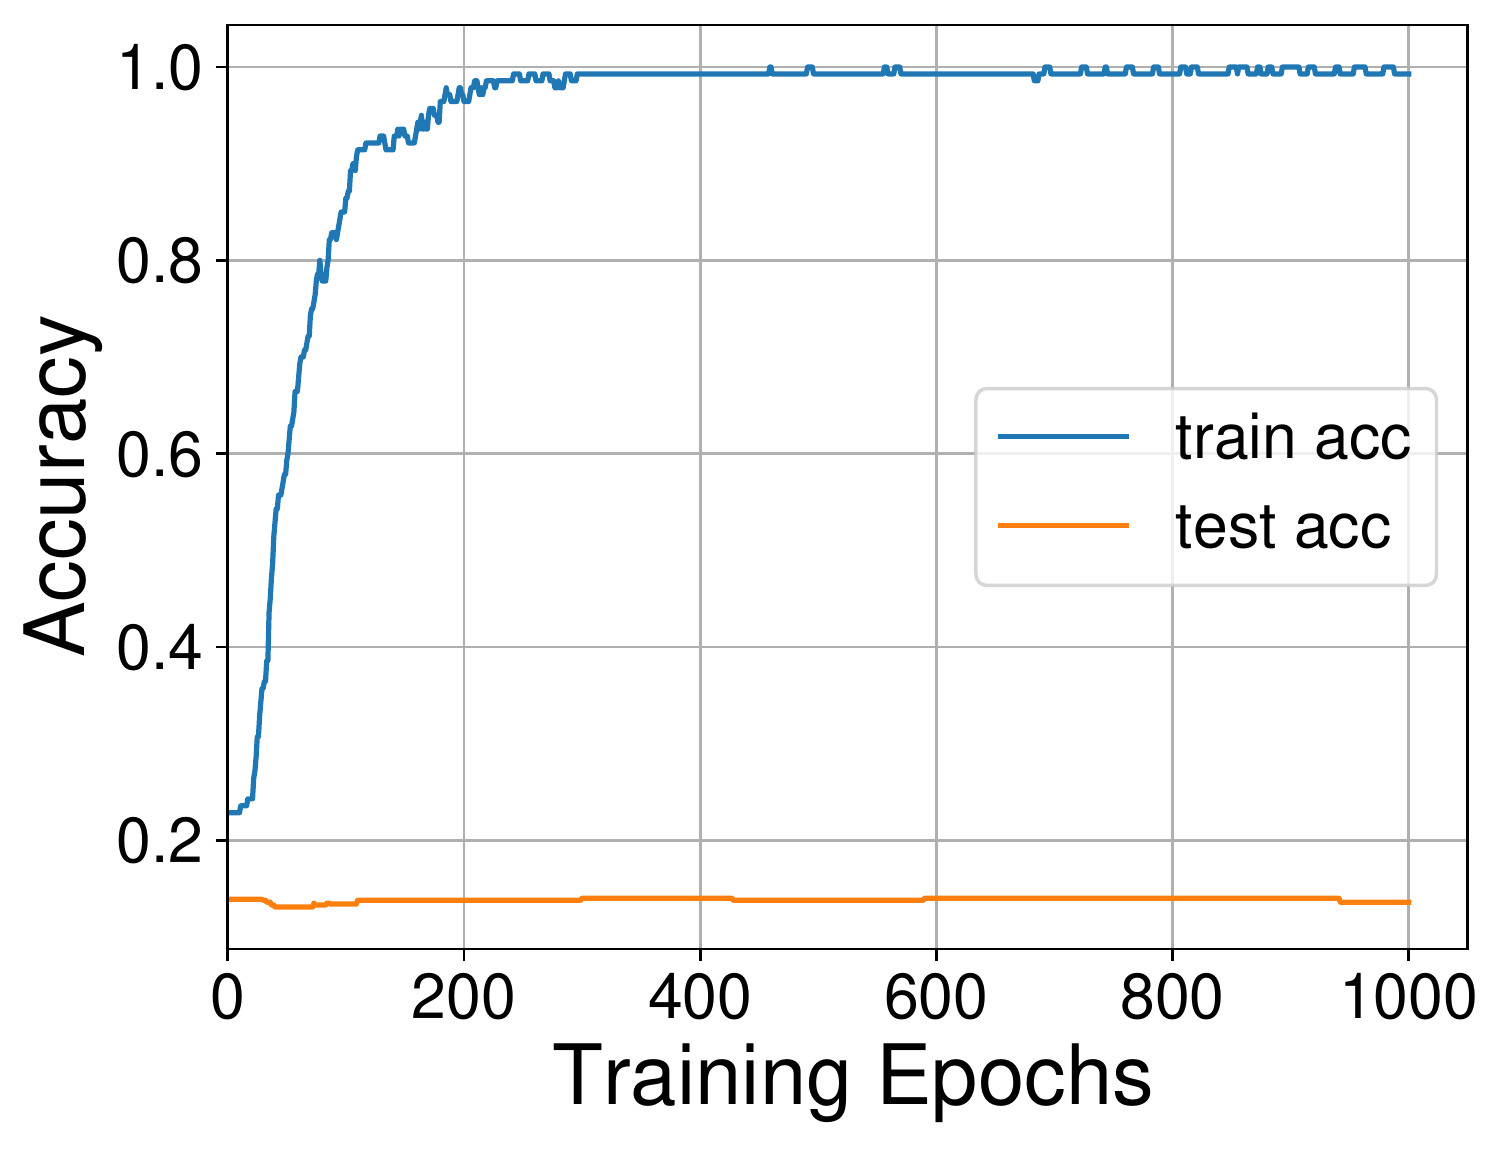}
		\caption{Original labels}
	\end{subfigure}
	\hfill
	\begin{subfigure}[b]{0.32\textwidth}
		\centering
		\includegraphics[width=\textwidth]{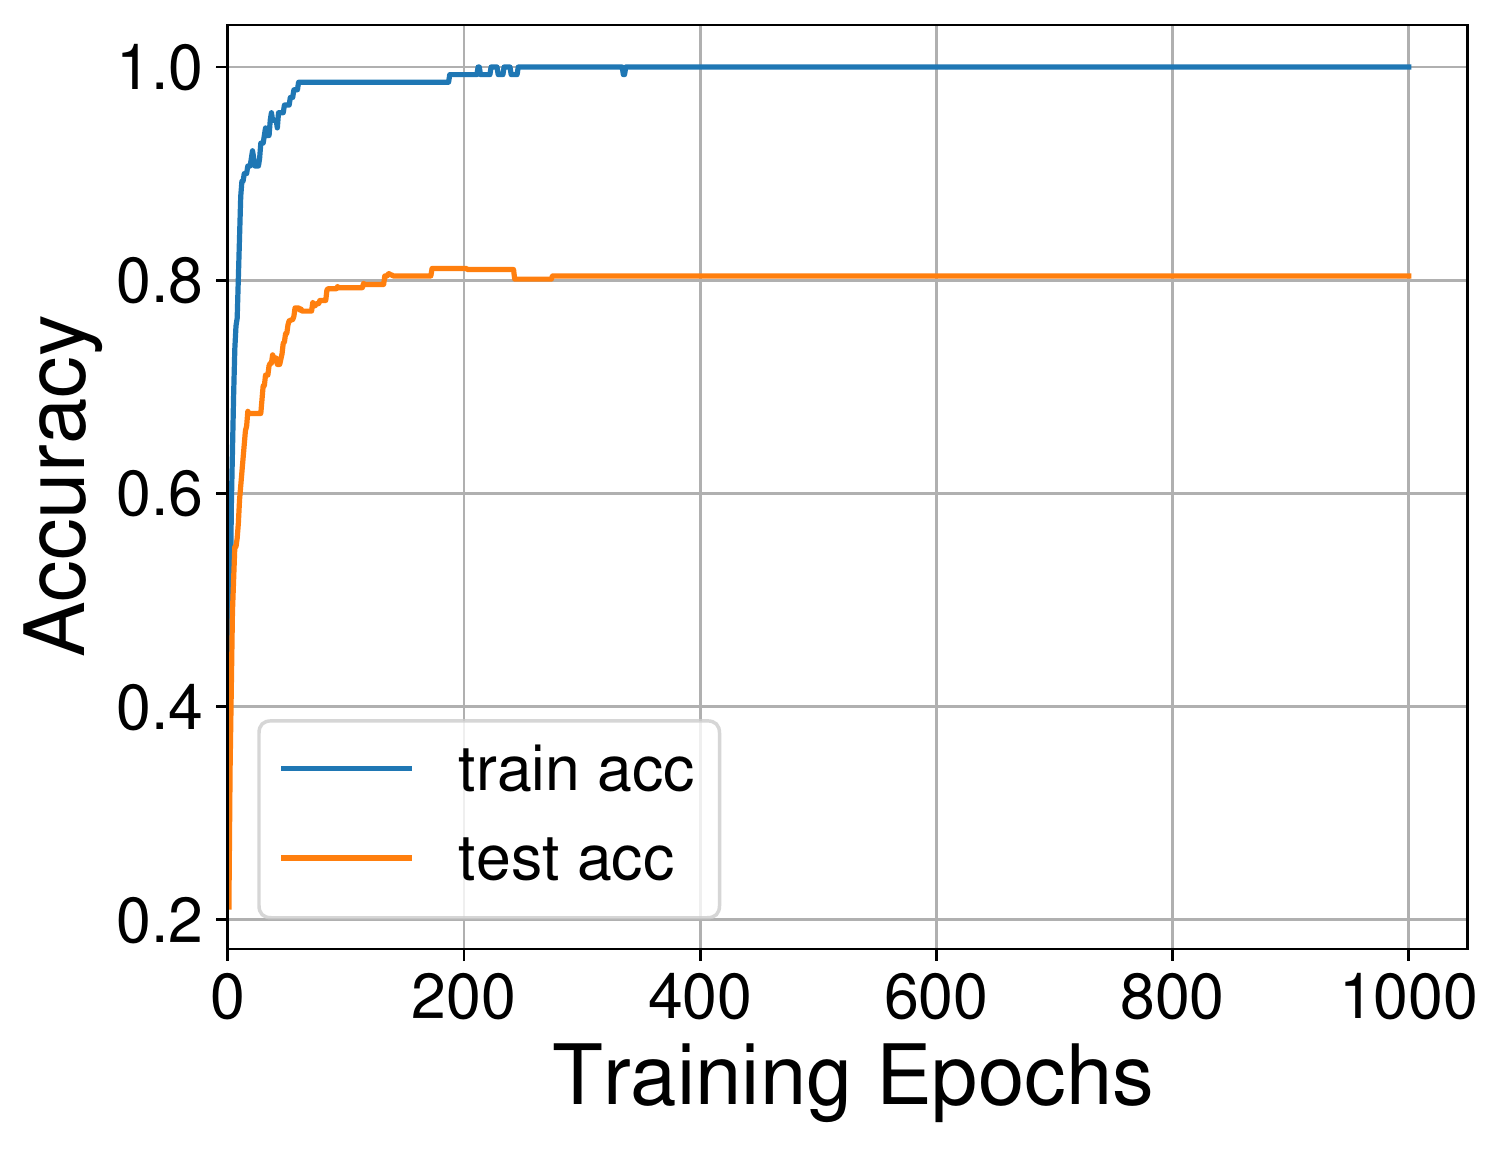}
		\caption{Random labels}
	\end{subfigure}
	\hfill
	\begin{subfigure}[b]{0.32\textwidth}
		\centering
		\includegraphics[width=\textwidth]{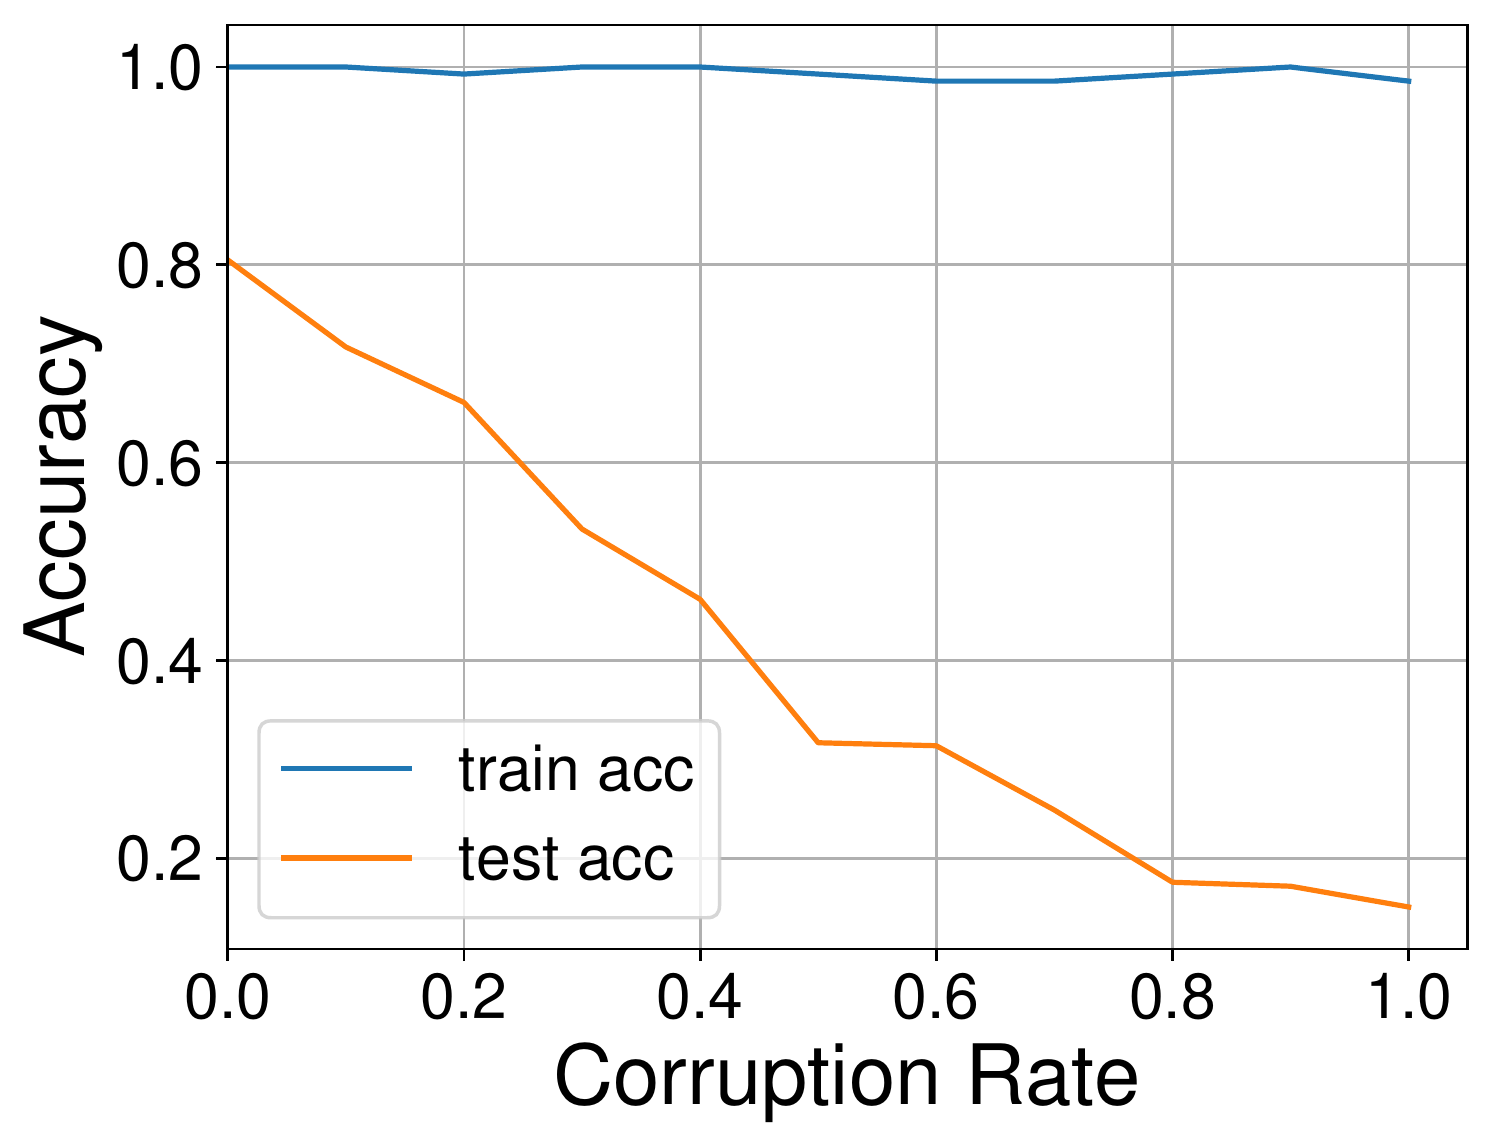}
		\caption{Partial random labels}
	\end{subfigure}
	\caption{Training curve of GCN on Cora with random labels}
	\label{fig:Memorization Effects of GNNs}
\end{figure}
We conduct experiments with GCN \citep{gcn} on Cora \citep{cora}. The architecture we select is a 2-Layer GCN with 16 hidden units, optimized using Adam \citep{adam} with a learning rate of $0.01$ and a $L_2$ weight decay of $5\times10^{-4}$ for the first layer. We train $1000$ epochs and report the training accuracy and test accuracy according to the best validation accuracy. We randomly sample certain percent of nodes from the whole graph and reset their labels. It can be seen from Fig.~\ref{fig:Memorization Effects of GNNs} (b) and (c) that even with all random labels, the training accuracy can reach to nearly $100\%$, which serves as a strong evidence for the existence of memorization effects in GNNs. In other words, even a GNN is trained on a heavily poisoned graph (changes dramatically in the sense of semantic), it can still achieve good training accuracy while the defender has no way to explicitly find it or do anything about it. That is against to the original setting and purpose of adversarial attacks \citep{intriguing,fgsm,pgd}. Thus, it urges the community for a proper solution to the ill-defined unnoticeability in current graph adversarial learning. Till the appearance of a silver bullet for unnoticeability on graphs, evasion attack can serve as a better solution than poisoning attack.

\section{More Details about GIA and GMA Comparison}
\label{sec:gma_gia_comparison_appdx}
\subsection{Implementation of Graph Modification Attack}
Following Metattack~\citep{metattack}, we implement Graph Modification Attack by taking $A$ as a hyper-parameter.
Nevertheless, since we are conducting evasion attack, we do not have meta-gradients but the gradient of $A$ with respect to $\mathcal{L}_\atk$, or $\nabla_{A}\mathcal{L}_\atk$.
Each step, we take the maximum entry in $\nabla_{A}\mathcal{L}_\atk$, denoted with $\max(\nabla_{A}\mathcal{L}_\atk)$, and change the corresponding edge, if it is not contained in the training graph.
Then we perform the perturbation as follows:
\begin{enumerate}[(a)]
	\item If $\max(\nabla_{A}\mathcal{L}_\atk)\leq 0$ and the corresponding entry in $A$ is $0$, i.e., the edge does not exist before, we will add the edge.
	\item If $\max(\nabla_{A}\mathcal{L}_\atk)\geq 0$ and the corresponding entry in $A$ is $1$, i.e., the edge exists before, we will remove the edge.
\end{enumerate}
If the selected entry can not satisfy neither of the above conditions, we will take the next maximum entry to perform the above procedure until we find one that satisfy the conditions.
Here we exclude perturbations on node features given limited budgets, since \cite{advsample_deepinsights} observed the edge perturbations produce more harm than node perturbations.
Besides, as shown in the proof, the damage brought by perturbations on node features is at most the damage brought by a corresponding injection to the targets in GIA,
hence when given the same budgets to compare GMA and GIA, we can exclude the perturbations on nodes without loss of generality.
Note that given the definitions of direct attack and influencer attack in Nettack~\citep{nettack}, our theoretical discussions are applicable to both direct GMA attack and indirect/influencer GMA attack, since the results are derived by establishing mappings between each kind of perturbations in GMA attack that are agnostic to these two types of GMA attacks. Moreover, the GMA attack evaluated in our experiments is exactly the direct attack.
As in our case, all of the test nodes become victim nodes and the adversary is allowed to modify the connections and features of these nodes to perform the attack.

\subsection{Implementation of Graph Injection Attack with Plural Mapping}
GIA with $\mathcal{M}_2$ is implemented based on the GMA above.
For each edge appears in the perturbed graph produced by GMA but does not exist in the original graph, in GIA,
we will inject a node to connect with the corresponding nodes of the edge. After injecting all of the nodes, then we use PGD~\citep{pgd} to optimize the features of the injected nodes.

\section{More Homophily Distributions}
\subsection{Edge-Centric Homophily}
\label{sec:homophily_edge_appdx}
In addition to node-centric homophily (Def.~\ref{eq:homophily_node}), we can also define edge-centric homophily as:
\begin{definition}[Edge-Centric Homophily]
	The homophily for an edge $(u,v)$ can be defined as.
	\begin{equation}
		\label{eq:homophily_edge}
		h_e=\text{sim}(X_u,X_v),
	\end{equation}
	where $\text{sim}(\cdot)$ is also a distance metric, e.g., cosine similarity.
\end{definition}
With the definition above, we can probe the natural edge-centric homophily distribution of real-world benchmarks, as shown in Fig.~\ref{fig:gia_homophily_dist_edge}.
It turns out that the edge-centric homophily distributes follows a Gaussian prior.
However, it seems to be improper to utilize edge-centric homophily to instantiate the homophily unnoticeability for several reasons.
On the one hand, edge similarity does not consider the degrees of the neighbors which is misaligned with the popular aggregation scheme of GNNs.
On the other hand, edge-centric and node-centric homophily basically perform similar functionality to retain the homophily,
but if considering the future extension to high-order neighbor relationships, edge similarity might be harder to extend than node-centric homophily.
Thus, we utilize the node-centric homophily for most of our discussions.
\begin{figure}[ht]
	\centering
	\begin{subfigure}[b]{0.315\textwidth}
		\centering
		\includegraphics[width=\textwidth]{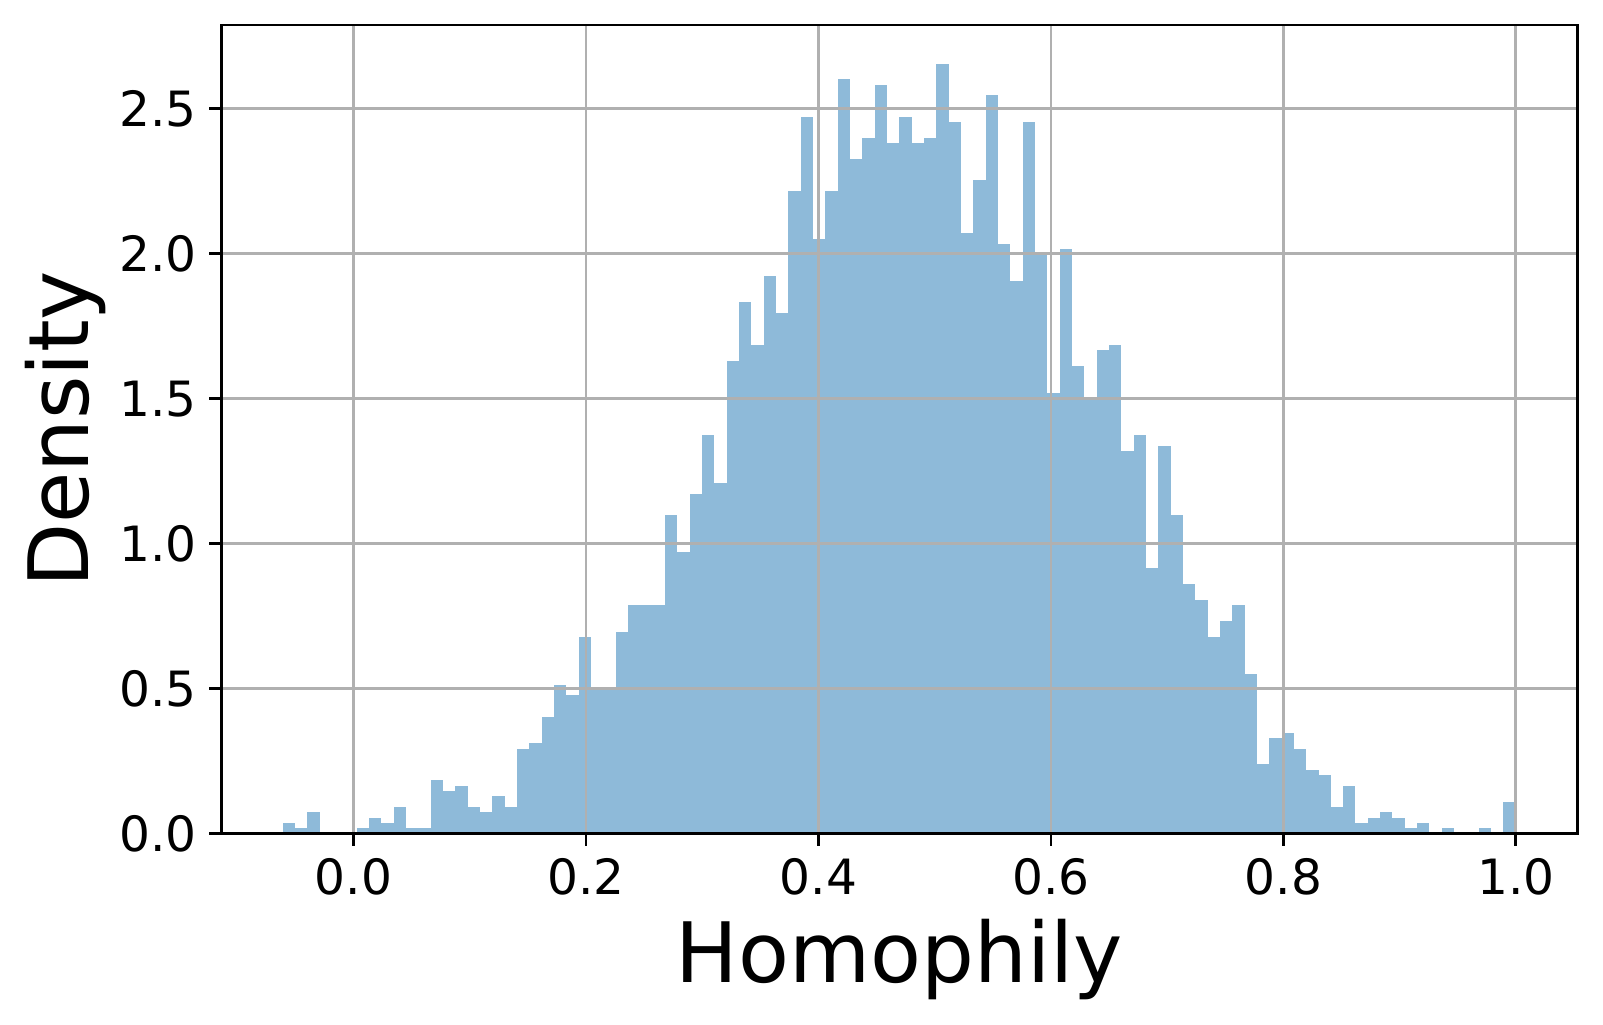}
		\caption{Cora}
	\end{subfigure}
	\begin{subfigure}[b]{0.32\textwidth}
		\centering
		\includegraphics[width=\textwidth]{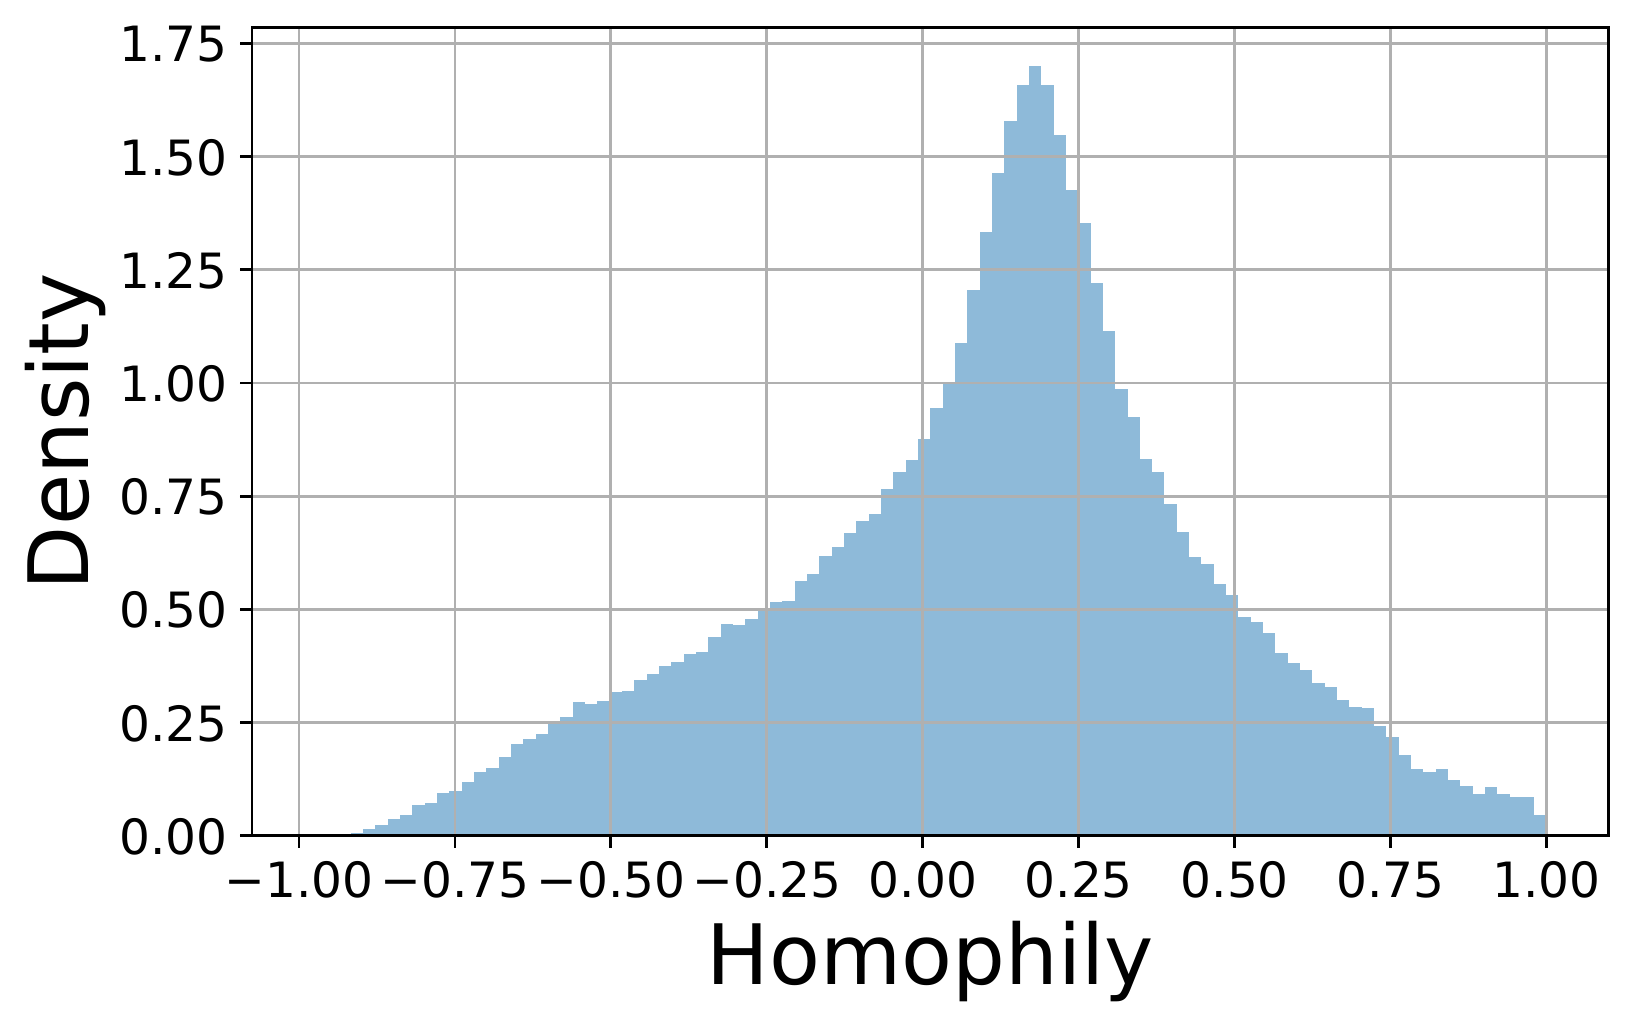}
		\caption{Computers}
	\end{subfigure}
	\begin{subfigure}[b]{0.305\textwidth}
		\centering
		\includegraphics[width=\textwidth]{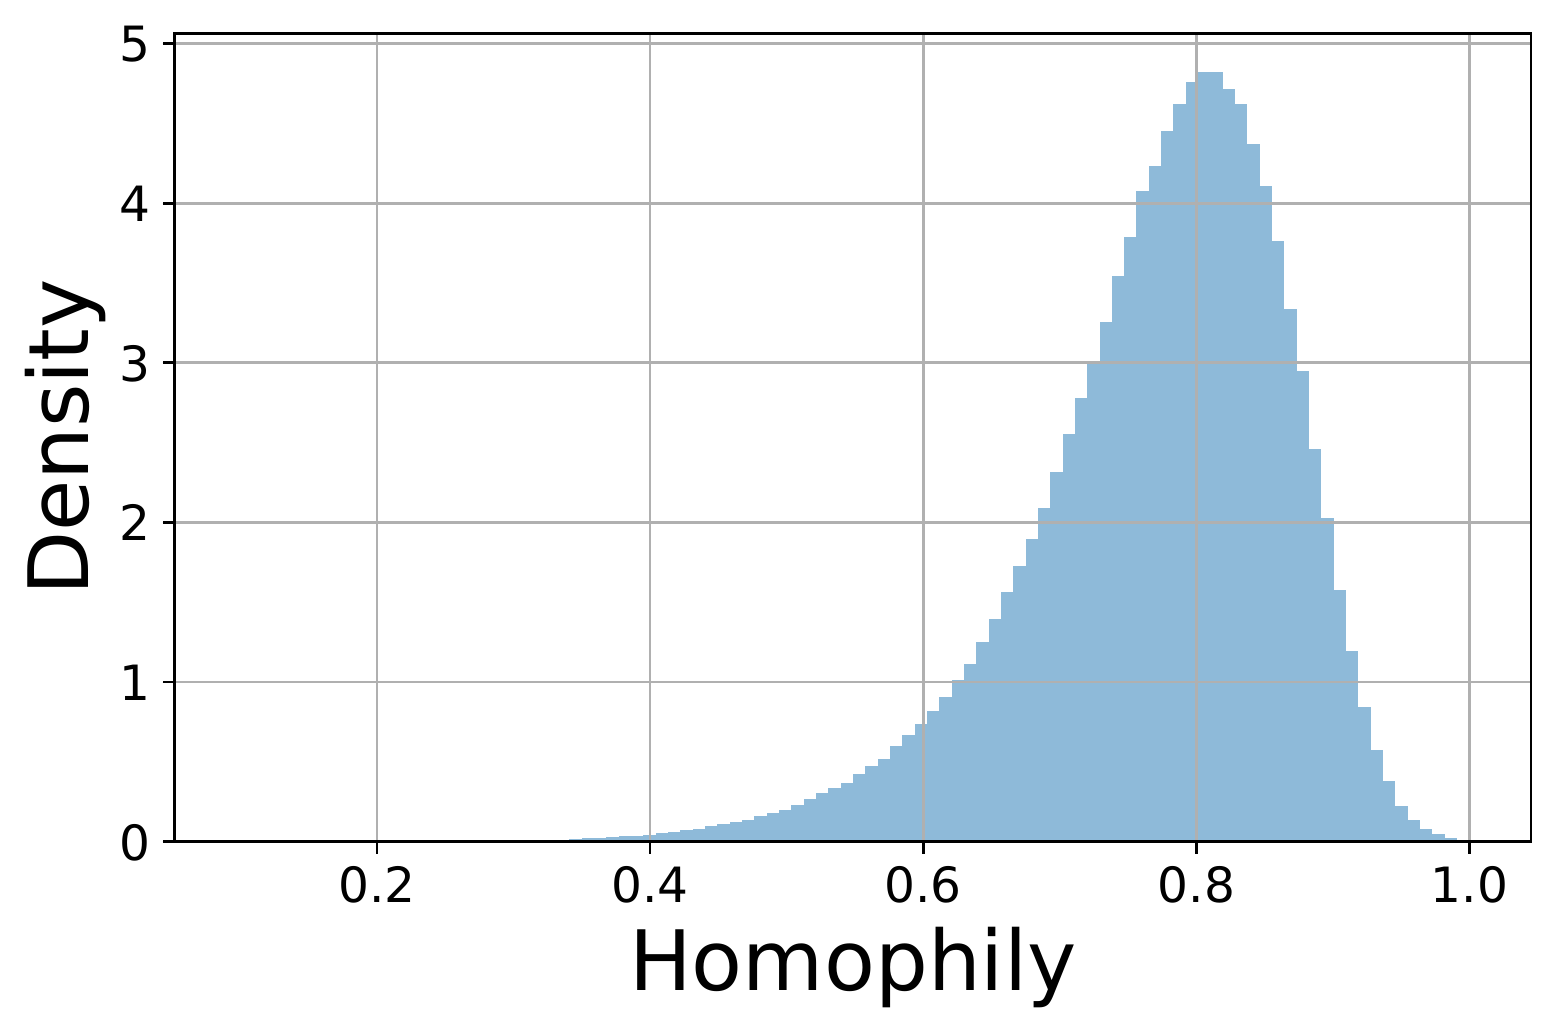}
		\caption{Arxiv}
	\end{subfigure}
	\caption{Edge-Centric homophily distributions}
	\label{fig:gia_homophily_dist_edge}
\end{figure}
\begin{figure}[ht]
	\centering
	\begin{subfigure}[b]{0.32\textwidth}
		\centering
		\includegraphics[width=\textwidth]{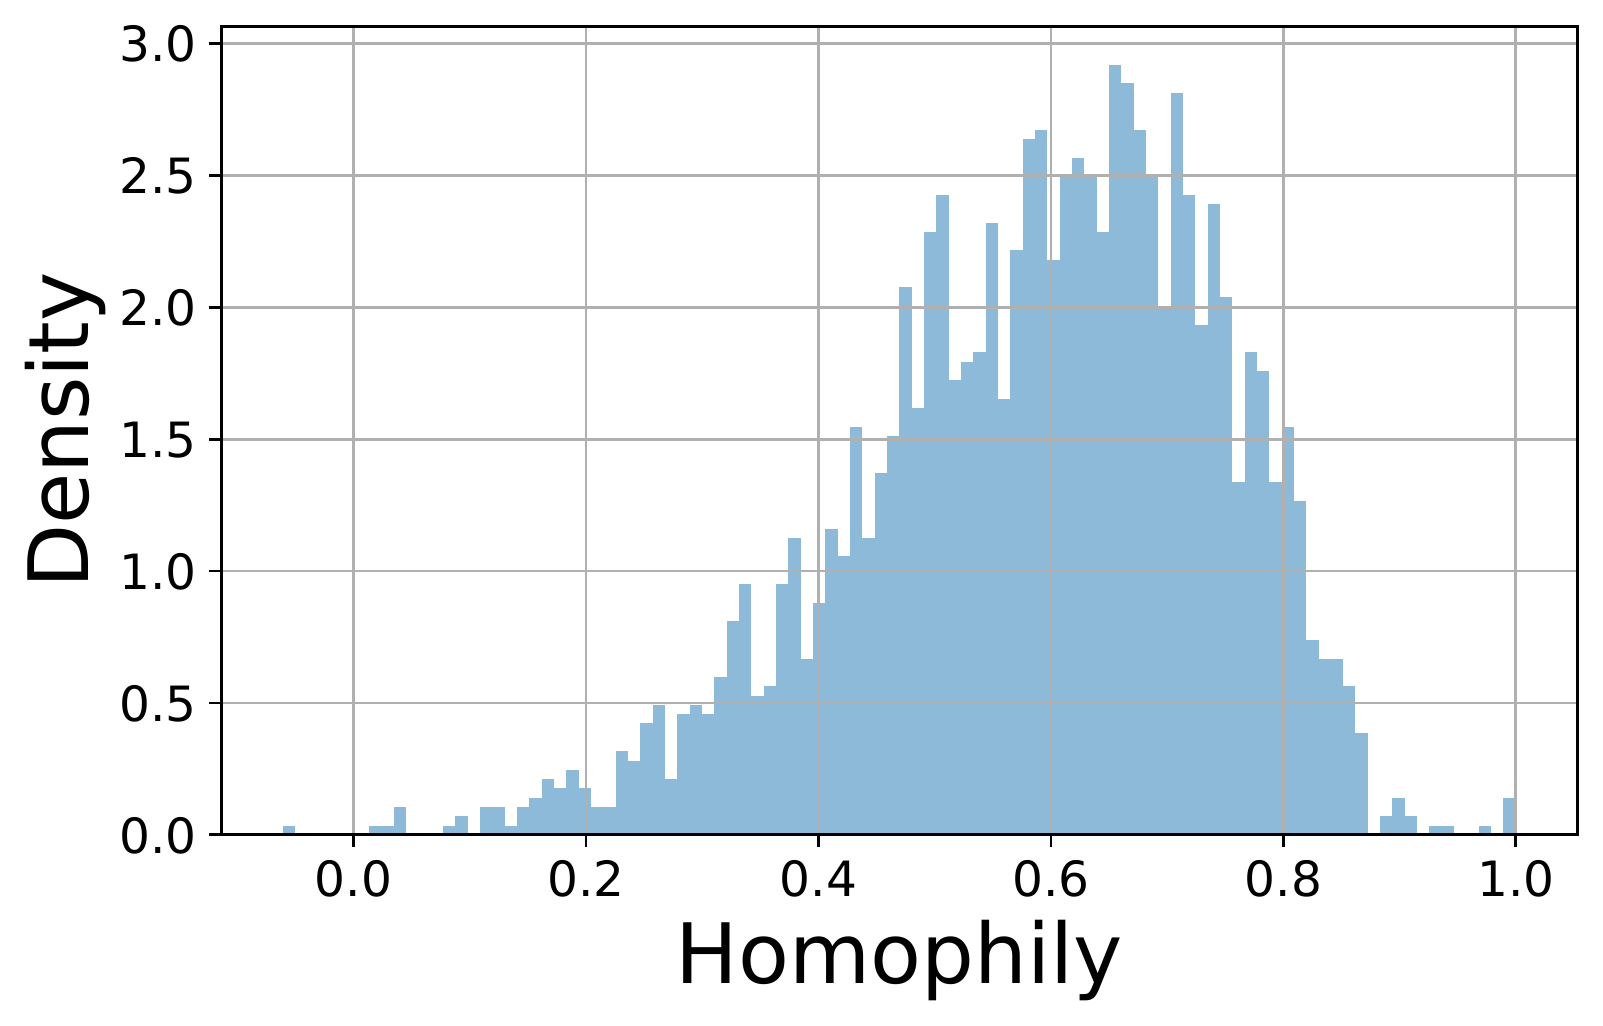}
		\caption{Cora}
	\end{subfigure}
	\begin{subfigure}[b]{0.32\textwidth}
		\centering
		\includegraphics[width=\textwidth]{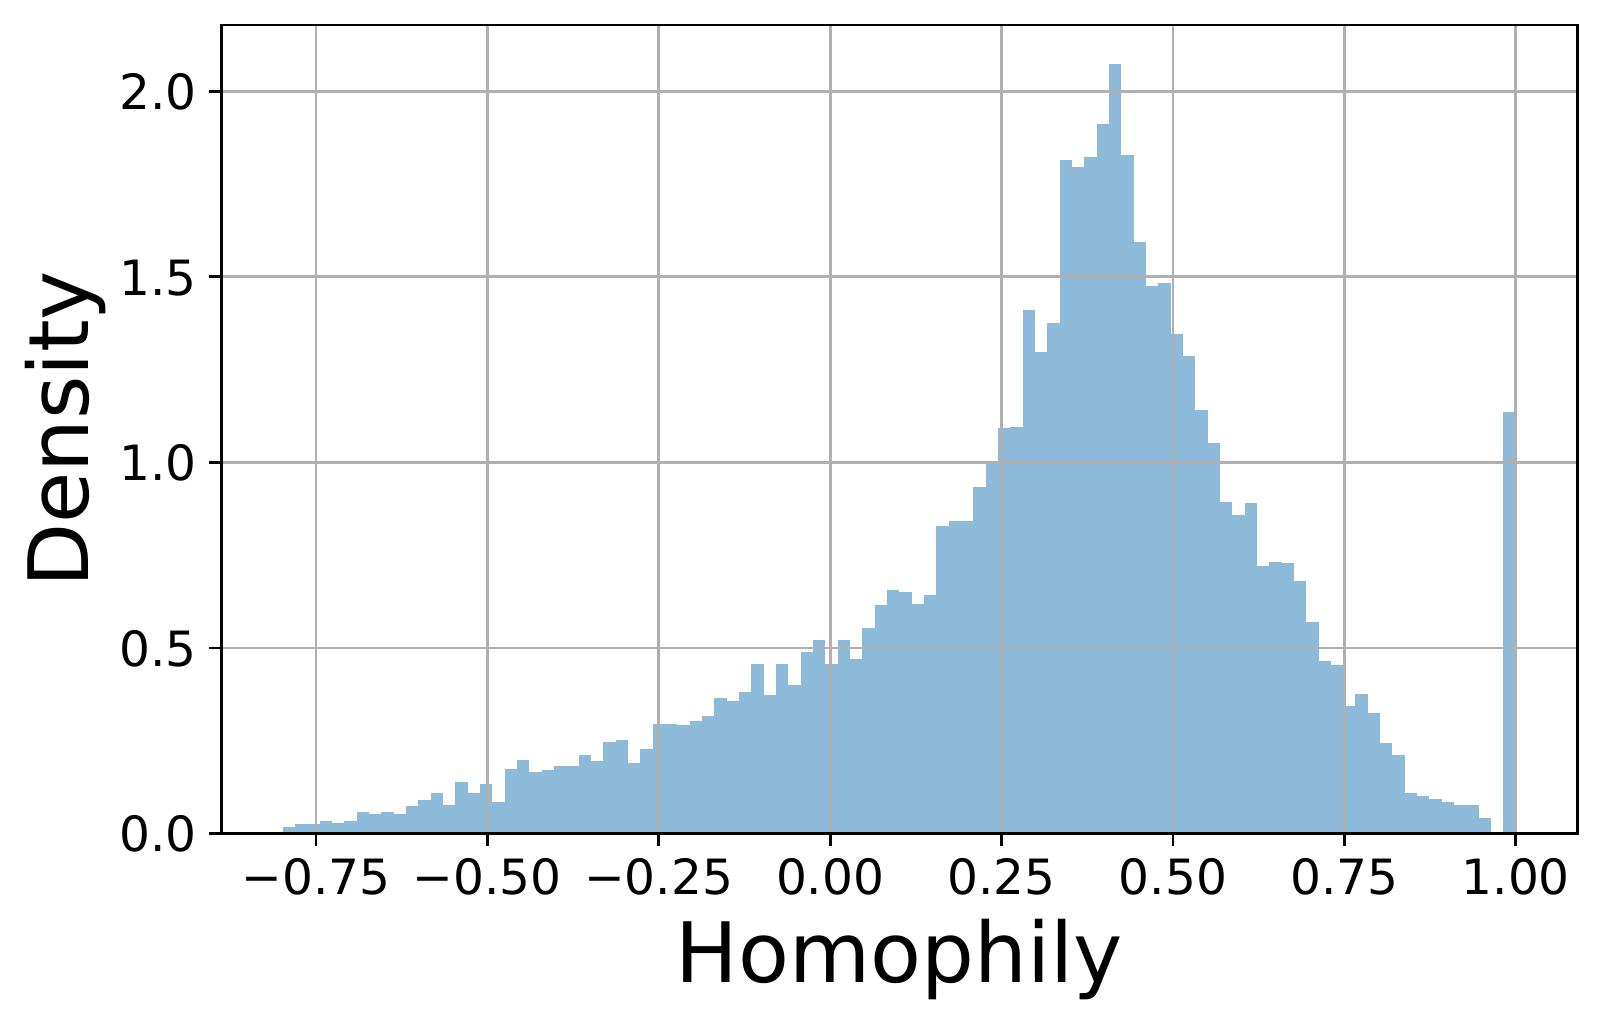}
		\caption{Computers}
	\end{subfigure}
	\begin{subfigure}[b]{0.31\textwidth}
		\centering
		\includegraphics[width=\textwidth]{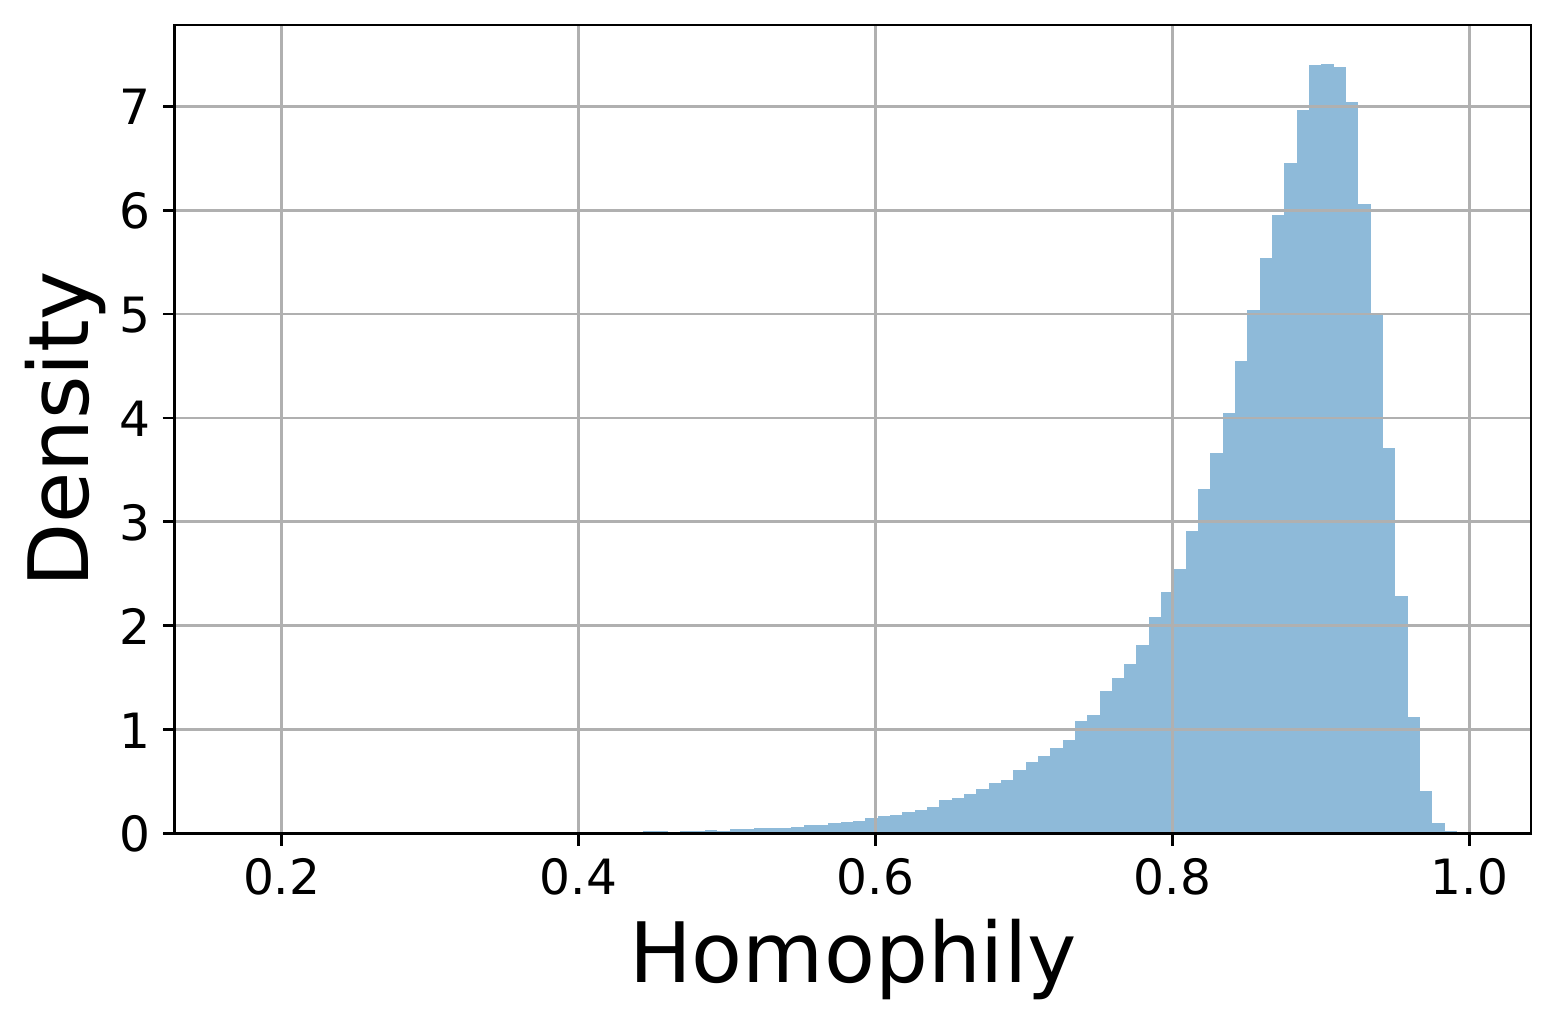}
		\caption{Arxiv}
	\end{subfigure}
	\caption{Homophily distributions before attack}
	\label{fig:gia_homophily_dist_node_atk_appdx_1}
\end{figure}

\begin{figure}[ht]
	\centering
	\begin{subfigure}[b]{0.33\textwidth}
		\centering
		\includegraphics[width=\textwidth]{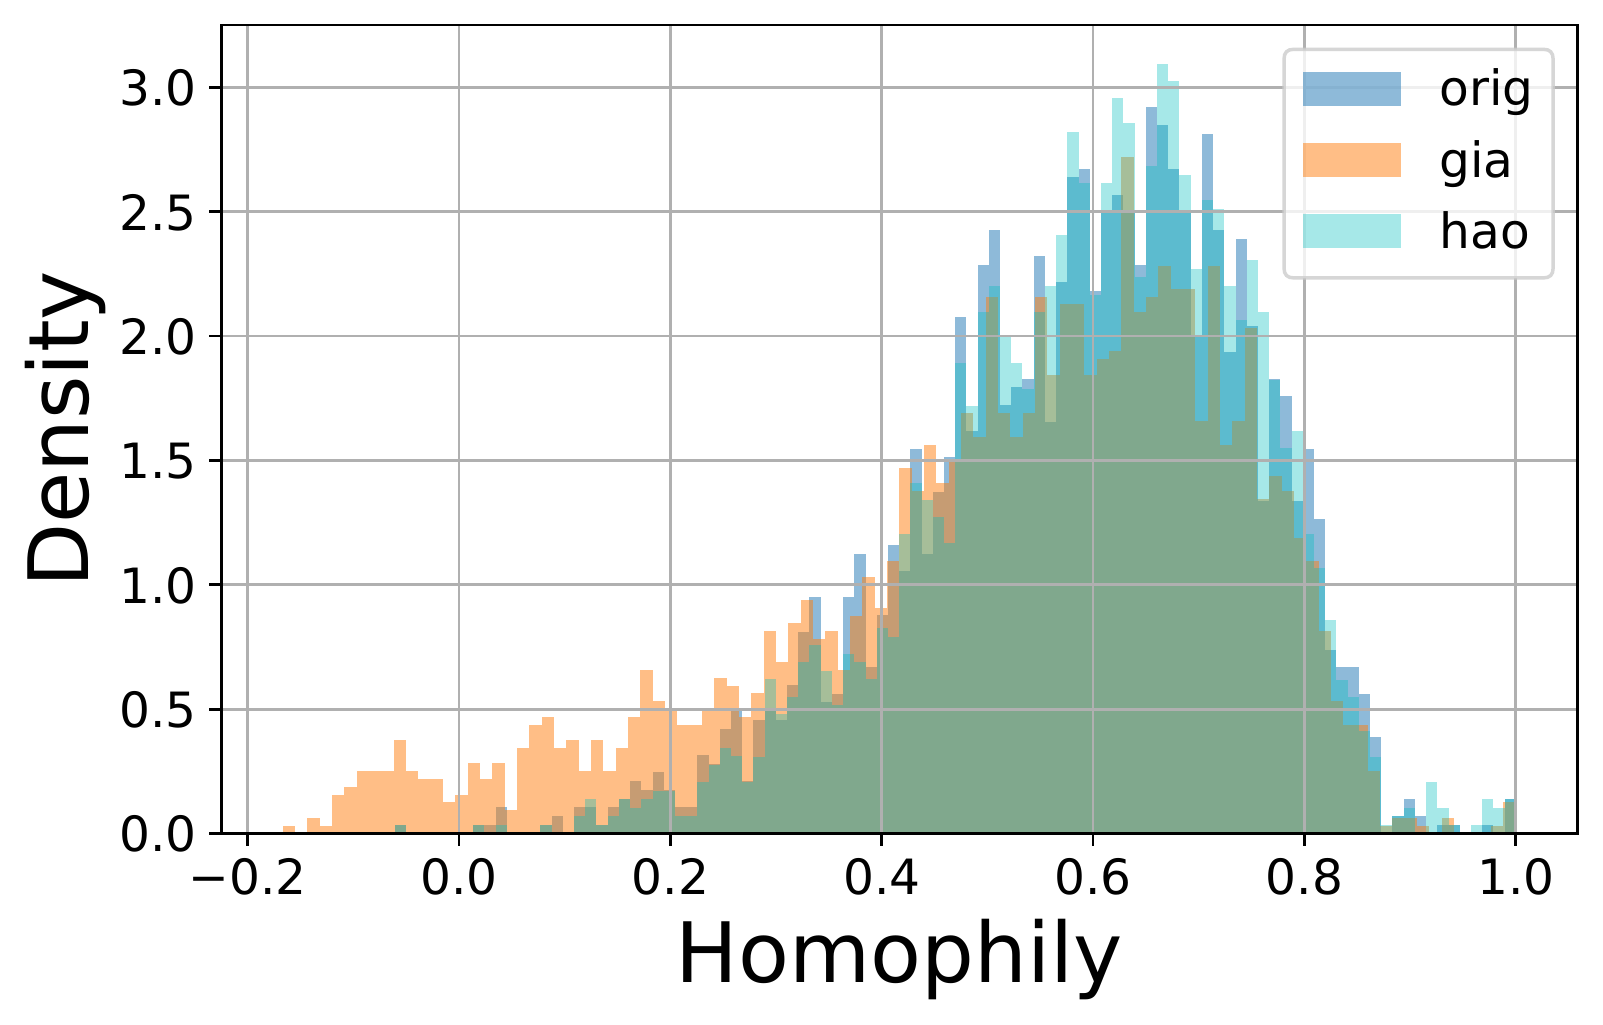}
		\caption{Cora}
	\end{subfigure}
	\begin{subfigure}[b]{0.33\textwidth}
		\centering
		\includegraphics[width=\textwidth]{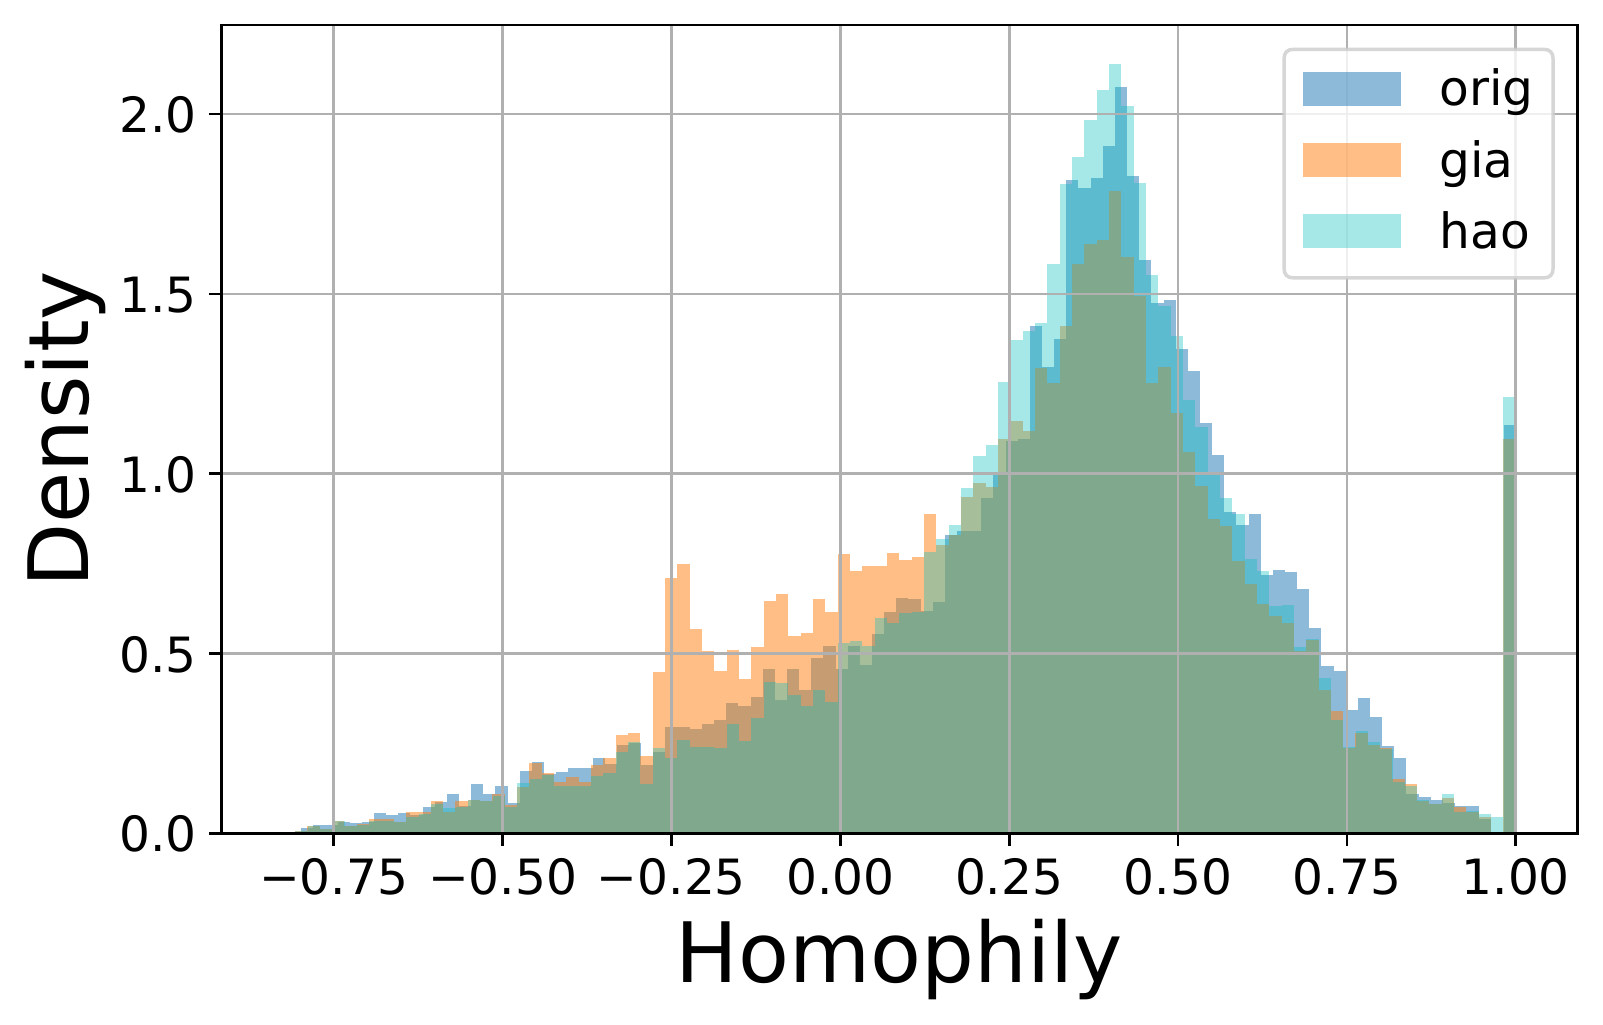}
		\caption{Computers}
	\end{subfigure}
	\begin{subfigure}[b]{0.32\textwidth}
		\centering
		\includegraphics[width=\textwidth]{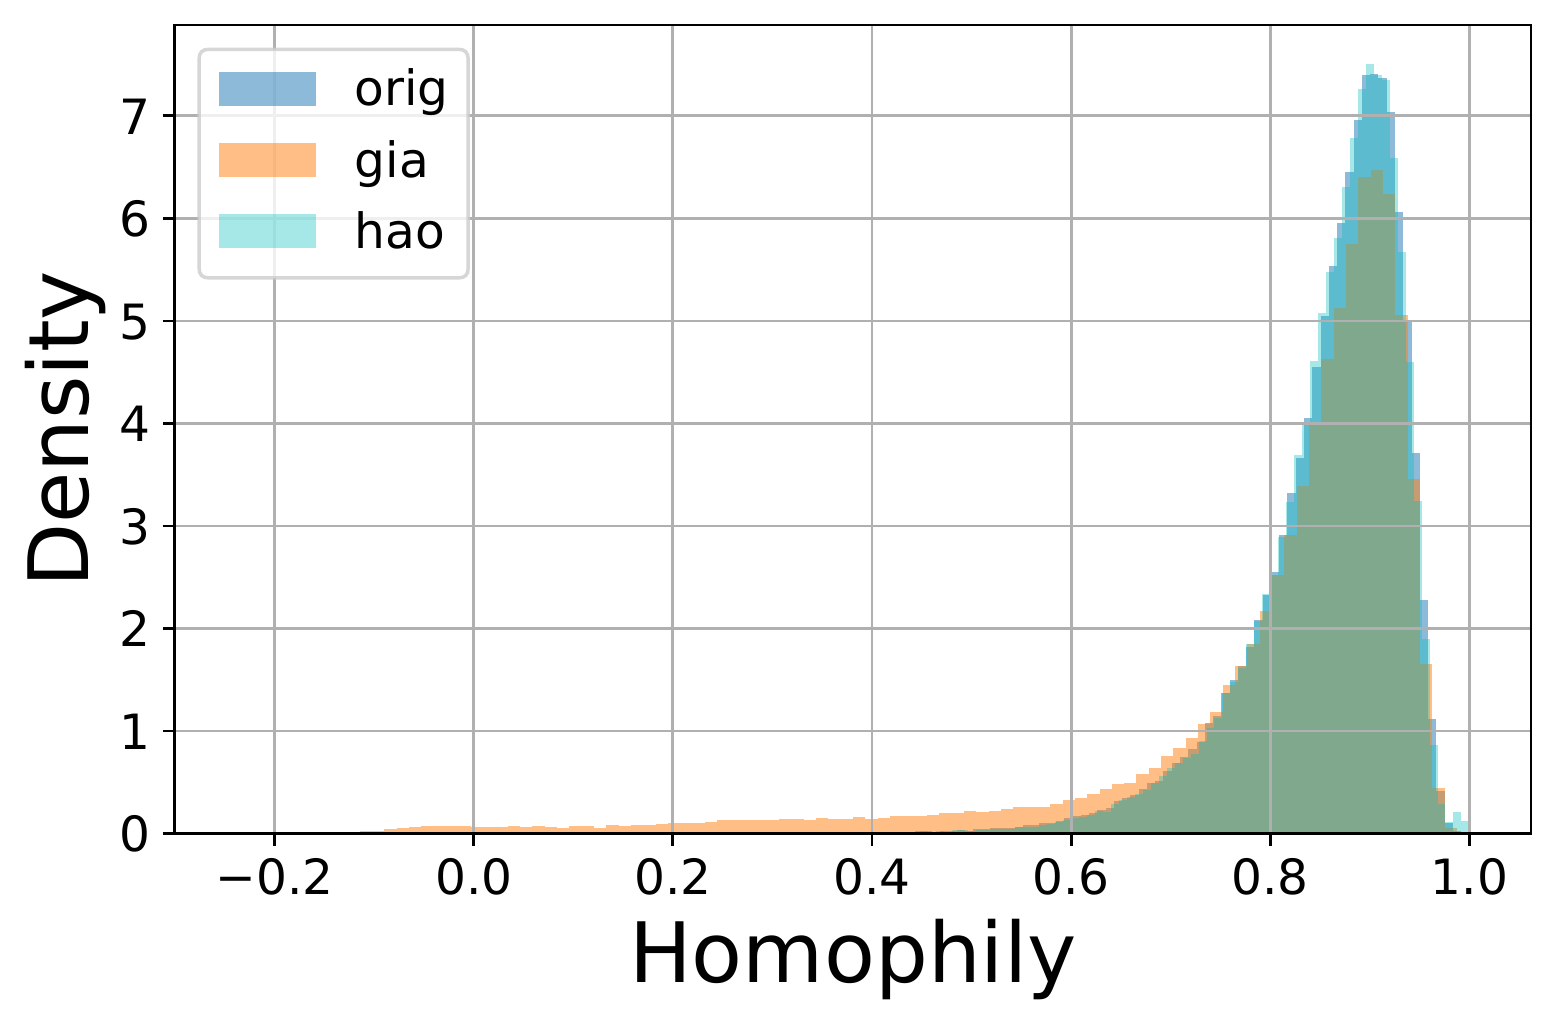}
		\caption{Arxiv}
	\end{subfigure}
	\caption{Homophily distributions after attack}
	\label{fig:gia_homophily_dist_node_atk_appdx_2}
\end{figure}
\subsection{More Homophily Distributions Changes}
\label{sec:homophily_appdx}
We provide more homophily distribution results of the benchmarks we used in the experiments for Cora, Computers and Arxiv, shown as in Fig.~\ref{fig:gia_homophily_dist_node_atk_appdx_1} and Fig.~\ref{fig:gia_homophily_dist_node_atk_appdx_2}, respectively.
GIA is implemented with TDGIA~\citep{tdgia}.
Note that the budgets for TDGIA here is different from that in the previous sections, which utilized the budgets resulting in the maximum harm when compared with GMA.
Similarly, GIA without HAO would severely break the original homophily distribution hence making GIA can be easily defended by homophily defenders.
While incorporated with HAO, GIA would retain the original homophily during attack.

\section{Proofs and Discussions of Theorems}
\label{sec:proof_disscussion_theory}
\subsection{Proof for Theorem~\ref{thm:gia_threat}}
\begin{nono-theorem}
Given moderate perturbation budgets $\triangle_\gia$ for GIA and $\triangle_\gma$ for GMA, that is,
let $\triangle_\gia \leq \triangle_\gma \ll |V|\leq |E|$,
for a fixed linearized GNN $f_\theta$ trained on $\gG$,
assume that $\gG$ has no isolated nodes,
and both GIA and GMA adversaries follow the optimal strategy,
then, \mbox{$\forall \triangle_\gma>0, \exists \triangle_\gia\leq \triangle_\gma$}, such that:
\[
	\mathcal{L}_{\atk}(f_\theta(\gG'_\gia))-\mathcal{L}_{\atk}(f_\theta(\gG'_\gma))\leq 0,
\]
where $\gG'_\gia$ and $\gG'_\gma$ are the perturbed graphs generated by GIA and GMA, respectively.
\end{nono-theorem}
\begin{proof}
	\label{proof:gia_threat}

	The proof sketch is to show that,
	\begin{enumerate}[(a)]
		\item Assume the given GNN model has $k$ layers, there exists a mapping, that when given the same budget, i.e., $\triangle_\gia= \triangle_\gma \ll |V|\leq |E|$, for each perturbation generated by GMA intended to attack node $u$ by perturbing edge $(u,v)$, or node attributes of node $u$ or some node $v$ that connects to $u$ within $k$ hops, we can always map it to a corresponding injection attack, that injects node $x_w$ to attack $u$, and lead to the same effects to the prediction.
		\item When the number of perturbation budget increases, the optimal objective values achieved of GIA is monotonically non-increasing with respect to $\triangle_\gia$, that is
		      \[
			      \mathcal{L}^{k+1}_{\text{atk}}(f_\theta(\gG'_{\text{GIA}}))\leq \mathcal{L}^{k}_{\text{atk}}(f_\theta(\gG'_{\text{GIA}})),
		      \]where $\mathcal{L}^{k}_{\text{atk}}(f_\theta(\gG'_{\text{GIA}}))$ is the optimal value achieved under the perturbation budget of $k$, which is obvious.
	\end{enumerate}
	Once we prove both (a) and (b), the $\mathcal{L}_{\text{atk}}(f_\theta(\gG'_{\text{GIA}}))$ will approach to $\mathcal{L}^{k}_{\text{atk}}(f_\theta(\gG'_{\text{GMA}}))$ from the above as $\triangle_\gia$ approaches to $\triangle_\gma$, hence proving Theorem~\ref{thm:gia_threat}.
	Furthermore, for the flexibility of the constraints on $X_w$, we may adopt the gradient information of $X_w$ with respect to $\mathcal{L}_{\text{atk}}(f_\theta(\gG'_{\text{GIA}}))$ to further optimize $X_w$ and make more damages. Hence, we have $\mathcal{L}_{\text{atk}}(f_\theta(\gG'_{\text{GIA}}))\leq \mathcal{L}^{k}_{\text{atk}}(f_\theta(\gG'_{\text{GMA}}))$.

	To prove (a), the key technique is to show that, under a predefined mapping, there exist a corresponding injection matrix $A_\atk$ along with the features of the injected nodes $X_\atk$,  such that the GIA adversary can cause the same damage as GMA. The definition of the mapping mostly derives how the injection matrix is generated. While for the generation of $X_\atk$, note that all of the input features $X$ is normalized to a specific range within $[-f_l,f_r]$ where $f_l,f_r\geq 0$, following previous works~\citep{grb}. Thus, for any features $X_v \in \mathcal{D}_X$, $\alpha X_v \in \mathcal{D}_X$ when $0 \leq \alpha \leq 1$. We will use the statement multiple times during the derivation of $X_\atk$.

	Next, we will start to prove (a). Following~\citet{advsample_deepinsights}, in GMA, adding new connections between nodes from different classes produces the most benefit to the adversarial objective.
	Hence, given the limited perturbation budget, we give our primary focus to the action of connecting nodes from different classes and
	will prove (a) also holds for the remaining two actions, i.e., edge deletion and node attribute perturbation.

	We prove (a) by induction on the number of linearized layers.
	First of all, we will show prove (a) holds for 1-layer and 2-layer linearized GNN as a motivating example. The model is as $f_\theta=\hat{A}^2X\Theta$ with $H=\hat{A}X\Theta$ and $Z=f_\theta$.

	\textbf{Plural Mapping $\mathcal{M}_2$.} Here we define the mapping $\mathcal{M}_2$ for edge addition. For each edge perturbation pair $(u,v)$ generated by GMA, we can insert a new node $w$ to connect $u$ and $v$.
	The influence of adversaries can be identified as follows, as $\Theta$ is fixed, we may exclude it for simplicity:
	\\
	In layer (1):
	\begin{itemize}
		\item Clean graph:
		      \begin{equation}
			      H_i = \sum_{t \in \mathcal{N}(i)\cup \{i\}}\frac{1}{\sqrt{d_i d_t}}X_t
		      \end{equation}
		\item GMA:
		      \begin{equation}
			      H'_i = \left\{
			      \begin{aligned}
				       & \sum_{t\in \mathcal{N}(i)\cup \{i\}}\frac{1}{\sqrt{d_t (d_i+1)}}X_t + \frac{1}{\sqrt{d_v(d_i+1)}}X_v, & i \in \{u\}      \\
				       & \sum_{t\in \mathcal{N}(i)\cup \{i\}}\frac{1}{\sqrt{d_t (d_i+1)}}X_t + \frac{1}{\sqrt{d_u(d_i+1)}}X_u, & i \in \{v\}      \\
				       & H_i,                                                                                                  & i \notin \{u,v\} \\
			      \end{aligned}
			      \right.
		      \end{equation}
		\item GIA:
		      \begin{equation}H''_i = \left\{
			      \begin{aligned}
				       & \sum_{t \in \mathcal{N}(i)\cup \{i\}}\frac{1}{\sqrt{d_t (d_i+1)}}X_t+\frac{1}{\sqrt{3(d_i+1)}}X_w, & i \in \{u,v\}      \\
				       & H_i,                                                                                               & u \notin \{u,v,w\} \\
				       & \frac{1}{\sqrt{3}}(\frac{1}{\sqrt{d_u+1}}X_u+\frac{1}{\sqrt{d_v+1}}X_v+\frac{1}{\sqrt{3}}X_w),     & i \in \{w\}        \\
			      \end{aligned}
			      \right.
		      \end{equation}
	\end{itemize}
	where $d_i$ refers to the degree of node $i$ with self-loops added for simplicity.
	Thus, in layer (1), to make the influence from GMA and GIA on node $u$ equal, the following constraint has to be satisfied:
	\begin{equation}
		\frac{1}{\sqrt{3(d_u+1)}}X_w = \frac{1}{\sqrt{(d_v+1)(d_u+1)}}X_v, \\
	\end{equation}
	which is trivially held by setting
	\begin{equation}X_w =
		\frac{\sqrt{3}}{\sqrt{d_v+1}}X_v.
	\end{equation}
	Normally, GMA does not consider isolated nodes~\citep{nettack,metattack} hence we have $d_v\geq 2$ and $X_w\in\mathcal{D}_X$.
	Note that we can even change $X_w$ to make more affects to node $u$ with gradient information, then we may generate a more powerful perturbation in this way. \\
	Then, we go deeper to layer 2.
	In layer (2):
	\begin{itemize}
		\item Clean graph:
		      \begin{equation}
			      Z_i = \sum_{t \in \mathcal{N}(i)\cup \{i\}}\frac{1}{\sqrt{d_i d_t}}H_t
		      \end{equation}
		\item GMA:
		      \begin{equation}
			      Z'_i = \left\{
			      \begin{aligned}
				       & \sum_{t\in \mathcal{N}(i)}\frac{H_t}{\sqrt{d_t (d_i+1)}} +\frac{H'_i}{d_i+1}+ \frac{H'_v}{\sqrt{(d_v+1)(d_i+1)}}, & u \in \{u\}                              \\
				       & \sum_{t\in \mathcal{N}(i)}\frac{H_t}{\sqrt{d_t (d_i+1)}} +\frac{H'_i}{d_i+1}+ \frac{H'_u}{\sqrt{(d_u+1)(d_i+1)}}, & u \in \{v\}                              \\
				       & \sum_{t\in \mathcal{N}(i)}\frac{H'_t}{\sqrt{d_t (d_i+1)}},                                                        & u \in \mathcal{N}(u) \cup \mathcal{N}(v) \\
				       & Z_u,                                                                                                              & \text{otherwise}                         \\
			      \end{aligned}
			      \right.
		      \end{equation}
		\item GIA:
		      \begin{equation}Z''_i = \left\{
			      \begin{aligned}
				       & \sum_{t \in \mathcal{N}(i)}\frac{1}{\sqrt{d_t (d_i+1)}}H_t+\frac{1}{d_i+1}H''_i+\frac{1}{\sqrt{3(d_i+1)}}H''_w, & i \in \{u,v\}      \\
				       & H_u,                                                                                                            & i \notin \{u,v,w\} \\
				       & \frac{1}{\sqrt{3}}(\frac{1}{\sqrt{d_u+1}}H''_u+\frac{1}{\sqrt{d_v+1}}H''_v+\frac{1}{\sqrt{3}}H''_w),            & i \in \{w\}        \\
			      \end{aligned}
			      \right.
		      \end{equation}
	\end{itemize}
	Similarly, to make $Z'_u=Z''_u$, we have to satisfy the following constraint:
	\begin{equation}
		\begin{aligned}
			\frac{1}{d_u+1}H''_u+\frac{1}{\sqrt{3(d_u+1)}}H''_w                                                & = \frac{1}{d_u+1}H'_i+ \frac{1}{\sqrt{(d_v+1)(d_u+1)}}H'_v, \\
			\frac{\sqrt{3}}{d_u+1}\sum_{t \in \mathcal{N}(u)\cup \{u\}}\frac{1}{\sqrt{d_t }}X_t+\frac{4}{3}X_w & +
			\frac{1}{\sqrt{3}}(\frac{1}{\sqrt{d_u+1}}X_u+\frac{1}{\sqrt{d_v+1}}X_v)                                                                                          \\
			=                                                                                                                                                                \\
			\frac{\sqrt{3}}{d_u+1}\sum_{t\in \mathcal{N}(u)\cup \{u\}}\frac{X_t}{\sqrt{d_t}}                   & + \frac{\sqrt{3X_v}}{\sqrt{d_v+1}}  +                       \\
			\frac{\sqrt{3}}{\sqrt{d_v+1}}(\sum_{t\in \mathcal{N}(v)\cup \{v\}}\frac{X_t}{\sqrt{d_t (d_v+1)}}   & + \frac{X_u}{\sqrt{(d_u+1)(d_v+1)}}),                       \\
			\frac{4}{3}X_w                                                                                                        +
			\frac{1}{\sqrt{3}}(\frac{1}{\sqrt{d_u+1}}X_u                                                       & +\frac{1}{\sqrt{d_v+1}}X_v)                                 \\
			=                                                                                                                                                                \\
			\frac{\sqrt{3X_v}}{\sqrt{d_v+1}}                                                                                      +
			\frac{\sqrt{3}}{\sqrt{d_v+1}}(\sum_{t\in \mathcal{N}(v)\cup \{v\}}\frac{X_t}{\sqrt{d_t (d_v+1)}}   & + \frac{X_u}{\sqrt{(d_u+1)(d_v+1)}}),                       \\
		\end{aligned}
	\end{equation}
	then we let $X_w=\frac{3}{4}(\text{RHS}-\frac{1}{\sqrt{3}}(\frac{1}{\sqrt{d_u+1}}X_u+\frac{1}{\sqrt{d_v+1}}X_v))$ to get the solution of $X_w$ that makes the same perturbation.
	Similarly, we can infer $X_w \in \mathcal{D}_X$. The following proof also applies to layer 2.

	Next, we will prove that, for a linearized GNN with $k$ layers ($k\geq 1$), i.e., $H^{(k)}=\hat{A}^kX\Theta$, once $\exists X_w$, such that the predictions for node $u$ is the same to that perturbed by GMA, i.e., $H^{(k-1)}_u=E^{(k-1)}_u$, then $\exists X'_w$, such that $H^{(k)}_u=E^{(k)}_u$. Here we use $H$ to denote the prediction of GNN attacked by GMA and $E$ for that of GIA. Note that, once the theorem holds, as we have already proven the existence for such $X_w$, it naturally generalizes to an arbitrary number of layers.

	To be more specific, when $H^{(k-1)}_u=E^{(k-1)}_u$, we need to show that, $\exists X_w$, s.t.,
	\begin{equation}
		\label{eq:klayer_con}
		\begin{aligned}
			H^{(k)}_u & = \sum_{j \in \mathcal{N}(u)}\frac{1}{\sqrt{d_u+1}\sqrt{d_j}}H_{j}^{(k-1)}+\frac{1}{d_u+1}H^{(k-1)}_u+\frac{1}{\sqrt{d_u+1}\sqrt{d_v+1}}H_v^{(k-1)}, \\
			E^{(k)}_u & = \sum_{j \in \mathcal{N}(u)}\frac{1}{\sqrt{d_u+1}\sqrt{d_j}}E_{j}^{(k-1)}+\frac{1}{d_u+1}E^{(k-1)}_u+\frac{1}{\sqrt{d_u+1}\sqrt{3}}E_w^{(k-1)},     \\
			H^{(k)}_u & = E^{(k)}_u.                                                                                                                                         \\
		\end{aligned}
	\end{equation}
	Here we make a simplification to re-write Eq.~\ref{eq:klayer_con} by defining the influence score.
	\begin{definition}[Influence Score]
		The influence score from node $v$ to $u$ after $k$ neighbor aggregations with a fixed GNN following Eq.~\ref{eq:gnn},
		is the weight for $X_v$ contributing to $H^{(k)}_u$:
		\begin{equation}
			\label{eq:influence_score_appd}
			H^{(k)}_{u} = \sum_{j\in \mathcal{N}(u)\cup\{u\}}I^{k}_{uj}\cdot X_j,
		\end{equation}
		which can be calculated recursively through:
		\begin{equation}
			I^{k}_{uw} = \sum_{j\in \mathcal{N}(u)\cup\{u\}}(I_{uj}\cdot I^{(k-1)}_{jw})+I^{(k-1)}_{uw}.
		\end{equation}
	\end{definition}
	As $\Theta$ is fixed here, we can simply regard $I^k_{uv}=\hat{A}^k_{uv}$.
	Compared to the predictions after $k$-th propagation onto the clean graph, in GMA, $H^{(k)}_u$ is additionally influenced by node $v$, while in GIA, $H_u^{(k)}$ is additionally influenced by node $v$ and node $w$. Without loss of generality, we may absorb the influence from neighbors of node $v$ into that of node $v$.
	Hence we can rewrite Eq.~\ref{eq:klayer_con} as the following:
	\begin{equation}
		\begin{aligned}
			\Delta H^{(k)}_u & = I^{k}_{\text{GMA}_{uv}}X_{v},                              \\
			\Delta E^{(k)}_u & = I^{k}_{\text{GIA}_{uv}}X_{v}+I^{k}_{\text{GIA}_{uw}}X_{w}, \\
			\Delta H^{(k)}_u & = \Delta E^{(k)}_u,                                          \\
		\end{aligned}
	\end{equation}
	where
	\[
		I^{k}_{\text{GIA}_{uv}} =
		\sum_{j \in \mathcal{N}(u)\cup\{u\}}I_{\text{GIA}_{uj}}\cdot I^{(k-1)}_{\text{GIA}_{jv}} +
		I_{\text{GIA}_{uw}}\cdot I^{(k-1)}_{\text{GIA}_{wv}}.
	\]
	Then we can further simplify it as,
	\begin{equation}
		\label{eq:xw_sol}
		(I^{k}_{\text{GMA}_{uv}}-I^{k}_{\text{GIA}_{uv}})X_{v}=I^{k}_{\text{GIA}_{uw}}X_{w}.
	\end{equation}
	To show the existence of $X_w$ that solves the above equation, it suffices to show $I^{k}_{\text{GIA}_{uw}}\neq 0$ and $X_w\in \mathcal{D}_X$.
	Note that $\exists X_w$ s.t.,
	\begin{equation}
		(I^{(k-1)}_{\text{GMA}_{uv}}-I^{(k-1)}_{\text{GIA}_{uv}})X_{v}=I^{(k-1)}_{\text{GIA}_{uw}}X_{w}.
	\end{equation}
	Since $\hat{A}^k \geq \mathbf{0}, \forall k \geq 0$, so we have $I^{(k-1)}_{\text{GIA}_{uw}}> 0$. Moreover,
	\[
		I^{k}_{uw} = \sum_{j\in \mathcal{N}(u)\cup\{u\}}(\hat{A}_{uj}\cdot\hat{A}^{(k-1)}_{jw})+I^{(k-1)}_{uw},
	\]
	then it is obvious that the $I^{k}_{uw} > 0$.
	Moreover, with the definition of $I^k_{uv}=\hat{A}^k_{uv}$, it is obvious that
	$I^{(k-1)}_{\text{GIA}_{uw}}\geq I^{(k-1)}_{\text{GMA}_{uv}}$ for $v$ with a degree not less than $1$ (i.e., $v$ is not an isolated node).
	Hence, we have $(I^{(k-1)}_{\text{GMA}_{uv}}-I^{(k-1)}_{\text{GIA}_{uv}})/I^{(k-1)}_{\text{GIA}_{uw}} \leq 1$ and $X_w\in \mathcal{D}_X$.

	Now we have proved (a) holds for edge addition. For the remaining actions of GMA, we can use a new mapping $\mathcal{M}_1$ that injects one node $w$ to node $u$ to prove (a).

	For an edge deletion of $(u,v)$, given $\mathcal{M}_1$, one may rewrite Eq.~\ref{eq:klayer_con} for the left nodes other than $v$, as well as the equation involving $I^{k}_{uw}$, and derive the same conclusions similarly. Intuitively, for edge deletion, considering the classification probability, removing an edge is equivalent to enlarge the predicted classification probability for other classes, hence it fictionalizes likewise the edge addition and we can use a similar proof for this action.

	Besides, $\mathcal{M}_1$ can also apply to the perturbation of features to node $u$ or the other neighbor nodes of $u$ within $k$ hops, where we inject one node $w$ to make the same effect. In this case, we can rewrite Eq.~\ref{eq:klayer_con} and simplify it as following:
	\begin{equation}
		\begin{aligned}
			\Delta H^{(k)}_u & = I^{k}_{\text{GMA}_{uv}}\Delta X_{v}, \\
			\Delta E^{(k)}_u & = I^{k}_{\text{GIA}_{uw}}X_{w},        \\
			\Delta H^{(k)}_u & = \Delta E^{(k)}_u,                    \\
		\end{aligned}
	\end{equation}
	where $v\in \{\mathcal{N}^k(u)\cup u\}$, i.e., node $u$ or its $k$-hop neighbor, and $\Delta X_{v}$ is the perturbation to the attributes of node $v$.
	Similarly, by the definition of $I^k_{uv}$, for node $v$ with a degree not less than $1$ (i.e., $v$ is not an isolated node), we have $I^{k}_{\text{GIA}_{uw}}\geq I^{k}_{\text{GMA}_{uv}}$, hence we have $I^{k}_{\text{GMA}_{uv}}/I^{k}_{\text{GIA}_{uw}}\leq 1$ and $X_{w}\in \mathcal{D}_X$.

	Thus, we complete the whole proof.
\end{proof}

\textbf{Theorem~\ref{thm:gia_threat} for other GNNs}. We can extend Theorem~\ref{thm:gia_threat} to other GNNs such as GCN, GraphSage, etc.
Recall the theorem 1 in~\cite{jknet}:
\begin{lemma}
	\label{thm:random_walk}
	Given a k-layer GNN following the neighbor aggregation scheme via Eq.~\ref{eq:gnn}, assume that all paths in the computation graph of the model are activated with the same probability of success $p$. Then the influence distribution $I_x$ for any node $x\in V$ is equivalent, in expectation, to the $k$-step random walk distribution on $\tilde{\gG}$ starting at node $x$.
\end{lemma}
To apply Lemma~\ref{thm:random_walk}, we observe that the definition of $I^{k}_{uw}$ is analogous to random walk starting from node $u$.
Thus, one may replace the definition of $I^{k}_{uw}$ here to the influence score defined by~\cite{jknet}, conduct a similar proof above with random walk score and obtain the same conclusions,
given the mapping $\mathcal{M}_2$, for each edge addition $(u,v)$, $\exists X_w$, such that
\begin{equation}
	\mathbb{E}(\mathcal{L}^{k}_{\text{atk}}(f_\theta(\gG'_{\text{GIA}}))) = \mathbb{E}(\mathcal{L}^{k}_{\text{atk}}(f_\theta(\gG'_{\text{GIA}}))).
\end{equation}
Though the original theorem only proves Lemma~\ref{thm:random_walk} for GCN and GraphSage, it is obvious one can easily extend the proof in \cite{jknet} for aggregation scheme as Eq.~\ref{eq:gnn}.

\textbf{Cases for Less GIA Budget}. We can reduce GIA budgets in two ways.
\begin{enumerate}[(a)]
	\item For GMA that performs both node feature perturbation and edge addition, considering a edge perturbation $(u,v)$, $\mathcal{M}_2$  essentially also applies for node feature perturbations on $u$ or $v$ without additional budgets.
	\item It is very likely that with the mapping above, GIA will produce many similar nodes. Hence, with one post-processing step to merge similar nodes together and re-optimize them again,
	      GIA tends to require less budgets to make the same or more harm than GMA. That is also reflected in our experiments as shown in Fig.~\ref{fig:motivate_w_defense}.
\end{enumerate}


\subsection{GIA with Plural Mapping for More GMA Operations}
\label{sec:m2_gma_appdx}
Here we explain how our theoretical results also apply to the remaining actions, i.e., edge deletion and node feature perturbation, of GMA with $\mathcal{M}_2$ (Def.~\ref{def:m2_mapping}). In the proof for Theorem~\ref{thm:gia_threat}, we have proved the existence of mappings for edge removal and node feature perturbation.
Once the injected node features are set to have the same influence to the predictions on the targets, they can be further optimized for amplifying the damage, thus all of our theoretical results can be derived similarly like that for edge addition operation.


\subsection{Proof for Theorem~\ref{thm:gia_easy_defend}}
\begin{nono-theorem}
Given conditions in Theorem~\ref{thm:gia_threat},
consider a GIA attack, which \textup{(i)} is mapped by $\mathcal{M}_2$ (Def.~\ref{def:m2_mapping}) from a GMA attack that only performs edge addition perturbations,
and \textup{(ii)} uses a linearized GNN trained with at least one node from each class in $\gG$ as the surrogate model, and \textup{(iii)} optimizes the malicious node features with PGD.
Assume that $\gG$ has no isolated node, and has node features as $X_u=\frac{C}{C-1}e_{Y_u}-\frac{1}{C-1}\mathbf{1}\in \R^d$,
where $Y_u$ is the label of node $u$ and $e_{Y_u}\in\R^d$ is a one-hot vector with the $Y_u$-th entry being $1$ and others being $0$.
Let the minimum similarity for any pair of nodes connected in $\gG$ be $s_{\gG}=\min_{(u,v)\in E}\text{sim}(X_u,X_v)$ with $\text{sim}(X_u,X_v)=\frac{X_u\cdot X_v}{\norm{X_u}_2\norm{X_v}_2}$.
For a homophily defender $g_\theta$ that prunes edges $(u,v)$ if $\text{sim}(X_u,X_v)\leq s_{\gG}$,
we have:
\[
	\mathcal{L}_{\text{atk}}(g_\theta(\mathcal{M}_2(\gG'_{\text{GMA}})))-\mathcal{L}_{\text{atk}}(g_\theta(\gG'_{\text{GMA}}))\geq 0.
\]
\end{nono-theorem}
\begin{proof}
	\label{proof:gia_easy_defend}
	We prove Theorem~\ref{thm:gia_easy_defend} by firstly show the following lemma.
	\begin{lemma}
		\label{thm:gia_lower_sim}
		Given conditions in Theorem~\ref{thm:gia_easy_defend}, as the optimization on $X_w$ with respect to $\mathcal{L}_{\text{atk}}$ by PGD approaches,
		we have:
		\[
			\text{sim}(X_u,X_w)^{(t+1)} \leq \text{sim}(X_u,X_w)^{(t)},
		\]
		where $t$ is the number of optimization steps.
	\end{lemma}
	We prove Lemma~\ref{thm:gia_lower_sim} in the follow-up section, i.e., Appendix~\ref{proof:gia_lower_sim}.
	With Lemma~\ref{thm:gia_lower_sim}, known that GIA is mapped from GMA with $\mathcal{M}_2$, $X_w$ will be optimized to have the same effects as GMA at first and continue being optimized to a more harmful state,
	hence for the unit perturbation case as Fig.~\ref{fig:m2_illustration}, we know:
	\begin{equation}
		\label{eq:gia_edge_less_sim}
		\text{sim}(X_u,X_w)\leq \text{sim}(X_u,X_v),
	\end{equation}
	as the optimization on $X_w$ approaches. Furthermore, it follows:
	\begin{equation}
		h_u^\gia \leq h_u^\gma,
	\end{equation}
	where $h_u^\gia$ and $h_u^\gma$ denote the homophily of node $u$ after GIA and GMA attack, respectively.
	Now if we go back to the homophily defender $g_\theta$, for any threshold specified to prune the edge $(u,v)$, as Lemma~\ref{thm:gia_lower_sim} and Eq.~\ref{eq:gia_edge_less_sim} indicates,
	direct malicious edges in GIA are more likely to be pruned by $g_\theta$. Let $\tau_\gia$ and $\tau_\gma$ denote the corresponding similarity between $(u,w)$ in GIA and $(u,v)$ in GMA,
	we have several possibilities compared with $s_{\gG}=\min_{(u,v)\in E}\text{sim}(X_u,X_v)$:
	\begin{enumerate}[(a)]
		\item $\tau_\gia\leq \tau_\gma \leq s_{\gG}$: all the malicious edges will be pruned, Theorem~\ref{thm:gia_easy_defend} holds;
		\item $\tau_\gia\leq  s_{\gG}\leq \tau_\gma$: all the GIA edges will be pruned, Theorem~\ref{thm:gia_easy_defend} holds;
		\item $ s_{\gG}\leq \tau_\gia\leq \tau_\gma$: this is unlikely to happen, otherwise $\tau_\gia$ can be optimized to even worse case, Theorem~\ref{thm:gia_easy_defend} holds;
	\end{enumerate}
	Thus, we complete our proof.
\end{proof}
Interestingly, we can also set a specific threshold $\tau_h$ for homophily defender s.t., $\tau_h-s_{\gG}\leq \epsilon\geq 0$, where some of the original edges will be pruned, too.
However, some of previous works indicate promoting the smoothness or slightly dropping some edges will bring better performance~\citep{dropedge,p-reg,aug_gnn,self-enhance}.
The similar discussion can also be applied to this case and obtain the same conclusions.

\subsection{Proof for Lemma~\ref{thm:gia_lower_sim}}
\label{proof:gia_lower_sim}
\begin{proof}
	To begin with, without loss of generality, we may assume the number of classes is $2$ and $Y_u=0$, which can be similarly extended to the case of multi-class.
	With the feature assignment in the premise, let the label of node $u$ is $Y_u$, we have:
	\begin{equation}
		\label{eq:xw_indicator}
		X_u = \left\{
		\begin{aligned}
			 & [1, -1]^T, & Y_u =0, \\
			 & [-1, 1]^T, & Y_u =1. \\
		\end{aligned}
		\right.
	\end{equation}
	After setting it to having the same influence as that in GMA following Eq.~\ref{eq:xw_sol}, we have:
	\begin{equation}
		X_{w}=\frac{(I^{k}_{\text{GMA}_{uv}}-I^{k}_{\text{GIA}_{uv}})}{I^{k}_{\text{GIA}_{uw}}}X_{v}.
	\end{equation}
	Then, let $\mathcal{L}_u$ denote the training loss $\mathcal{L}_{\text{train}}$ on node $u$, we can calculate the gradient of $X_w$:
	\begin{equation}
		\frac{\partial \mathcal{L}_u}{\partial X_u}=\frac{\partial \mathcal{L}_u}{\partial H^{(k)}_u}\cdot \frac{\partial H^{(k)}_u}{\partial X_w}=\frac{\partial \mathcal{L}_u}{\partial H^{(k)}_u}\cdot I^{k}_{\text{GIA}_{uw}}\cdot \Theta.
	\end{equation}
	With Cross-Entropy loss, we further have:
	\begin{equation}
		\frac{\partial \mathcal{L}_u}{\partial H^{(k)}_u}=[-1, 1]^T.
	\end{equation}
	Then, we can induce the update step of optimizing $X_w$ with respect to $\mathcal{L_\atk}=-\mathcal{L}_{\text{train}}$ by PGD:
	\begin{equation}
		X^{(t+1)}_w = X^{(t)}_w+\epsilon \sign(I^{k}_{\text{GIA}_{uw}}\cdot [-1, 1]^T\cdot \Theta),
	\end{equation}
	where $t$ is the number of update steps.
	As the model is trained on at least nodes with indicator features following Eq.~\ref{eq:xw_indicator} from each class,
	without loss of generality, here we may assume $\Theta \geq \mathbf{0}$,
	the optimal $\Theta$ would converge to $\Theta \geq \mathbf{0}$. Thus,
	\[
		\sign(I^{k}_{\text{GIA}_{uw}}\cdot [-1, 1]^T\cdot \Theta) = \sign(I^{k}_{\text{GIA}_{uw}}\cdot [-1, 1]^T).
	\]
	Let us look into the change of cosine similarity between node $u$ and node $v$ as:
	\begin{equation}
		\Delta \text{sim}(X_u,X_w) = \alpha (X_u\cdot X^{(t+1)}_w-X_u\cdot X^{(t)}_w),
	\end{equation}
	where $\alpha\geq 0$ is the normalized factor. To determine the sign of $\Delta \text{sim}(X_u,X_w)$, we may compare $X_u\cdot X^{(t+1)}$ with $X_u\cdot X^{(t)}_w$.
	Here we expand $X_u\cdot X^{(t+1)}_w$. Let $X_{u0}, X_{u1}$ to denote the first and second element in $X_u$ respectively, we have:
	\begin{equation}
		\label{eq:x_t_cos}
		\begin{aligned}
			X_u\cdot X^{(t+1)}_w & =\frac{X_u\cdot X_w+\epsilon \sign(I^{k}_{\text{GIA}_{uw}}\cdot [-1, 1]^T)X_u}{\norm{X_u}_2\cdot\norm{X^{(t+1)}_w}_2},   \\
			                     & =\frac{X_u\cdot X_w+\epsilon (X_{u1}-X_{u0})}{\norm{X_u}_2\sqrt{X^2_{w0}+X^2_{w1}+\epsilon^2+2\epsilon(X_{w1}-X_{w0})}}, \\
		\end{aligned}
	\end{equation}
	where we omit the sign of $I^{k}_{\text{GIA}_{uw}}$ for $I^{k}_{\text{GIA}_{uw}}\geq 0$ according to the definition. Recall that we let $Y_u=0$, hence we have $(X_{u1}-X_{u0})\leq 0$.
	Besides, following Eq.~\ref{eq:xw_sol}, we have $\sign(X_{w1}-X_{w0})=\sign(X_{v1}-X_{v0})$. As GMA tend to connect nodes from different classes, we further have $\sign(X_{w1}-X_{w0})\geq 0$.
	Comparing to $X_u\cdot X^{(t)}_w$, we know in Eq.~\ref{eq:x_t_cos}, the numerator decreases and the denominator increases, as $\epsilon\geq0$, so the overall scale decreases. In other words, we have:
	\begin{equation}
		\Delta \text{sim}(X_u,X_w) = \alpha (X_u\cdot X^{(t+1)}_w-X_u\cdot X^{(t)}_w)\leq 0,
	\end{equation}
	which means that the cosine similarity between node $u$ and node $v$ decreases as the optimization of $X_w$ with respect to $\mathcal{L}_\atk$ processes. Thus, we complete our proof for Lemma~\ref{thm:gia_lower_sim}.
\end{proof}

\subsection{Proof for Theorem~\ref{thm:hao_break_limit}}
\begin{nono-theorem}
Given conditions as Theorem~\ref{thm:gia_easy_defend},
when $\lambda>0$, we have
$m(\mathcal{H}_\gG,\mathcal{H}_{\gG'_{\text{HAO}}})\leq m(\mathcal{H}_\gG,\mathcal{H}_{\gG'_{\text{GIA}}})$,
hence:
\[
	\mathcal{L}_{\text{atk}}(g_\theta(\gG'_{\text{HAO}}))-\mathcal{L}_{\text{atk}}(g_\theta(\gG'_{\text{GIA}}))\leq 0,
\]
where $\gG'_{\text{HAO}}$ is generated by GIA with HAO, and $\gG'_{\text{GIA}}$ is generated by GIA without HAO.
\end{nono-theorem}
\begin{proof}
	\label{proof:hao_break_limit}
	Similar with the proof for Theorem~\ref{thm:gia_easy_defend}, we begin with binary classification, without loss of generality.
	With the feature assignment in the premise, let the label of node $u$ is $Y_u$, we have:
	\begin{equation}
		X_u = \left\{
		\begin{aligned}
			 & [1, -1]^T, & Y_u =0, \\
			 & [-1, 1]^T, & Y_u =1. \\
		\end{aligned}
		\right.
	\end{equation}
	Let $\mathcal{L}_u$ denote the training loss $\mathcal{L}_{\text{train}}$ on node $u$, we look into the gradient of $X_w$ with respect to $\mathcal{L}_u$:
	\begin{equation}
		\frac{\partial \mathcal{L}_u}{\partial X_u}=\frac{\partial \mathcal{L}_u}{\partial H^{(k)}_u}\cdot \frac{\partial H^{(k)}_u}{\partial X_w}=\frac{\partial \mathcal{L}_u}{\partial H^{(k)}_u}\cdot I^{k}_{\text{GIA}_{uw}}\cdot \Theta.
	\end{equation}
	With Cross-Entropy loss, we further have:
	\begin{equation}
		\frac{\partial \mathcal{L}_u}{\partial H^{(k)}_u}=[-1, 1]^T.
	\end{equation}
	Together with HAO, we can infer the update step of optimizing $X_w$ with respect to \mbox{$\mathcal{L_\atk}=-\mathcal{L}_{\text{train}}+\lambda C(\gG,\gG')$} by PGD:
	\begin{equation}
		X^{(t+1)}_w = X^{(t)}_w+\epsilon \sign((I^{k}_{\text{GIA}_{uw}}\cdot [-1, 1]^T+\lambda[1,-1]^T)\cdot \Theta),
	\end{equation}
	where $t$ is the number of update steps. Similarly, without loss of generality, we may assume $\Theta\geq \mathbf{0}$.
	As the optimization approaches, given $\lambda>0$, GIA with HAO will early stop to some stage that $(I^{k}_{\text{GIA}_{uw}}\cdot [-1, 1]^T+\lambda[1,-1]^T)=\mathbf{0}$,
	hence similar to the proof of Theorem~\ref{thm:gia_easy_defend}, it follows:
	\begin{equation}
		h_u^\gia \leq h_u^\text{HAO},
	\end{equation}
	where $h_u^\gia$ and $h_u^\text{HAO}$ denote the homophily of node $u$ after GIA and GIA with HAO attack, respectively.
	Likewise, we can infer that:
	\[
		\mathcal{L}_{\text{atk}}(g_\theta(\gG'_{\text{HAO}}))-\mathcal{L}_{\text{atk}}(g_\theta(\gG'_{\text{GIA}}))\leq 0.
	\]
	Thus, we complete our proof.
\end{proof}

\subsection{Certified Robustness of Homophily Defender}
Here we prove the certified robustness of homophily for a concrete GIA case. We prove via the decision margin as follows:
\label{sec:gia_cer_robo}
\begin{definition}[Decision Margin]
	\label{def:decision_margin}
	Given a $k$-layer GNN,
	let $H^{(k)}_{[u,c]}$ denote the corresponding entry in $H^{(k)}_{u}$ for the class $c$,
	the decision margin on node u with class label $Y_u$ can be denoted by:
	\[
		m_u = 	H^{(k)}_{[u,y_u]}-\max_{c\in \{0,..,C-1\}}H^{(k)}_{[u,c]}.
	\]
\end{definition}
A Multi-Layer Perceptron (MLP) can be taken as a $0$-layer GNN which the definition also applies.
Then, we specify the certified robustness as follows:
\begin{proposition}[Certified Robustness of Homophily Defender]
	\label{thm:gia_cer_robo}
	Consider a direct GIA attack uses a linearized GNN trained with at least one node from each class in $\gG$,
	that targets at node $u$ by injecting a node $w$ connecting to $u$,
	let node features $x_u=\frac{C}{C-1}\text{onehot}(Y_u)-\frac{1}{C-1}\mathbf{1}$,
	the homophily of $u$ be $\tau$, the decision margin of a MLP on $u$ be $\gamma$,
	the minimum similarity for any pair of nodes connected in the original graph be $s_{\gG}=\min_{(u,v)\in E}\text{sim}(X_u,X_v)$,
	homophily defender $g_\theta$ can defend such attacks, if $-\alpha\frac{1}{\sqrt{1+1/d_u}}(\tau+\beta \gamma)\leq s_{\gG}$,
	and $g_\theta$ prunes edges $(u,v)$ s.t.,
	\[
		\text{sim}(X_u,X_w)\leq -\alpha\sqrt{\frac{1}{1+1/d_u}}(\tau+\beta\gamma),
	\]
	where $\alpha,\beta\geq 0$ are corresponding normalization factors.
\end{proposition}
Intuitively, effective attacks on a node with higher degrees, homophily or decision margin require a lower similarity between node $w$ and $u$ hence more destruction to the homophily of node $u$.
GIA without any constraints tends to optimize $\text{sim}(X_u,X_w)$ to a even lower value.
Thus, it becomes easier to find a suitable condition for $g_\theta$, with which it can painlessly prune all vicious edges while keeping all original edges.
\begin{proof}
	\label{proof:gia_cer_robo}
	Analogous to the proof for Lemma~\ref{thm:gia_lower_sim}, without loss of generality, we begin with
	binary classification, normalized indicator features and $Y_u=0$ as follows:
	\begin{equation}
		X_u = \left\{
		\begin{aligned}
			 & [1, -1]^T, & Y_u =0, \\
			 & [-1, 1]^T, & Y_u =1. \\
		\end{aligned}
		\right.
	\end{equation}
	The decision margin based on $k$-th layer representation can be denoted by
	\begin{equation}
		m=H^{(k)}_{[u,y_u]}-\max_{c\in \{0,..,C-1\}}H^{(k)}_{[u,c]},
	\end{equation}
	follows the Definition~\ref{def:decision_margin}. In our binary classification case, we have
	\begin{equation}
		\gamma=H^{(0)}_{[u,0]}-H^{(0)}_{[u,1]},
	\end{equation}
	where $H^{(0)}$ is the output of a $0$-layer GNN, or MLP (Multi-Layer Perceptron). A $k$-layer GNN can be regarded as
	generating new hidden representation for node $u$ by aggregating its neighbors, hence, we may induce the decision margin
	for a $k$-layer GNN at node $u$ as
	\begin{equation}
		m=H^{(k)}_{[u,0]}-H^{(k)}_{[u,1]}=([\sum_{j\in \mathcal{N}(u)}I_{uj}X_j]_{[0]}-[\sum_{j\in \mathcal{N}(u)}I_{uj}X_j]_{[1]})+I_{uu}^{(k)}\gamma,
	\end{equation}
	where we can replace the influence from neighbors with homophily of node $u$. Observe that $h_u$ essentially indicates how much neighbors of node $u$ contribute to $H_{[u,0]}^{(k)}$, for example, in binary case, let $\zeta> 0$ be the corresponding normalization factor,
	\[
		h_u = \frac{1}{\zeta}([\sum_{j\in \mathcal{N}(u)}I_{uj}X_j]_{[0]}[X_u]_{[0]}+[\sum_{j\in \mathcal{N}(u)}I_{uj}X_j]_{[1]}[X_u]_{[1]}),
	\]
	which means,
	\[
		[\sum_{j\in \mathcal{N}(u)}I_{uj}X_j]_{[1]} = \frac{1}{[X_u]_{[1]}} (\zeta h_u-[\sum_{j\in \mathcal{N}(u)}I_{uj}X_j]_{[0]}[X_u]_{[0]}),
	\]
	replaced with $X_u=[1,-1]^T$,
	\begin{equation}
		\begin{aligned}
			m & =H^{(k)}_{[u,0]}-H^{(k)}_{[u,1]}                                                                                                                           \\
			  & =([\sum_{j\in \mathcal{N}(u)}I_{uj}X_j]_{[0]}-[\sum_{j\in \mathcal{N}(u)}I_{uj}X_j]_{[1]})+                                                                \\
			  & =([\sum_{j\in \mathcal{N}(u)}I_{uj}X_j]_{[0]}-\frac{1}{[X_u]_{[1]}} (\zeta h_u-[\sum_{j\in \mathcal{N}(u)}I_{uj}X_j]_{[0]}[X_u]_{[0]}))+I_{uu}^{(k)}\gamma \\
			  & =\zeta h_u+I_{uu}^{(k)}\gamma.                                                                                                                             \\
		\end{aligned}
	\end{equation}
	Hence, we have:
	\[
		m=H^{(k)}_{[u,0]}-H^{(k)}_{[u,1]}=\zeta h_u+I_{uu}^{(k)}\gamma,
	\]
	where $\zeta\geq 0$ is the factor of $h_u$.
	With node $w$ injected, the margin can be rewritten as:
	\begin{equation}
		m'=\sqrt{\frac{d_u}{d_u+1}}m+I^{(k)}_{uw}(X_{[w,0]}-X_{[w,1]}).
	\end{equation}
	To perturb the prediction of node $u$, we make $m\leq 0$, hence, we have
	\begin{equation}
		\label{eq:homo_req}
		\begin{aligned}
			m'                                & =\sqrt{\frac{d_u}{d_u+1}}m+I^{(k)}_{uw}(X_{[w,0]}-X_{[w,1]})\leq 0,                \\
			I^{(k)}_{uw}(X_{[w,1]}-X_{[w,0]}) & \geq \sqrt{\frac{d_u}{d_u+1}}m,                                                    \\
			(X_{[w,1]}-X_{[w,0]})             & \geq \frac{1}{I^{(k)}_{uw}}\sqrt{\frac{d_u}{d_u+1}}(\zeta h_u+I_{uu}^{(k)}\gamma). \\
		\end{aligned}
	\end{equation}
	Observe that $\text{sim}(X_u,X_w)=(X_{[w,0]}-X_{[w,1]})$ and $h_u=\tau$, hence, we can write Eq.~\ref{eq:homo_req} in a clean form as
	\begin{equation}
		\text{sim}(X_u,X_w)\leq -\alpha\sqrt{\frac{d_u}{d_u+1}}(\tau+\beta\gamma),
	\end{equation}
	where $\alpha,\beta$ are corresponding normalization factors whose signs are determined by signs of $I^k_{uw}$ and $I^k_{uu}$ respectively.
	In other words, GIA has to optimize $X_w$ satisfying the above requirement to make the attack \textit{effective},
	however, given the premise that all $s_\gG=\min_{(u,v)\in E}\text{sim}(X_u,X_v)\geq -\alpha\sqrt{\frac{d_u}{d_u+1}}(\tau+\beta\gamma)$,
	a defense model $g_\theta$ will directly prune all of the vicious edges satisfying the above requirement and make the attack \textit{ineffective},
	which is exactly what we want to prove.
\end{proof}

\section{More Implementations of Homophily Defender}
\label{sec:more_homo_defender_appdx}
There are many ways to design homophily defenders, inheriting the spirit of recovering the original homophily.
In addition to edge pruning, one could leverage variational inference to learn the homophily distribution or the similarity distribution among neighbors.
Then we use adversarial training to train the model to denoise.
Similarly, learning to promote the smoothness of the graph can also be leveraged to build homophily defenders~\citep{aug_gnn,p-reg,self-enhance}.
Besides, outlier detection can also be adopted to remove or reduce the aggregation weights of malicious edges or nodes.
In the following two subsections, we will present two variants that perform better than GNNGuard~\citep{gnnguard}.

\subsection{Details of Efficient GNNGuard}
\label{sec:egnnguard_appdx}
The originally released GNNGuard requires $O(n^2)$ computation for node-node similarity, making it prohibitive to run on large graphs.
To this end, we implement an efficient alternative of GNNGuard adopting a similar message passing scheme, let $\tau$ be the threshold to prune an edge:
\begin{equation}
	\label{eq:egnngaurd}
	H^{(k)}_u = \sigma(W_k \cdot \sum_{j \in \mathcal{N}(u)\cup\{u\}} \alpha_{uj} H^{(k-1)}_j),
\end{equation}
where
\[
	\alpha_{uj}=\text{softmax}(\frac{z_{uj}}{\sum_{v\in \mathcal{N}(u)\cup \{u\}}z_{uv}}),
\]
and
\[
	z_{uj}  = \left\{
	\begin{aligned}
		 & \frac{\mathbf{1}\{\text{sim}(H^{(k-1)}_j, H^{(k-1)}_u)> \tau\}\cdot\text{sim}(H^{(k-1)}_j\cdot H^{(k-1)}_u)}{\sum_{v \in \mathcal{N}(u)}\mathbf{1}\{\text{sim}(H^{(k-1)}_v, H^{(k-1)}_u)> \tau\}\cdot\text{sim}(H^{(k-1)}_v, H^{(k-1)}_u)}, & u\neq j, \\
		 & \frac{1}{\sum_{v \in \mathcal{N}(u)}\mathbf{1}\{\text{sim}(H^{(k-1)}_v\cdot H^{(k-1)}_u)> \tau\}+1}                                                                                                                                         & u=j.     \\
	\end{aligned}
	\right.
\]
Essentially, it only requires $O(E)$ complexity. We will present the performance of Efficient GNNGuard (EGNNGuard) in table~\ref{tab:homo_defender_performance}.

\subsection{Details of Robust Graph Attention Network (RGAT)}
\label{sec:rgat_appdx}
We introduce another implementation of Robust Graph Attention Network (RGAT).
We adopt the same spirit of GCNGuard \citep{gnnguard}, that eliminates unlike neighbors during message passing based on neighbor similarity. Specifically, we change the standard GAT \citep{gat} attention mechanism as
\[
	\alpha_{i,j} = \frac{\mathbb{1}\{\text{sim}(x_i, x_j)\geq\tau\}}{\sum_{k\in \mathcal{N}(i)\cup \{i\}}\mathbb{1}\{\text{sim}(x_i, x_k)\geq\tau\}},
\]
Additionally, we also adopt the idea of RobustGCN \citep{robustgcn} that stabilize the hidden representations between layers, so we add Layer Normalization \citep{layer_norm} among layers of RGAT. Empirical experiments show that RGAT is a more robust model with or without GIA attacks. For more details, we refer readers to Table~\ref{tab:homo_defender_performance}.

\subsection{Performance of Homophily Defenders}
\bgroup
\def\arraystretch{1.1}
\begin{table}[!h]
	\centering\small
	\caption{Performance of homophily defenders used in experiments}
	\label{tab:homo_defender_performance}
	\begin{tabular}{lccc}
		\toprule
		\multicolumn{1}{l}{\textbf{Model}} & \textbf{Natural Accuracy} & \textbf{Test Robustness} & \textbf{Running Time}         \\\midrule
		GNNGuard                           & $83.58$                   & $64.96$                  & $1.76\times 10^{-3}$
		\\\hline
		EGNNGuard                          & $84.45$                   & $64.27$                  & $\mathbf{5.39\times 10^{-5}}$
		\\\hline
		RGAT                               & $\mathbf{85.75}$          & $\mathbf{66.57}$         & $6.03\times 10^{-5}$          \\\hline
		GCN                                & $84.99$                   & $36.62$                  & $5.87\times 10^{-5}$
		\\\bottomrule
	\end{tabular}
\end{table}
\egroup

We test the performance of different homophily defenders on Cora. Natural Accuracy refers to the test accuracy on clean graph. Test Robustness refers to their averaged performance against all the attacks.
Running time refers to their averaged running time for one training epoch. We repeat the evaluation $10$ times to obtain the average accuracy.
We can see that EGNNGuard has competitive performance with GNNGuard while $20\times$ faster. RGAT performs slightly better and $10\times$ faster.
Hence, for large graphs and adversarial training of GNNGuard, we will use EGNNGuard instead.

\section{More Details about Algorithms used}
\label{sec:gia_alg_desc}
Here we provide detailed descriptions of algorithms mentioned in Section.~\ref{sec:gia_algorithm}.

\subsection{Details of MetaGIA and AGIA}
\label{sec:gia_gradient_appdx}

\subsubsection{Induction of Meta Gradients for MetaGIA}
\label{sec:gia_meta_appdx}
With the bi-level optimization formulation of GIA, similar to meta-attack, we can infer the meta-gradients as follows:
\begin{equation}
	\nabla^{meta}_{A_{\atk}} = \nabla_{A_{\atk}}\mathcal{L}_{\atk}(f_{\theta^*}(A_{\atk},X^*_{\atk})),\quad
	X^*_{\atk} = \text{opt}_{X_{\atk}}\mathcal{L}_{\atk}(f_{\theta^*}(A_{\atk},X_{\atk})).
\end{equation}
Consider the $\text{opt}$ process, we have
\begin{equation}
	\label{x_opt}
	X_{\atk}^{(t+1)} = X_{\atk}^{(t)}-\alpha \nabla_{X_{\atk}^{(t)}}\mathcal{L}_{\atk}(f_{\theta^*}(A_{\atk},X^{(t)}_{\atk})).
\end{equation}
With that, we can derive the meta-gradient for $A_{\atk}$:
\begin{equation}
	\begin{aligned}
		\nabla^{\text{meta}}_{A_{\atk}} & = \nabla_{A_{\atk}}\mathcal{L}_{\atk}(f_{\theta^*}(A_{\atk},X^*_{\atk}))     \\
		                                & = \nabla_{X_{\atk}}\mathcal{L}_{\atk}(f_{\theta^*}(A_{\atk},X^{(t)}_{\atk}))
		\cdot[\nabla_{A_{\atk}}f_{\theta^*}(A_{\atk},X^{(t)}_{\atk})+
		\nabla_{X^{(t)}_{\atk}}f_{\theta^*}(A_{\atk},X^{(t)}_{\atk})\cdot
		\nabla_{A_{\atk}}X^{(t)}_{\atk}],                                                                              \\
	\end{aligned}
\end{equation}
where
\begin{equation}
	\nabla_{A_{\atk}}X^{(t+1)}_{\atk} = \nabla_{A_{\atk}}X^{(t)}_{\atk}
	-\alpha \nabla_{A_{\atk}} \nabla_{X^{(t)}_{\atk}}\mathcal{L}_{\atk}(f_{\theta^*}(A_{\atk},X^{(t)}_{\atk})).
\end{equation}

Note that $X^{(t)}_{\atk}$ depends on $A_{\atk}$ according to Eq.~\ref{x_opt}, so the derivative w.r.t. $A_{\atk}$ need to be traced back. Finally, the update schema for $A_{\atk}$ is as follows:
\begin{equation}
	A^{(t+1)}_{\atk} = A^{(t)}_{\atk} - \beta \nabla^{\text{meta}}_{A^{(t)}_{\atk}}.
\end{equation}
Directly computing the meta gradients is expensive, following Metattack, we adopt approximations like MAML~\citep{maml} for efficiency consideration.
We refer readers to the paper of Metattack for the detailed algorithms by replacing the corresponding variables with those above.

\subsection{Details of AGIA}
For optimizing weights of edge entries in $A_\atk$, we can use either Adam~\citep{adam}, PGD~\citep{pgd} or other optimization methods leveraging gradients.
For simplicity, we use PGD to illustrate the algorithm description of AGIA as follows:

\begin{algorithm}[!h]
	\caption{AGIA: Adaptive Graph Injection Attack with Gradient}
	\label{alg:gia_apgd}
	\SetKwInput{KwInput}{Input}
	\SetKwInput{KwOutput}{Output}
	\SetKwFunction{FInjection}{Injection}
	\SetKwFunction{FUpd}{FeatureUpdate}
	\SetKwComment{Comment}{/* }{ */}

	\KwInput{A graph $\gG=(A,X)$, a trained GNN model $f_{\theta^*}$, number of injected nodes $c$, degree budget $b$, outer attack epochs $e_{\text{outer}}$, inner attack epochs for node features and adjacency matrix $e^X_{\text{inner}},e^A_{\text{inner}}$, learning rate $\eta$, weight for sparsity penalty $\beta$, weight for homophily penalty $\lambda$ \;}
	\KwOutput{Perturbed graph $\gG'=(A', X')$\;}

	Random initialize injection parameters ($A_\atk, X_\atk$)\;
	$\mY_{\text{orig}} \leftarrow f_{\theta^*}(A,X)$ \Comment*[r]{Obtain original predictions on clean graph}
	\For{epoch $\leftarrow$ $0$ to $e_{\text{outer}}$}
	{
	Random initialize $X_\atk$\;
	\For{epoch $\leftarrow$ $0$ to $e^X_{\text{inner}}$}
	{
	$A'\leftarrow A\concat A_\atk, X'\leftarrow X\concat X_\atk$ \;
	$X_\atk \leftarrow \text{Clip}_{(x_{\min},x_{\max})}(X_\atk - \eta \cdot \nabla_{X_\atk}(\mathcal{L}^h_{\text{atk}}))$ \;
	}


	\For{epoch $\leftarrow$ $0$ to $e^A_{\text{inner}}$}
	{
	$A'\leftarrow A \concat A_\atk, X'\leftarrow X\concat X_\atk$ \;
	$A_\atk \leftarrow \text{Clip}_{(0,1)}(A_\atk - \eta \cdot \nabla_{A_\atk}(\mathcal{L}^A_{\text{atk}}))$ \;
	}
	$A_\atk \leftarrow \bigparallel_{i=1}^{k}\argmax_{\text{top}\ b}(A_{\atk[i, :]})$ \;
	}
\end{algorithm}
Here, $\mathcal{L}^h_{\text{atk}}$ refers to the objective of GIA with HAO for the optimization of $X_\atk$.
For the optimization of $A_\atk$, we empirically find the $\lambda_A$ would degenerate the performance, which we hypothesize that is because of the noises as $A_\atk$ is a discrete variable.
Hence, we set $\lambda_A=0$ in our experiments. Additionally, we introduce a sparsity regularization term for the optimization of $A_\atk$:
\begin{equation}
	\mathcal{L}^{A}_\atk = \mathcal{L}_\atk+\beta\frac{1}{|V_\atk|} \sum_{u\in V_\atk}|b-\lVert A_{\atk_{u,:}} \rVert_1|.
\end{equation}
Besides, we empirically observe that Adam performs better than PGD. Hence, we would use Adam for AGIA in our experiments, and leave other methods for future work.
Adopting Adam additionally brings the benefits to utilize momentum and history information to accelerate the optimization escape from the local optimum, which PGD fails to achieve.

\subsection{Details of SeqGIA}
\label{sec:gia_apgd_seq_appdx}
Since gradient methods require huge computation overhead,
we propose a novel divide-and-conquer strategy to iteratively select some of the most vulnerable targets with Eq.~\ref{eq:tdgia+_score} to attack.
Note that it is different from traditional sequential injection methods which still connect the targets in full batch.
For simplicity, we also illustrate the algorithm with PGD, and one may switch to other optimizer such as Adam to optimize $A_\atk$.
The detailed algorithm is as follows:

\begin{algorithm}[H]
	\caption{SeqGIA: Sequential Adaptive Graph Injection Attack}
	\label{alg:gia_apgd_seq}
	\SetKwInput{KwInput}{Input}
	\SetKwInput{KwOutput}{Output}
	\SetKwFunction{FInjection}{Injection}
	\SetKwFunction{FUpd}{FeatureUpdate}
	\SetKwComment{Comment}{/* }{ */}

	\KwInput{A graph $\gG=(A,X)$, a trained GNN model $f_{\theta^*}$, number of injected nodes $k$, degree budget $b$, outer attack epochs $e_{\text{outer}}$, inner attack epochs for node features and adjacency matrix $e^X_{\text{inner}},e^A_{\text{inner}}$, learning rate $\eta$, weight for sparsity penalty $\beta$, weight for homophily penalty $\lambda$,
	sequential step for vicious nodes $\gamma_\atk$, sequential step for target nodes $\gamma_c$ \;}
	\KwOutput{Perturbed graph $\gG'=(A', X')$\;}

	Initialize injection parameters ($A_\atk, X_\atk$)\;
	$\mY_{\text{orig}} \leftarrow f_{\theta^*}(A,X)$ \; \Comment*[r]{Obtain original predictions on clean graph}
	\While{Not Injecting All Nodes}
	{
	$n_\atk \leftarrow  \gamma_\atk*|V_\atk|$; $n_c \leftarrow \gamma_c*|V_c|$ \;
	Ranking and selecting $n_c$ targets with Eq.~\ref{eq:tdgia+_score}\;
	Random initialize $A_\atk^{(\text{cur})}\in\R^{n_c\times n_\atk},X_\atk^{(\text{cur})} \in \R^{n_\atk\times d}$ \;

	\For{epoch $\leftarrow$ $0$ to $e_{\text{outer}}$}
	{
	\For{epoch $\leftarrow$ $0$ to $e^X_{\text{inner}}$}
	{
	$A'\leftarrow A\concat A_\atk \concat A_\atk^{(\text{cur})}, X'\leftarrow X\concat X_\atk \concat X_\atk^{(\text{cur})} $\;
	$X^{(\text{cur})}_\atk \leftarrow \text{Clip}_{(x_{\min},x_{\max})}(X_\atk^{(\text{cur})} - \eta \cdot \nabla_{X^{(\text{cur})}_\atk}(\mathcal{L}^h_{\text{atk}}))$ \;
	}
	\For{epoch $\leftarrow$ $0$ to $e^A_{\text{inner}}$}
	{
	$A'\leftarrow A\concat A_\atk \concat A_\atk^{(\text{cur})}, X'\leftarrow X\concat X_\atk \concat X_\atk^{(\text{cur})} $\;
	$A_\atk^{(\text{cur})} \leftarrow \text{Clip}_{(0,1)}(A_\atk^{(\text{cur})} - \eta \cdot \nabla_{A_\atk^{(\text{cur})}}(\mathcal{L}^A_{\text{atk}}))$ \;
	}
	$A_\atk^{(\text{cur})} \leftarrow \bigparallel_{i=1}^{n_\atk}\argmax_{\text{top}\ b}(A_{\atk[i, :]}^{(\text{cur})})$ \;
	}
	$A_\atk$=$A_\atk$ $\Vert$ $A_\atk^{(\text{cur})}$; $X_\atk$=$X_\atk$ $\Vert$ $X_\atk^{(\text{cur})}$\;
	}
\end{algorithm}

Actually, one may also inject few nodes via heuristic based algorithms first, then inject the left nodes with gradients sequentially.
Assume that $\alpha$ nodes are injected by heuristic, we may further optimize the complexity
from
\[
	O(\frac{1}{\gamma_\atk}(|V_c|\log|V_c|+ e_{\text{outer}}(e^A_{\text{inner}}|V_c|\gamma_c|V_\atk|+e^X_{\text{inner}}|V_\atk| d))N_{V_c})
\]
to
\[
	\begin{aligned}
		O(\alpha\frac{1}{\gamma_\atk}(|V_c|\log|V_c|+   & |V_\atk|b+e^X_{\text{inner}}|V_\atk|d)N_{V_c}+                                                  \\
		(1-\alpha)\frac{1}{\gamma_\atk}(|V_c|\log|V_c|+ & e_{\text{outer}}(e^A_{\text{inner}}|V_c|\gamma_c|V_\atk|+e^X_{\text{inner}}|V_\atk| d))N_{V_c})
	\end{aligned}
\]
in Table~\ref{tab:complexity}.
