# Supplementary material for: Nuclear matrix elements for neutrinoless double beta decays and spin-dipole giant resonances
Source: arXiv:2202.00361 source file (2022-02-14)
Supplement: Supplementary file 2 [file 7_appendix_2.tex]

% Appendix about experiments

\section{More Details about the Experiments}
\label{sec:experiment_appdx}


\subsection{Statistics and Budgets of Datasets}
\label{sec:datasets_appdx}
Here we provide statistics of datasets used in the experiments as Sec.~\ref{sec:exp_setups}.
The label homophily utilizes the previous homophily definition~\citep{beyond_homophily},
while the avg. homophily utilizes the node-centric homophily based on node similarity.

\begin{table}[!ht]
	\centering\small
	\caption{Statistics of datasets}
	\label{tab:datasets}%\resizebox{\textwidth}{!}{
	\begin{tabular}{lcccccc}
		\toprule
		\textbf{Datasets} & \textbf{Nodes} & \textbf{Edges} & \textbf{Classes} & \textbf{Avg. Degree} & \textbf{Label Homophily} & \textbf{Avg. Homophily} \\\midrule
		Cora              & $2680$         & $5148$         & $7$              & $3.84$               & $0.81$                   & $0.59$                  \\
		Citeseer          & $3191$         & $4172$         & $6$              & $2.61$               & $0.74$                   & $0.90$                  \\
		Computers         & $13,752$       & $245,861$      & $10$             & $35.76$              & $0.77$                   & $0.31$                  \\
		Arxiv             & $169,343$      & $1,166,243$    & $40$             & $13.77$              & $0.65$                   & $0.86$                  \\
		Aminer            & $659,574$      & $2,878,577$    & $18$             & $8.73$               & $0.65$                   & $0.38$                  \\
		Reddit            & $232,965$      & $11,606,919$   & $41$             & $99.65$              & $0.78$                   & $0.31$                  \\\bottomrule
	\end{tabular}%}
\end{table}
Following previous works~\citep{tdgia,grb}, we heuristically specify the budgets for each dataset according to the the number of target nodes and average degrees.

\begin{table}[!ht]
	\centering\small
	\caption{Budgets for non-targeted attacks on different datasets}
	\label{tab:datasets_budget_nontarget}
	\begin{tabular}{lcccccc}
		\toprule
		\textbf{Datasets} & \textbf{Nodes} & \textbf{Degree} & \textbf{Node Per.($\%$)} & \textbf{Edge Per.($\%$)} \\\midrule
		Cora              & $60$           & $20$            & $2.24\%$                 & $23.31\%$                \\
		Citeseer          & $90$           & $10$            & $2.82\%$                 & $21.57\%$                \\
		Computers         & $300$          & $150$           & $2.18\%$                 & $18.30\%$                \\
		Arxiv             & $1500$         & $100$           & $0.71\%$                 & $10.29\%$                \\\bottomrule
	\end{tabular}
\end{table}

For targeted attack, we follow previous works~\citep{nettack} to select $800$ nodes as targets according to the classification margins of the surrogate model.
Specifically, we select $200$ nodes with the highest classification margin, $200$ nodes with lowest classification margin and $400$ randomly.
For the budgets, we scale down the number of injected nodes and the maximum allowable degrees accordingly.
\begin{table}[!h]
	\centering\small
	\caption{Budgets of targeted attacks on different datasets}
	\label{tab:datasets_budget_target}
	\begin{tabular}{lcccccc}
		\toprule
		\textbf{Datasets} & \textbf{Nodes} & \textbf{Degree} & \textbf{Node Per.($\%$)} & \textbf{Edge Per.($\%$)} \\\midrule
		Computers         & $100$          & $150$           & $0.73\%$                 & $6.1\%$                  \\
		Arxiv             & $120$          & $100$           & $0.07\%$                 & $1.03\%$                 \\
		Aminer            & $150$          & $50$            & $0.02\%$                 & $0.26\%$                 \\
		Reddit            & $300$          & $100$           & $0.13\%$                 & $0.26\%$                 \\\bottomrule
	\end{tabular}
\end{table}

\subsection{Additional Discussions about Attack Baselines}
\label{sec:exp_rl_appdx}
For the selection of attack baselines, from the literature reviews~\citep{sun_gadv_survey,deeprobust},
existing reinforcement learning (RL) based approaches adopt different settings from ours, which either focus on the
poisoning attack, transductive learning, edge perturbation or other application tasks.
Even for NIPA~\citep{nipa} which has the closest setting to ours,
since it focuses on poisoning and transductive attack, and the features of the injected nodes are generated heuristically according to the labels assigned by the RL agent,
without author released code, the adaption requires lots of efforts including redesigning the markov decision process in NIPA,
hence we would like to leave them for future work. More discussions on RL based future works are given in Appendix~\ref{sec:future_direction_appdx}.


\subsection{Complexity of Algorithms}
\label{sec:gia_alg_complexity}
Here we provide complexity analyses of the GIA algorithms used in the experiments as discussed and selected in Sec.~\ref{sec:exp_setups}.
As also defined in algorithm description section from Appendix~\ref{sec:gia_alg_desc}, $e^X_{\text{inner}}$ is the number of epochs optimized for node features,
$b$ is the number of maximum degree of vicious nodes, $d$ is the number of feature dimension,
$N_{V_c}$ is the number of $k$-hop neighbors of the victim nodes for perform one forwarding of a $k$-layer GNN,
$e_{\text{outer}}$ is the number of epochs for optimizing $A_\atk$,
$\gamma_c$ is the ratio of target nodes to attack in one batch,
$\gamma_\atk$ is the ratio of vicious nodes to inject in one batch.
\bgroup
\def\arraystretch{2}
\begin{table}[!h]
	\centering
	\caption{Complexity of various attacks}
	\label{tab:complexity}
	\resizebox{\textwidth}{!}{
		\begin{tabular}{clcc}
			\toprule
			\textbf{Type} & \multicolumn{1}{c}{\textbf{Algorithm}}                                      & \textbf{Time Complexity}                                                                                                                   & \textbf{Space Complexity} \\ \hhline{----}
			\multirow{3}{*}{\small{Gradient}}
			              & MetaGIA                                                                     & $O(|V_\atk|b(|V_c||V_\atk|\log(|V_c||V_\atk|)+e^X_{\text{inner}}d(|V_\atk|+N_{V_c})))$
			              & $O(|V_c||V_\atk|+e^X_{\text{inner}}d(|V_\atk|+N_{V_c}))$
			\\\hhline{~|-|-|-}
			              & AGIA                                                                        & $O(e_{\text{outer}}(e^A_{\text{inner}}|V_c||V_\atk|+(e^A_{\text{inner}}+e^X_{\text{inner}})d(N_{V_c}+|V_\atk|)))$
			              & $O(|V_c||V_\atk|+e^X_{\text{inner}}d(|V_\atk|+N_{V_c}))$
			\\\hhline{~|-|-|-}
			              & AGIA-SeqGIA                                                                 & $O(e_{\text{outer}}(|V_c|\log(|V_c|)+e^A_{\text{inner}}\gamma_c|V_c||V_\atk|+(e^A_{\text{inner}}+e^X_{\text{inner}})d(N_{V_c}+|V_\atk|)))$
			              & $O(\gamma_c|V_c|\gamma_\atk|V_\atk|+e^X_{\text{inner}}d(|V_\atk|+N_{V_c}))$
			\\\hhline{====}
			\multirow{4}{*}{\small{Heuristic}}
			              & PGD
			              & $O(|V_\atk|b+e^X_{\text{inner}}d(|V_\atk|+N_{V_c}))$
			              & $O(|V_\atk|b+e^X_{\text{inner}}d(|V_\atk|+N_{V_c}))$
			\\\hhline{~|-|-|-}
			              & TDGIA
			              & $O((|V_c|\log|V_c|+|V_\atk|b+e^X_{\text{inner}}d(|V_\atk|+N_{V_c}))$
			              & $O(|V_\atk|b+e^X_{\text{inner}}d(|V_\atk|+N_{V_c}))$
			\\\hhline{~|-|-|-}
			              & ATDGIA                                                                      & $O(|V_c|\log|V_c|+|V_\atk|b+e^X_{\text{inner}}d(|V_\atk|+N_{V_c}))$
			              & $O(|V_\atk|b+e^X_{\text{inner}}d(|V_\atk|+N_{V_c}))$
			\\\bottomrule
		\end{tabular}}
\end{table}
\egroup

\subsection{Details of Defense Baselines}
\label{sec:baseline_detail_appdx}
Here we provide the categories of defense models used in the experiments as Sec.~\ref{sec:exp_setups}.
We categorize all models into Vanilla, Robust and Extreme Robust (Combo).
Basically, popular GNNs are belong to vanilla category, robust GNNs are belong to robust categorty,
and a robust trick will enhance the robust level by one to the next Category.
Consistenly to the observation in GRB~\citep{grb}, we find adding Layer Normalization~\citep{layer_norm} before or between convulotion layers can enhance the model robustness.
We use LN to denote adding layer norm before the first convulotion layer and LNi to denote adding layer norm between convulotion layers.
\bgroup
\def\arraystretch{1.5}
\begin{table}[H]
	\caption{Defense model categories}
	\label{tab:defense_category}
	\resizebox{\textwidth}{!}{
		\begin{tabular}{lc|lc|lc|lc}
			\textbf{Model} & \textbf{Category} & \textbf{Model} & \textbf{Category} & \textbf{Model}  & \textbf{Category} & \textbf{Model}     & \textbf{Category} \\ \midrule
			GCN            & Vanilla           & GCN+LN         & Robust            & GCN+LNi         & Robust            & GCN+FLAG           & Robust            \\
			GCN+LN+LNi     & Combo             & GCN+FLAG+LN    & Combo             & GCN+FLAG+LNi    & Combo             & GCN+FLAG+LN+LNi    & Combo             \\\hline
			Sage           & Vanilla           & Sage+LN        & Robust            & Sage+LNi        & Robust            & Sage+FLAG          & Robust            \\
			Sage+LN+LNi    & Combo             & Sage+FLAG+LN   & Combo             & Sage+FLAG+LNi   & Combo             & Sage+FLAG+LN+LNi   & Combo             \\\hline
			GAT            & Vanilla           & GAT+LN         & Robust            & GAT+LNi         & Robust            & GAT+FLAG           & Robust            \\
			GAT+LN+LNi     & Combo             & GAT+FLAG+LN    & Combo             & GAT+FLAG+LNi    & Combo             & GAT+FLAG+LN+LNi    & Combo             \\\hline
			Guard          & Robust            & Guard+LN       & Combo             & Guard+LNi       & Combo             & EGuard+FLAG        & Combo             \\
			Guard+LN+LNi   & Combo             & EGuard+FLAG+LN & Combo             & EGuard+FLAG+LNi & Combo             & EGuard+FLAG+LN+LNi & Combo             \\\hline
			RGAT           & Robust            & RGAT+LN        & Combo             & RGAT+FLAG       & Combo             & RGAT+FLAG+LN       & Combo             \\\hline
			RobustGCN      & Robust            & RobustGCN+FLAG & Combo             &                 &                   &                    &                   \\
		\end{tabular}
	}
\end{table}
\egroup

\subsection{Details of Evaluation and Model Settings}
\label{sec:model_setting_appdx}
\subsubsection{Model Setting}
By default, all GNNs used in our experiments have $3$ layers, a hidden dimension of $64$ for Cora, Citeseer, and Computers, a hidden dimension of $128$ for the rest medium to large scale graphs. We also adopt dropout~\citep{dropout} with dropout rate of $0.5$ between each layer. The optimizer we used is Adam~\citep{adam} with a learning rate of $0.01$. By default, we set total training epochs as $400$ and employ the early stop of $100$ epochs according to the validation accuracy. For the set of threshold in homophily defenders, we use PGD~\citep{pgd} to find the threshold which performs well on both the clean data and perturbed data. By default, we set the threshold as $0.1$, while for Computers and Reddit, we use $0.15$ for Guard and EGuard, and for Citeseer and Arxiv we use $0.2$ for RGAT.

For adversarial training with FLAG~\citep{flag}, we set the step size be $1\times 10^{-3}$, and train $100$ steps for Cora, $50$ steps for Citeseer, $10$ steps for the rest datasets. We empirically observe that FLAG can enhance both the natural accuracy and robustness of GNNs. We refer readers to the results for more details in Sec.~\ref{sec:eval_nontarget_detailed} and Sec.~\ref{sec:eval_target_detailed}.

\subsubsection{Evaluation Setting}
For final model selection, we select the final model with best validation accuracy.
For data splits, we follow the split methods in GRB~\citep{grb} which splits the datasets according to the node degrees, except for non-targeted attack on Arxiv where we use the official split to probe the performances of various methods in a natural setting.
For non-targeted attack, following previous works~\citep{tdgia,grb}, we select all test nodes as targets.
While for targeted attacks, we follow previous works~\citep{nettack} to select $200$ nodes with highest classification margin and lowest classification margin of the surrogate model. Then we randomly select $400$ nodes as targets. In other words, there are $800$ target nodes in total for targeted attack. Note for targeted attack, the natural accuracy on the target nodes might be different from normal test accuracy.
We also follow previous works to specify the attack budgets as Table.~\ref{tab:datasets_budget_nontarget} for non-targeted attack and Table.~\ref{tab:datasets_budget_target} for targeted attack.

During evaluation, we follow the black-box setting. Specifically, we firstly use the surrogate model to generate the perturbed graph, then we let the target models which has trained on the clean graph to test on the perturbed graph. We repeat the evaluation for $10$ times on Cora, Citeseer, Computers, and Arxiv, and $5$ times for Aminer and Reddit since model performs more stably on large graphs. Then we report mean test accuracy of the target models on the target nodes and omit the variance due to the space limit.

\subsubsection{Attacks Setting}
By default, we use PGD~\citep{pgd} to generate malicious node features. The learning step is $0.01$ and the default training epoch is $500$. We also employ the early stop of $100$ epochs according to the accuracy of the surrogate model on the target nodes. While for heuristic approaches such as TDGIA~\citep{tdgia} and ATDGIA, we follow the setting of TDGIA to update the features. Empirically, we find the original TDGIA feature update suits better for heuristic approaches while they show no advance over PGD for other approaches. Besides, as Table~\ref{tab:complexity} shows, MetaGIA requires huge amount of time originally. Thus, to scale up, we use a batch update which updates the injected edges by a step size of $b$, i.e., the maximum degree of injected nodes, and limit the overall update epochs by $|V_\atk|/6$, where we empirically observe this setting performs best in Cora hence we stick it for the other datasets.

For the setting of $\lambda$ for HAO, we search the parameters within $0.5$ to $8$ by a step size of $0.5$ such that the setting of $\lambda$ will not degenerate the performance of the attacks on surrogate model. Besides heuristic approaches, we additionally use a hinge loss to stabilize the gradient information from $\mathcal{L}_\atk$ and $C(\gG,\gG')$, where the former can be too large that blurs the optimization direction of the latter. Take Cross Entropy with $\log\_\text{softmax}$ as an example, we adopt the following to constrict the magnitude of $\mathcal{L}_\atk$:
\begin{equation}
	\label{eq:cross_entropy_hinge}
	\begin{aligned}
		{\mathcal{L}_\atk}_{[u]} & = (-H^{(k)}_{[u,Y_u]})\cdot \mathbf{1}\{\frac{\exp(H^{(k)}_{[u,Y_u]})}{\sum_{i}\exp(H^{(k)}_{[u,i]})}\geq \tau\}              \\
		                         & +\log(\sum_{i}\exp(H^{(k)}_{[u,i]}\cdot \mathbf{1}\{\frac{\exp(H^{(k)}_{[u,i]})}{\sum_{j}\exp(H^{(k)}_{[u,j]})}\geq \tau\})),
	\end{aligned}
\end{equation}
where $\mathbf{1}\{\frac{\exp(H^{(k)}_{[u,Y_u]})}{\sum_{i}\exp(H^{(k)}_{[u,i]})}\geq \tau\}$ can be taken as the predicted probability for $Y_u=u$ and $\tau$ is the corresponding threshold for hinge loss that we set as $1\times 10^{-8}$.

For the hyper-parameter setting of our proposed strategies in Sec.~\ref{sec:gia_algorithm}, we find directly adopting $\lambda$ in PGD for $\lambda_X$ and setting $\lambda_A=0$ performs empirically better. Hence we stick to the setting for $\lambda_A$ and $\lambda_X$. For the weight of sparsity regularization term in AGIA, we directly adopt $1/b$. For the hyper-parameters in heuristic methods, we directly follow TDGIA~\citep{tdgia}. For SeqGIA, we set $\gamma_\atk$ be $\min(0.2,\floor{|V_c|/2b})$ and $\gamma_c=\min(|V_c|,\gamma_\atk|V_\atk|b)$ by default.


\subsection{Software and Hardware}
We implement our methods with PyTorch~\citep{pytorch} and PyTorch Geometric~\citep{pytorch_geometric}.
We ran our experiments on Linux Servers with 40 cores Intel(R) Xeon(R) Silver 4114 CPU @ 2.20GHz, 256 GB Memory, and Ubuntu 18.04 LTS installed. One has 4 NVIDIA RTX 2080Ti graphics cards with CUDA 10.2 and the other has 2 NVIDIA RTX 2080Ti and 2 NVIDIA RTX 3090Ti graphics cards with CUDA 11.3.


\section{More Experimental Results }
In this section, we provide more results from experiments about HAO to further validate its effectiveness.
Specifically, we provide full results of averaged attack performance across all defense models,
as well as initial experiments of HAO on two disassortative graphs.

\subsection{Full Results of Averaged Attack Performance}
In this section, we provide full results of averaged attack performance across all defense models, as a supplementary for Table~\ref{tab:averaged_performance}.
\begin{table}[t]
	\caption{Full averaged performance across all defense models}
	\label{tab:averaged_performance_full_appdx}
	\scriptsize
	\centering\resizebox{\textwidth}{!}{
		\begin{tabular}{lcccccccc}
			\toprule
			\textbf{Model} & \textbf{Cora}$^\dagger$ & \textbf{Citeseer}$^\dagger$ & \textbf{Computers}$^\dagger$ & \textbf{Arxiv}$^\dagger$ & \textbf{Arxiv}$^\ddagger$ & \textbf{Computers}$^\ddagger$ & \textbf{Aminer}$^\ddagger$ & \textbf{Reddit}$^\ddagger$ \\\midrule
			Clean          & $84.74$                 & $74.10$                     & $92.25$                      & $70.44$                  & $70.44$                   & $91.68$                       & $62.39$                    & $95.51$                    \\
			PGD            & $61.09$                 & $54.08$                     & $61.75$                      & $54.23$                  & $36.70$                   & $62.41$                       & $26.13$                    & $62.72$                    \\
			\hfill +HAO    & $\underline{56.63}$     & $48.12$                     & $\underline{59.16}$          & $\underline{45.05}$      & $28.48$                   & $59.09$                       & $\underline{22.15}$        & $56.99$                    \\
			MetaGIA        & $60.56$                 & $53.72$                     & $61.75$                      & $53.69$                  & $28.78$                   & $62.08$                       & $32.78$                    & $60.14$                    \\
			\hfill +HAO    & $58.51$                 & $47.44$                     & $60.29$                      & $48.48$                  & $\underline{24.61}$       & $\underline{58.63}$           & $29.91$                    & $\mathbf{54.14}$           \\
			AGIA           & $60.10$                 & $54.55$                     & $60.66$                      & $48.86$                  & $32.68$                   & $61.98$                       & $31.06$                    & $59.96$                    \\
			\hfill +HAO    & $\mathbf{53.79}$        & $48.30$                     & $\mathbf{58.71}$             & $48.86$                  & $29.52$                   & $\mathbf{58.37}$              & $26.51$                    & $56.36$                    \\
			TDGIA          & $66.86$                 & $52.45$                     & $66.79$                      & $49.73$                  & $31.68$                   & $62.47$                       & $32.37$                    & $57.97$                    \\
			\hfill +HAO    & $65.22$                 & $\underline{46.61}$         & $65.46$                      & $49.54$                  & $\mathbf{22.04}$          & $59.67$                       & $22.32$                    & $\underline{54.32}$        \\
			ATDGIA         & $61.14$                 & $49.46$                     & $65.07$                      & $46.53$                  & $32.08$                   & $64.66$                       & $24.72$                    & $61.25$                    \\
			\hfill +HAO    & $58.13$                 & $\mathbf{43.41}$            & $63.31$                      & $\mathbf{44.40}$         & $29.24$                   & $59.27$                       & $\mathbf{17.62}$           & $56.90$                    \\\bottomrule
			\multicolumn{9}{l}{The lower is better. $^\dagger$Non-targeted attack. $^\ddagger$Targeted attack.  }
		\end{tabular}}
\end{table}


\subsection{More Results on Disassortative Graphs}
In this section, we provide initial investigation into the non-targeted attack performances of various GIA methods with or without HAO on disassortative graphs.
Specifically, we select Chameleon and Squirrel provided by~\cite{geom_gcn}. Statistics and budgets used for attack are given in Table~\ref{tab:datasets_nonhomo} and Table~\ref{tab:datasets_budget_nontarget_nonhomo}.

\begin{table}[!h]
	\centering\small
	\caption{Statistics of the disassortative datasets}
	\label{tab:datasets_nonhomo}%\resizebox{\textwidth}{!}{
	\begin{tabular}{lcccccc}
		\toprule
		\textbf{Datasets} & \textbf{Nodes} & \textbf{Edges} & \textbf{Classes} & \textbf{Avg. Degree} & \textbf{Label Homophily} & \textbf{Avg. Homophily} \\\midrule
		Chameleon         & $2277$         & $31,421$       & $5$              & $27.60$              & $0.26$                   & $0.62$                  \\
		Squirrel          & $5201$         & $198,493$      & $5$              & $76.33$              & $0.23$                   & $0.58$                  \\\bottomrule
	\end{tabular}%}
\end{table}
We also heuristically specify the budgets for each dataset according the the number of target nodes and average degrees.

\begin{table}[!h]
	\centering\small
	\caption{Budgets for non-targeted attacks on disassortative datasets}
	\label{tab:datasets_budget_nontarget_nonhomo}
	\begin{tabular}{lcccccc}
		\toprule
		\textbf{Datasets} & \textbf{Nodes} & \textbf{Degree} & \textbf{Node Per.($\%$)} & \textbf{Edge Per.($\%$)} \\\midrule
		Chameleon         & $60$           & $100$           & $2.64\%$                 & $19.10\%$                \\
		Squirrel          & $90$           & $50$            & $1.73\%$                 & $2.27\%$                 \\\bottomrule
	\end{tabular}
\end{table}

For the settings of hyperparameters in attack methods and evaluation, we basically follow the same setup as given in Appendix~\ref{sec:model_setting_appdx}.
In particular, we find using a threshold of $0.05$ for homophily defenders work best on Chameleon.
Besides, we also observe robust tricks can not always improve performances of GNNs on these graphs.
For example, we observe that using a large step-size of FLAG may degenerate the performances of GNNs on these datasets,
hence we use a smaller step-size of $5\times 10^{-4}$ as well as a small number of steps of $10$.
Moreover, using a LN before the first GNN layer may also hurt the performance.
For fair comparison, we remove these results from defenses.
Finally, in Table~\ref{tab:eval_non_targeted_nonhomo_appdx},
we report both categorized defense results as Table~\ref{tab:eval_non_targeted} as well as the averaged attack performance as Table~\ref{tab:averaged_performance}.

% \bgroup
% \setlength{\tabcolsep}{5pt}
\begin{table}[t]
	\caption{Results of non-targeted attacks on disassortative graphs}
	\label{tab:eval_non_targeted_nonhomo_appdx}
	%\resizebox{\textwidth}{!}{
	\scriptsize\centering
	\begin{tabular}{@{}{l}*{10}{c}@{}}
		%\begin{tabular}{@{}l*{10}{c}@{}}
		\toprule
		                                         &              & \multicolumn{4}{c}{{\small Chameleon ($\downarrow$)}} & \multicolumn{4}{c}{{\small Squirrel($\downarrow$)}}                                                                                                                                                                                                                               \\\cmidrule(lr){3-6}\cmidrule(lr){7-10}
		                                         & HAO          & \multicolumn{1}{c}{\textbf{Homo}}                     & \multicolumn{1}{c}{\textbf{Robust}}                 & \multicolumn{1}{c}{\textbf{Combo}} & \multicolumn{1}{c}{\textbf{AVG.}} & \multicolumn{1}{c}{\textbf{Homo}} & \multicolumn{1}{c}{\textbf{Robust}} & \multicolumn{1}{c}{\textbf{Combo}} & \multicolumn{1}{c}{\textbf{AVG.}} & \\ \midrule
		Clean                                    &              & $61.89$                                               & $65.18$                                             & $64.92$                            & $62.58$                           & $37.33$                           & $43.88$                             & $45.87$                            & $40.04$                             \\  \hdashline[0.5pt/1pt]
		\rule{0pt}{10pt}PGD                      &              & $61.89$                                               & $61.89$                                             & $63.61$                            & $\underline{33.24}$               & $35.66$                           & $36.28$                             & $40.54$                            & $\underline{26.03}$                 \\
		PGD                                      & $\checkmark$ & $52.78$                                               & $57.87$                                             & $59.31$                            & $38.00$                           & $33.32$                           & $39.36$                             & $35.83$                            & $26.37$                             \\\hdashline[0.5pt/1pt]
		\rule{0pt}{10pt}MetaGIA$^\dagger$        &              & $61.89$                                               & $61.89$                                             & $63.61$                            & $34.38$                           & $35.66$                           & $\mathbf{35.66}$                    & $39.40$                            & $26.09$                             \\
		MetaGIA$^\dagger$                        & $\checkmark$ & $49.25$                                               & $55.83$                                             & $55.73$                            & $33.63$                           & $34.07$                           & $38.26$                             & $\mathbf{35.24}$                   & $\mathbf{25.81}$                    \\
		AGIA$^\dagger$                           &              & $61.89$                                               & $61.89$                                             & $63.61$                            & $35.95$                           & $35.66$                           & $\underline{35.89}$                 & $39.93$                            & $26.93$                             \\
		AGIA$^\dagger$                           & $\checkmark$ & $\underline{43.98}$                                   & $\mathbf{48.88}$                                    & $\mathbf{53.33}$                   & $\mathbf{32.03}$                  & $35.69$                           & $36.31$                             & $36.40$                            & $26.77$                             \\\hdashline[0.5pt/1pt]
		\rule{0pt}{10pt}TDGIA                    &              & $61.95$                                               & $61.95$                                             & $63.76$                            & $41.17$                           & $35.66$                           & $\mathbf{35.66}$                    & $40.81$                            & $29.02$                             \\
		TDGIA                                    & $\checkmark$ & $46.36$                                               & $\underline{51.12}$                                 & $\underline{55.14}$                & $38.90$                           & $\mathbf{31.51}$                  & $38.21$                             & $\underline{35.63}$                & $28.65$                             \\
		ATDGIA                                   &              & $61.95$                                               & $61.95$                                             & $63.76$                            & $41.11$                           & $35.66$                           & $\mathbf{35.66}$                    & $41.62$                            & $29.62$                             \\
		ATDGIA                                   & $\checkmark$ & $\mathbf{36.93}$                                      & $57.75$                                             & $59.25$                            & $38.88$                           & $\underline{32.02}$               & $40.00$                             & $40.62$                            & $30.24$                             \\\hdashline[0.5pt/1pt]
		\hdashline[0.5pt/3pt]\rule{0pt}{10pt}MLP &              & \multicolumn{4}{c}{{$50.15$}}                         & \multicolumn{4}{c}{{$32.51$}}                                                                                                                                                                                                                                                     \\ \bottomrule
		\multicolumn{10}{l}{$^\downarrow$The lower number indicates better attack performance.  $^\dagger$Runs with SeqGIA framework on Computers and Arxiv.  }                                                                                                                                                                                                                                             \\                                                                                                                                                                                                                                                                                                                                              \\
	\end{tabular}%}
\end{table}
% \egroup

From the results, we observe that, although our methods are not initially designed for disassortative graphs, HAO still brings empirical improvements.
Specifically, on Chameleon, HAO improves the attack performance up to $25\%$ against homophily defenders, up to $12\%$ against robust models, up to $10\%$ against extreme robust models,
and finally brings up to $3\%$ averaged test robustness of all models.
While on Squirrel, the improvements become relatively low while still non-trivial. For example, HAO improves the attack performance up to $4\%$ in terms of test robustness against homophily defenders.
We hypothesize the reason why HAO also works on disassortative graphs is because GNN can still learn the homophily information implicitly, e.g., similarity between class label distributions~\citep{is_homophily_necessity},
which we will leave the in-depth analyses to future work.

\section{Detailed Results of Attack Performance}

\subsection{Detailed Results of Non-Targeted Attacks}
\label{sec:eval_nontarget_detailed}
In this section, we present the detailed non-targeted attack results of the methods and datasets used in our experiments for Table~\ref{tab:eval_non_targeted}.
For simplicity, we only give the results of top $20$ robust models according to the averaged test accuracy against all attacks.


\bgroup
\def\arraystretch{1.6}
\begin{table}[!t]
	\caption{Detailed results of non-targeted attacks on Cora (1)}
	\label{tab:eval_nontarget_detailed_cora1}
	\resizebox{\textwidth}{!}{
		\begin{tabular}{l*{10}{>{$}c<{$}}}
			\toprule
			             & \text{\scriptsize EGuard+LNi+FLAG+LN} & \text{\scriptsize EGuard+FLAG+LN} & \text{\scriptsize EGuard+LNi+FLAG} & \text{\scriptsize Guard+LNi+LN} & \text{\scriptsize RGAT+FLAG+LN} & \text{\scriptsize GCN+LNi+FLAG+LN} & \text{\scriptsize RobustGCN+FLAG} & \text{\scriptsize RGAT+LN} & \text{\scriptsize Guard+LN} & \text{\scriptsize EGuard+FLAG} \\ \midrule
			Clean        & 83.48                                 & 84.17                             & 85.9                               & 79.56                           & 87.29                           & 86.37                              & 86.21                             & 85.29                      & 81.72                       & 85.56                          \\\hdashline[0.5pt/1pt]
			PGD          & 82.53                                 & 83.94                             & 85.74                              & 79.74                           & 76.78                           & 71.10                              & 69.57                             & 79.56                      & 81.44                       & 85.35                          \\
			\hfill +HAO  & 77.99                                 & 73.04                             & 66.25                              & 74.21                           & 68.09                           & 71.06                              & 70.3                              & 67.92                      & 68.12                       & 53.99                          \\
			MetaGIA      & 82.68                                 & 83.96                             & 85.86                              & 79.51                           & 75.18                           & 69.72                              & 69.4                              & 78.04                      & 81.59                       & 85.48                          \\
			\hfill +HAO  & 69.49                                 & 65.92                             & 66.83                              & 63.02                           & 66.38                           & 71.86                              & 76.8                              & 57.75                      & 55.35                       & 56.77                          \\
			AGIA         & 82.75                                 & 83.69                             & 85.78                              & 79.56                           & 75.77                           & 69.25                              & 69.10                             & 79.10                      & 81.43                       & 85.34                          \\
			\hfill +HAO  & 75.25                                 & 69.10                             & 61.00                              & 70.12                           & 65.48                           & 69.86                              & 71.08                             & 62.76                      & 60.96                       & 48.54                          \\
			TDGIA        & 83.13                                 & 83.65                             & 85.72                              & 79.13                           & 82.37                           & 79.31                              & 76.11                             & 82.2                       & 81.37                       & 85.39                          \\
			\hfill +HAO  & 77.93                                 & 73.58                             & 75.47                              & 73.67                           & 75.18                           & 79.45                              & 78.63                             & 69.58                      & 64.66                       & 65.31                          \\
			ATDIGA       & 82.57                                 & 83.54                             & 85.39                              & 79.38                           & 78.76                           & 76.09                              & 73.08                             & 79.8                       & 81.47                       & 84.88                          \\
			\hfill +HAO  & 74.43                                 & 71.88                             & 71.21                              & 66.97                           & 72.51                           & 76.87                              & 76.17                             & 60.61                      & 62.38                       & 63.53                          \\\hdashline[0.5pt/1pt]
			\textbf{AVG} & 79.29                                 & 77.86                             & 77.74                              & 74.99                           & 74.89                           & 74.63                              & 74.22                             & 72.96                      & 72.77                       & 72.74                          \\\bottomrule
		\end{tabular}}
\end{table}
\egroup

\bgroup
\def\arraystretch{1.5}
\begin{table}[t]
	\caption{Detailed results of non-targeted attacks on Cora (2)}
	\label{tab:eval_nontarget_detailed_cora2}
	\resizebox{\textwidth}{!}{
		\begin{tabular}{l*{10}{>{$}c<{$}}}
			\toprule
			             & \text{\scriptsize RGAT+FLAG} & \text{\scriptsize Guard+LNi} & \text{\scriptsize RobustGCN} & \text{\scriptsize GCN+FLAG+LN} & \text{\scriptsize GCN+LNi+FLAG} & \text{\scriptsize RGAT} & \text{\scriptsize GAT+LNi+FLAG+LN} & \text{\scriptsize Sage+LNi+FLAG+LN} & \text{\scriptsize Guard} & \text{\scriptsize GCN+LNi+LN} \\ \midrule
			Clean        & 87.21                        & 83.18                        & 84.63                        & 85.86                          & 86.36                           & 85.74                   & 86.55                              & 84.95                               & 83.61                    & 84.47                         \\\hdashline[0.5pt/1pt]
			PGD          & 76.93                        & 83.11                        & 63.20                        & 62.55                          & 60.68                           & 79.28                   & 61.29                              & 61.84                               & 83.08                    & 58.46                         \\
			\hfill +HAO  & 62.35                        & 53.68                        & 62.60                        & 63.60                          & 61.69                           & 52.60                   & 62.81                              & 62.34                               & 44.02                    & 58.78                         \\
			MetaGIA      & 75.14                        & 83.08                        & 63.53                        & 59.18                          & 60.36                           & 77.97                   & 57.88                              & 61.01                               & 83.61                    & 58.10                         \\
			\hfill +HAO  & 61.53                        & 57.31                        & 69.83                        & 67.00                          & 66.64                           & 49.25                   & 65.82                              & 65.69                               & 45.41                    & 61.94                         \\
			AGIA         & 76.04                        & 83.08                        & 62.67                        & 61.26                          & 59.09                           & 78.95                   & 57.84                              & 58.61                               & 83.44                    & 57.05                         \\
			\hfill +HAO  & 57.17                        & 49.12                        & 61.59                        & 62.65                          & 59.25                           & 47.24                   & 59.80                              & 59.56                               & 39.87                    & 55.62                         \\
			TDGIA        & 82.02                        & 83.04                        & 71.34                        & 71.35                          & 73.47                           & 81.79                   & 71.52                              & 70.30                               & 83.44                    & 70.69                         \\
			\hfill +HAO  & 70.52                        & 67.04                        & 73.38                        & 73.52                          & 75.00                           & 56.95                   & 71.96                              & 71.56                               & 50.79                    & 72.90                         \\
			ATDIGA       & 79.06                        & 82.85                        & 66.96                        & 69.61                          & 65.89                           & 79.91                   & 65.57                              & 63.81                               & 83.07                    & 62.95                         \\
			\hfill +HAO  & 64.50                        & 55.13                        & 70.30                        & 72.46                          & 70.94                           & 42.18                   & 69.26                              & 67.59                               & 40.46                    & 65.53                         \\\hdashline[0.5pt/1pt]
			\textbf{AVG} & 72.04                        & 70.97                        & 68.18                        & 68.09                          & 67.22                           & 66.53                   & 66.39                              & 66.11                               & 65.53                    & 64.23                         \\\bottomrule
		\end{tabular}}
\end{table}
\egroup


\bgroup
\def\arraystretch{1.5}
\begin{table}[t]
	\caption{Detailed results of non-targeted attacks on Citeseer (1)}
	\label{tab:eval_nontarget_detailed_citeseer1}
	\resizebox{\textwidth}{!}{
		\begin{tabular}{l*{10}{>{$}c<{$}}}
			\toprule
			             & \text{\scriptsize RGAT+LN} & \text{\scriptsize RGAT+FLAG+LN} & \text{\scriptsize EGuard+LNi+FLAG+LN} & \text{\scriptsize Guard+LNi+LN} & \text{\scriptsize RGAT} & \text{\scriptsize EGuard+FLAG+LN} & \text{\scriptsize RGAT+FLAG} & \text{\scriptsize EGuard+LNi+FLAG} & \text{\scriptsize EGuard+FLAG} & \text{\scriptsize GCN+LNi+FLAG+LN} \\ \midrule
			Clean        & 74.82                      & 75.72                           & 75.44                                 & 74.25                           & 74.85                   & 73.64                             & 75.56                        & 74.75                              & 73.57                          & 75.67                              \\\hdashline[0.5pt/1pt]
			PGD          & 71.00                      & 71.32                           & 75.19                                 & 74.21                           & 69.33                   & 73.55                             & 69.84                        & 74.83                              & 73.57                          & 57.97                              \\
			\hfill +HAO  & 71.00                      & 70.82                           & 66.07                                 & 73.04                           & 69.05                   & 61.55                             & 65.78                        & 50.01                              & 47.54                          & 58.77                              \\
			MetaGIA      & 70.32                      & 70.21                           & 75.15                                 & 74.21                           & 68.42                   & 73.55                             & 68.90                        & 74.83                              & 73.57                          & 56.36                              \\
			\hfill +HAO  & 70.37                      & 69.77                           & 64.00                                 & 71.25                           & 68.04                   & 59.94                             & 63.10                        & 49.70                              & 46.95                          & 57.17                              \\
			AGIA         & 71.45                      & 70.51                           & 75.29                                 & 74.21                           & 70.31                   & 73.60                             & 69.40                        & 74.83                              & 73.61                          & 56.50                              \\
			\hfill +HAO  & 71.80                      & 70.70                           & 64.54                                 & 70.58                           & 70.24                   & 59.32                             & 62.31                        & 50.33                              & 46.77                          & 58.02                              \\
			TDGIA        & 72.29                      & 73.81                           & 75.26                                 & 74.21                           & 70.99                   & 73.55                             & 73.34                        & 74.85                              & 73.57                          & 63.01                              \\
			\hfill +HAO  & 72.51                      & 70.18                           & 68.04                                 & 56.69                           & 60.91                   & 65.70                             & 53.99                        & 56.73                              & 52.86                          & 66.52                              \\
			ATDIGA       & 72.23                      & 72.82                           & 75.12                                 & 74.21                           & 70.61                   & 73.55                             & 72.37                        & 74.82                              & 73.54                          & 61.55                              \\
			\hfill +HAO  & 71.22                      & 69.63                           & 65.82                                 & 52.97                           & 61.08                   & 64.51                             & 53.76                        & 52.94                              & 51.20                          & 64.04                              \\\hdashline[0.5pt/1pt]
			\textbf{AVG} & 71.73                      & 71.41                           & 70.90                                 & 69.98                           & 68.53                   & 68.41                             & 66.21                        & 64.42                              & 62.43                          & 61.42                              \\\bottomrule
		\end{tabular}}
\end{table}
\egroup

\bgroup
\def\arraystretch{1.5}
\begin{table}[t]
	\caption{Detailed results of non-targeted attacks on Citeseer (2)}
	\label{tab:eval_nontarget_detailed_citeseer2}
	\resizebox{\textwidth}{!}{
		\begin{tabular}{l*{10}{>{$}c<{$}}}
			\toprule
			             & \text{\scriptsize Guard+LN} & \text{\scriptsize Guard+LNi} & \text{\scriptsize RobustGCN+FLAG} & \text{\scriptsize Guard} & \text{\scriptsize GCN+LNi+FLAG} & \text{\scriptsize Sage+LNi+FLAG+LN} & \text{\scriptsize GAT+LNi+FLAG+LN} & \text{\scriptsize RobustGCN} & \text{\scriptsize GCN+LNi+LN} & \text{\scriptsize Sage+LNi+FLAG} \\ \midrule
			Clean        & 73.97                       & 74.41                        & 75.87                             & 74.78                    & 75.45                           & 73.89                               & 75.60                              & 75.46                        & 74.65                         & 73.70                            \\\hdashline[0.5pt/1pt]
			PGD          & 74.07                       & 74.28                        & 53.81                             & 74.70                    & 47.56                           & 46.82                               & 45.00                              & 39.77                        & 40.69                         & 40.11                            \\
			\hfill +HAO  & 48.48                       & 38.91                        & 51.10                             & 33.83                    & 49.19                           & 46.93                               & 44.06                              & 39.72                        & 40.79                         & 40.88                            \\
			MetaGIA      & 74.07                       & 74.28                        & 53.11                             & 74.70                    & 47.14                           & 46.13                               & 44.76                              & 39.84                        & 40.87                         & 40.13                            \\
			\hfill +HAO  & 45.32                       & 38.98                        & 50.85                             & 33.95                    & 49.03                           & 46.42                               & 44.08                              & 39.79                        & 41.02                         & 40.90                            \\
			AGIA         & 74.07                       & 74.29                        & 53.12                             & 74.72                    & 47.30                           & 46.29                               & 44.07                              & 40.16                        & 41.76                         & 40.73                            \\
			\hfill +HAO  & 43.47                       & 41.04                        & 50.88                             & 36.51                    & 49.61                           & 47.28                               & 45.66                              & 41.53                        & 42.32                         & 42.82                            \\
			TDGIA        & 74.07                       & 74.28                        & 55.01                             & 74.76                    & 49.47                           & 47.06                               & 41.08                              & 37.94                        & 40.68                         & 36.21                            \\
			\hfill +HAO  & 36.83                       & 36.50                        & 60.37                             & 26.45                    & 57.45                           & 49.82                               & 49.74                              & 47.44                        & 43.85                         & 40.83                            \\
			ATDIGA       & 74.07                       & 74.21                        & 54.95                             & 74.72                    & 45.09                           & 41.89                               & 36.24                              & 34.65                        & 32.10                         & 31.17                            \\
			\hfill +HAO  & 30.21                       & 28.74                        & 55.40                             & 21.70                    & 52.22                           & 45.66                               & 45.19                              & 40.35                        & 35.05                         & 38.81                            \\\hdashline[0.5pt/1pt]
			\textbf{AVG} & 58.97                       & 57.27                        & 55.86                             & 54.62                    & 51.77                           & 48.93                               & 46.86                              & 43.33                        & 43.07                         & 42.39                            \\\bottomrule
		\end{tabular}}
\end{table}
\egroup


\bgroup
\def\arraystretch{1.6}
\begin{table}[t]
	\caption{Detailed results of non-targeted attacks on Computers (1)}
	\label{tab:eval_nontarget_detailed_computers1}
	\resizebox{\textwidth}{!}{
		\begin{tabular}{l*{10}{>{$}c<{$}}}
			\toprule
			             & \text{\scriptsize EGuard+LNi+FLAG+LN} & \text{\scriptsize Guard+LNi+LN} & \text{\scriptsize EGuard+FLAG+LN} & \text{\scriptsize Guard+LN} & \text{\scriptsize RGAT+FLAG+LN} & \text{\scriptsize RGAT+FLAG} & \text{\scriptsize EGuard+LNi+FLAG} & \text{\scriptsize Guard+LNi} & \text{\scriptsize RGAT+LN} & \text{\scriptsize RGAT} \\ \midrule
			Clean        & 91.04                                 & 90.88                           & 91.40                             & 91.23                       & 93.21                           & 93.32                        & 92.16                              & 91.95                        & 93.20                      & 93.17                   \\\hdashline[0.5pt/1pt]
			PGD          & 90.94                                 & 90.87                           & 91.41                             & 91.24                       & 81.59                           & 80.19                        & 88.24                              & 87.93                        & 79.68                      & 79.05                   \\
			\hfill +HAO  & 87.83                                 & 87.59                           & 80.41                             & 75.94                       & 81.80                           & 82.26                        & 64.18                              & 62.69                        & 79.29                      & 79.33                   \\
			MetaGIA      & 90.94                                 & 90.87                           & 91.41                             & 91.24                       & 81.58                           & 80.18                        & 88.23                              & 87.91                        & 79.68                      & 79.06                   \\
			\hfill +HAO  & 90.25                                 & 90.21                           & 90.11                             & 88.32                       & 81.64                           & 81.72                        & 78.11                              & 76.58                        & 79.29                      & 78.96                   \\
			AGIA         & 90.98                                 & 90.90                           & 91.40                             & 91.22                       & 78.09                           & 76.59                        & 88.25                              & 87.86                        & 76.62                      & 75.56                   \\
			\hfill +HAO  & 86.02                                 & 85.77                           & 75.97                             & 71.49                       & 77.55                           & 78.17                        & 63.96                              & 62.74                        & 75.23                      & 75.14                   \\
			TDGIA        & 90.97                                 & 90.91                           & 91.40                             & 91.24                       & 77.07                           & 75.40                        & 90.26                              & 89.94                        & 75.94                      & 74.66                   \\
			\hfill +HAO  & 90.42                                 & 90.34                           & 90.35                             & 89.00                       & 77.12                           & 76.61                        & 74.58                              & 74.22                        & 75.71                      & 74.77                   \\
			ATDIGA       & 90.97                                 & 90.90                           & 91.41                             & 91.24                       & 82.42                           & 81.77                        & 89.24                              & 88.84                        & 81.29                      & 80.76                   \\
			\hfill +HAO  & 84.60                                 & 83.93                           & 74.38                             & 69.33                       & 82.97                           & 83.50                        & 69.92                              & 68.50                        & 80.92                      & 80.86                   \\\hdashline[0.5pt/1pt]
			\textbf{AVG} & 89.54                                 & 89.38                           & 87.24                             & 85.59                       & 81.37                           & 80.88                        & 80.65                              & 79.92                        & 79.71                      & 79.21                   \\\bottomrule
		\end{tabular}}
\end{table}
\egroup

\bgroup
\def\arraystretch{1.6}
\begin{table}[t]
	\caption{Detailed results of non-targeted attacks on Computers (2)}
	\label{tab:eval_nontarget_detailed_computers2}
	\resizebox{\textwidth}{!}{
		\begin{tabular}{l*{10}{>{$}c<{$}}}
			\toprule
			             & \text{\scriptsize GAT+FLAG+LN} & \text{\scriptsize EGuard+FLAG} & \text{\scriptsize Guard} & \text{\scriptsize RobustGCN+FLAG} & \text{\scriptsize GAT+LNi+FLAG+LN} & \text{\scriptsize RobustGCN} & \text{\scriptsize Sage+LNi+FLAG+LN} & \text{\scriptsize GAT+LNi+FLAG} & \text{\scriptsize GCN+LNi+FLAG+LN} & \text{\scriptsize GAT+LNi+LN} \\ \midrule
			Clean        & 92.17                          & 91.68                          & 91.55                    & 92.46                             & 92.40                              & 92.24                        & 91.71                               & 92.45                           & 93.22                              & 92.05                         \\\hdashline[0.5pt/1pt]
			PGD          & 82.31                          & 85.82                          & 84.91                    & 73.27                             & 77.91                              & 67.14                        & 63.83                               & 67.61                           & 54.96                              & 52.20                         \\
			\hfill +HAO  & 69.83                          & 55.62                          & 54.31                    & 72.73                             & 65.08                              & 68.80                        & 62.55                               & 54.93                           & 63.28                              & 69.19                         \\
			MetaGIA      & 82.31                          & 85.81                          & 84.91                    & 73.28                             & 77.91                              & 67.14                        & 63.83                               & 67.62                           & 54.96                              & 52.21                         \\
			\hfill +HAO  & 77.39                          & 69.73                          & 67.90                    & 70.42                             & 69.52                              & 64.76                        & 62.45                               & 58.24                           & 59.31                              & 63.69                         \\
			AGIA         & 79.60                          & 86.08                          & 85.21                    & 71.95                             & 75.01                              & 66.01                        & 60.72                               & 64.25                           & 52.34                              & 50.69                         \\
			\hfill +HAO  & 63.02                          & 56.48                          & 55.35                    & 72.18                             & 61.22                              & 68.84                        & 60.68                               & 53.95                           & 62.78                              & 67.54                         \\
			TDGIA        & 80.42                          & 88.64                          & 88.32                    & 72.23                             & 75.27                              & 69.45                        & 63.87                               & 68.58                           & 64.96                              & 58.98                         \\
			\hfill +HAO  & 79.19                          & 69.75                          & 68.76                    & 71.39                             & 70.84                              & 69.11                        & 63.72                               & 63.45                           & 66.56                              & 65.81                         \\
			ATDIGA       & 82.42                          & 87.11                          & 86.03                    & 76.96                             & 79.13                              & 71.92                        & 68.42                               & 71.15                           & 66.01                              & 53.34                         \\
			\hfill +HAO  & 60.74                          & 61.46                          & 58.81                    & 76.79                             & 64.38                              & 74.26                        & 68.33                               & 57.90                           & 72.34                              & 73.82                         \\\hdashline[0.5pt/1pt]
			\textbf{AVG} & 77.22                          & 76.20                          & 75.10                    & 74.88                             & 73.52                              & 70.88                        & 66.37                               & 65.47                           & 64.61                              & 63.59                         \\\bottomrule
		\end{tabular}}
\end{table}
\egroup

\bgroup
\def\arraystretch{1.6}
\begin{table}[t]
	\caption{Detailed results of non-targeted attacks on Arxiv (1)}
	\label{tab:eval_nontarget_detailed_arxiv1}
	\resizebox{\textwidth}{!}{
		\begin{tabular}{l*{10}{>{$}c<{$}}}
			\toprule
			             & \text{\scriptsize Guard+LNi+LN} & \text{\scriptsize RGAT+LN} & \text{\scriptsize RGAT+FLAG+LN} & \text{\scriptsize EGuard+LNi+FLAG+LN} & \text{\scriptsize EGuard+FLAG+LN} & \text{\scriptsize Guard+LN} & \text{\scriptsize RobustGCN+FLAG} & \text{\scriptsize RobustGCN} & \text{\scriptsize GCN+LNi+FLAG+LN} & \text{\scriptsize Guard+LNi} \\ \hline
			             & 71.15                           & 70.95                      & 70.84                           & 69.50                                 & 69.46                             & 69.76                       & 67.85                             & 67.50                        & 71.40                              & 70.99                        \\\hdashline[0.5pt/1pt]
			PGD          & 71.11                           & 66.57                      & 66.61                           & 69.28                                 & 69.24                             & 69.62                       & 60.60                             & 60.81                        & 55.99                              & 70.26                        \\
			             & 68.68                           & 66.68                      & 66.60                           & 61.05                                 & 61.02                             & 58.92                       & 62.99                             & 62.89                        & 60.02                              & 47.84                        \\
			MetaGIA      & 71.09                           & 67.87                      & 67.67                           & 69.23                                 & 69.22                             & 69.59                       & 64.10                             & 64.10                        & 63.58                              & 70.40                        \\
			             & 69.97                           & 66.81                      & 66.52                           & 66.14                                 & 66.13                             & 65.70                       & 63.20                             & 63.30                        & 64.13                              & 58.58                        \\
			AGIA         & 70.97                           & 65.22                      & 64.46                           & 68.23                                 & 68.17                             & 68.57                       & 59.26                             & 59.23                        & 57.26                              & 64.60                        \\
			             & 63.57                           & 57.02                      & 56.60                           & 58.27                                 & 58.20                             & 57.73                       & 60.77                             & 60.72                        & 61.50                              & 58.08                        \\
			TDIGA        & 71.02                           & 67.54                      & 67.28                           & 68.37                                 & 68.33                             & 68.72                       & 63.70                             & 63.56                        & 61.01                              & 65.63                        \\
			             & 64.31                           & 61.61                      & 60.99                           & 59.73                                 & 59.74                             & 58.33                       & 63.08                             & 63.30                        & 62.81                              & 53.04                        \\
			ATDGIA       & 71.01                           & 68.49                      & 68.45                           & 68.18                                 & 68.14                             & 68.49                       & 64.95                             & 64.88                        & 63.95                              & 66.39                        \\
			             & 69.92                           & 68.67                      & 68.58                           & 66.34                                 & 66.35                             & 65.47                       & 65.56                             & 65.62                        & 65.83                              & 55.42                        \\\hdashline[0.5pt/1pt]
			\textbf{AVG} & 69.34                           & 66.13                      & 65.87                           & 65.85                                 & 65.82                             & 65.54                       & 63.28                             & 63.26                        & 62.50                              & 61.93                        \\\bottomrule
		\end{tabular}}
\end{table}
\egroup

\bgroup
\def\arraystretch{1.5}
\begin{table}[t]
	\caption{Detailed results of non-targeted attacks on Arxiv (2)}
	\label{tab:eval_nontarget_detailed_arxiv2}
	\resizebox{\textwidth}{!}{
		\begin{tabular}{l*{10}{>{$}c<{$}}}
			\toprule
			             & \text{\scriptsize RGAT+FLAG} & \text{\scriptsize GCN+LNi+LN} & \text{\scriptsize RGAT} & \text{\scriptsize GCN+FLAG+LN} & \text{\scriptsize GAT+FLAG+LN} & \text{\scriptsize EGuard+LNi+FLAG} & \text{\scriptsize GCN+LN} & \text{\scriptsize EGuard+FLAG} & \text{\scriptsize GCN+LNi+FLAG} & \text{\scriptsize GAT+LNi+FLAG+LN} \\ \midrule
			             & 70.63                        & 71.38                         & 70.77                   & 70.00                          & 70.28                          & 69.37                              & 70.42                     & 69.34                          & 71.31                           & 71.00                              \\\hdashline[0.5pt/1pt]
			PGD          & 66.49                        & 54.46                         & 66.26                   & 54.21                          & 57.44                          & 68.04                              & 51.97                     & 68.03                          & 48.00                           & 57.65                              \\
			             & 57.18                        & 58.40                         & 55.38                   & 55.51                          & 59.16                          & 37.02                              & 52.45                     & 36.80                          & 52.75                           & 53.97                              \\
			MetaGIA      & 67.42                        & 62.88                         & 67.68                   & 58.54                          & 61.92                          & 68.48                              & 57.04                     & 68.40                          & 55.73                           & 61.56                              \\
			             & 58.21                        & 63.35                         & 57.05                   & 59.65                          & 51.65                          & 50.32                              & 57.39                     & 50.23                          & 57.72                           & 54.63                              \\
			AGIA         & 63.75                        & 57.12                         & 64.49                   & 49.55                          & 45.96                          & 59.35                              & 48.54                     & 59.25                          & 54.55                           & 49.14                              \\
			             & 50.31                        & 61.29                         & 49.36                   & 58.25                          & 49.71                          & 49.24                              & 57.24                     & 49.20                          & 58.10                           & 48.78                              \\
			TDIGA        & 66.74                        & 58.91                         & 66.95                   & 55.47                          & 56.30                          & 62.18                              & 52.39                     & 62.10                          & 48.86                           & 52.58                              \\
			             & 47.88                        & 61.90                         & 45.59                   & 59.20                          & 49.44                          & 45.08                              & 56.42                     & 44.91                          & 54.68                           & 47.80                              \\
			ATDGIA       & 67.97                        & 62.21                         & 68.07                   & 58.61                          & 63.36                          & 62.73                              & 55.26                     & 62.67                          & 54.19                           & 58.50                              \\
			             & 60.82                        & 64.82                         & 59.32                   & 62.69                          & 57.51                          & 46.94                              & 59.50                     & 46.83                          & 57.90                           & 56.58                              \\\hdashline[0.5pt/1pt]
			\textbf{AVG} & 61.58                        & 61.52                         & 60.99                   & 58.33                          & 56.61                          & 56.25                              & 56.24                     & 56.16                          & 55.80                           & 55.65                              \\\bottomrule
		\end{tabular}}
\end{table}
\egroup



\subsection{Detailed Results of Targeted Attacks}
\label{sec:eval_target_detailed}
In this section, we present the detailed targeted attack results of the methods and datasets used in our experiments for Table~\ref{tab:eval_targeted}.
For simiplicity, we only give the results of top $20$ robust models according to the averaged test accuracy against all attacks.


\bgroup
\def\arraystretch{1.5}
\begin{table}[t]
	\caption{Detailed results of targeted attacks on Computers (1)}
	\label{tab:eval_target_detailed_computers1}
	\resizebox{\textwidth}{!}{
		\begin{tabular}{l*{10}{>{$}c<{$}}}
			\toprule
			             & \text{\scriptsize EGuard+LNi+FLAG+LN} & \text{\scriptsize Guard+LNi+LN} & \text{\scriptsize EGuard+FLAG+LN} & \text{\scriptsize Guard+LN} & \text{\scriptsize Guard+LNi} & \text{\scriptsize EGuard+LNi+FLAG} & \text{\scriptsize RobustGCN+FLAG} & \text{\scriptsize RGAT+FLAG} & \text{\scriptsize RGAT+FLAG+LN} & \text{\scriptsize EGuard+FLAG} \\ \midrule
			Clean        & 90.96                                 & 90.76                           & 91.56                             & 91.11                       & 91.12                        & 91.29                              & 91.85                             & 92.83                        & 92.78                           & 90.75                          \\\hdashline[0.5pt/1pt]
			PGD          & 90.96                                 & 90.76                           & 91.56                             & 91.11                       & 89.38                        & 89.54                              & 72.36                             & 72.17                        & 74.28                           & 88.36                          \\
			\hfill +HAO  & 85.81                                 & 85.75                           & 79.51                             & 73.71                       & 65.01                        & 64.15                              & 72.58                             & 74.40                        & 74.08                           & 56.50                          \\
			MetaGIA      & 90.96                                 & 90.76                           & 91.56                             & 91.11                       & 88.93                        & 89.10                              & 73.81                             & 70.58                        & 72.24                           & 88.10                          \\
			\hfill +HAO  & 85.83                                 & 85.69                           & 78.46                             & 72.61                       & 65.62                        & 65.53                              & 73.50                             & 72.10                        & 72.00                           & 56.12                          \\
			AGIA         & 91.00                                 & 90.82                           & 91.58                             & 91.06                       & 89.11                        & 89.33                              & 72.96                             & 68.85                        & 69.64                           & 88.00                          \\
			\hfill +HAO  & 85.72                                 & 85.71                           & 79.50                             & 74.28                       & 64.71                        & 63.90                              & 73.12                             & 72.61                        & 72.22                           & 56.18                          \\
			TDGIA        & 90.96                                 & 90.76                           & 91.56                             & 91.11                       & 89.15                        & 89.36                              & 72.06                             & 72.42                        & 72.58                           & 87.75                          \\
			\hfill +HAO  & 77.15                                 & 75.64                           & 65.21                             & 62.97                       & 69.78                        & 70.43                              & 73.08                             & 74.33                        & 74.00                           & 64.31                          \\
			ATDIGA       & 90.96                                 & 90.76                           & 91.56                             & 91.11                       & 88.99                        & 89.22                              & 75.15                             & 75.68                        & 73.32                           & 88.43                          \\
			\hfill +HAO  & 78.35                                 & 77.67                           & 62.87                             & 59.65                       & 63.75                        & 63.15                              & 74.06                             & 75.78                        & 74.14                           & 56.51                          \\\hdashline[0.5pt/1pt]
			\textbf{AVG} & 87.15                                 & 86.83                           & 83.18                             & 80.89                       & 78.69                        & 78.64                              & 74.96                             & 74.70                        & 74.66                           & 74.64                          \\\bottomrule
		\end{tabular}}
\end{table}
\egroup

\bgroup
\def\arraystretch{1.5}
\begin{table}[t]
	\caption{Detailed results of targeted attacks on Computers (2)}
	\label{tab:eval_target_detailed_computers2}
	\resizebox{\textwidth}{!}{
		\begin{tabular}{l*{10}{>{$}c<{$}}}
			\toprule
			             & \text{\scriptsize Guard} & \text{\scriptsize RobustGCN} & \text{\scriptsize RGAT} & \text{\scriptsize RGAT+LN} & \text{\scriptsize GAT+FLAG+LN} & \text{\scriptsize GAT+LNi+FLAG+LN} & \text{\scriptsize GAT+LNi+FLAG} & \text{\scriptsize GCN+LNi+FLAG+LN} & \text{\scriptsize GAT+LNi+LN} & \text{\scriptsize GCN+LNi+FLAG} \\ \midrule
			Clean        & 90.50                    & 92.07                        & 92.68                   & 92.76                      & 91.07                          & 91.90                              & 91.92                           & 92.25                              & 91.56                         & 92.35                           \\\hdashline[0.5pt/1pt]
			PGD          & 88.13                    & 70.40                        & 71.85                   & 72.65                      & 77.69                          & 75.25                              & 72.57                           & 63.08                              & 58.46                         & 60.79                           \\
			\hfill +HAO  & 54.96                    & 70.76                        & 71.78                   & 71.40                      & 71.03                          & 66.01                              & 62.46                           & 66.01                              & 70.49                         & 64.17                           \\
			MetaGIA      & 87.67                    & 71.78                        & 70.44                   & 71.33                      & 74.93                          & 73.12                              & 70.89                           & 62.54                              & 57.40                         & 60.71                           \\
			\hfill +HAO  & 55.00                    & 71.61                        & 70.21                   & 70.35                      & 69.56                          & 64.82                              & 62.58                           & 64.81                              & 67.57                         & 63.04                           \\
			AGIA         & 87.57                    & 70.92                        & 68.36                   & 68.58                      & 73.00                          & 71.03                              & 68.50                           & 61.08                              & 56.62                         & 59.26                           \\
			\hfill +HAO  & 54.89                    & 71.58                        & 69.96                   & 69.99                      & 68.44                          & 64.81                              & 61.00                           & 64.68                              & 69.39                         & 62.28                           \\
			TDGIA        & 87.21                    & 69.86                        & 71.54                   & 71.28                      & 74.24                          & 72.86                              & 70.60                           & 62.74                              & 57.54                         & 60.35                           \\
			\hfill +HAO  & 61.62                    & 71.62                        & 71.39                   & 71.92                      & 54.19                          & 60.51                              & 66.69                           & 66.79                              & 66.74                         & 63.97                           \\
			ATDIGA       & 87.85                    & 73.33                        & 74.39                   & 72.19                      & 73.36                          & 75.24                              & 74.06                           & 65.14                              & 56.22                         & 62.67                           \\
			\hfill +HAO  & 54.93                    & 72.53                        & 72.00                   & 71.49                      & 62.03                          & 63.19                              & 62.14                           & 68.50                              & 73.15                         & 66.06                           \\\hdashline[0.5pt/1pt]
			\textbf{AVG} & 73.67                    & 73.31                        & 73.15                   & 73.09                      & 71.78                          & 70.79                              & 69.40                           & 67.06                              & 65.92                         & 65.06                           \\\bottomrule
		\end{tabular}}
\end{table}
\egroup


\bgroup
\def\arraystretch{1.6}
\begin{table}[t]
	\caption{Detailed results of targeted attacks on Arxiv (1)}
	\label{tab:eval_target_detailed_arxiv1}
	\resizebox{\textwidth}{!}{
		\begin{tabular}{l*{10}{>{$}c<{$}}}
			\toprule
			             & \multicolumn{1}{l}{Guard+LNi+LN} & \multicolumn{1}{l}{EGuard+LNi+FLAG+LN} & \multicolumn{1}{l}{Guard+LNi} & \multicolumn{1}{l}{EGuard+FLAG+LN} & \multicolumn{1}{l}{EGuard+LNi+FLAG} & \multicolumn{1}{l}{Guard+LN} & \multicolumn{1}{l}{EGuard+FLAG} & \multicolumn{1}{l}{Guard} & \multicolumn{1}{l}{RobustGCN+FLAG} & \multicolumn{1}{l}{RGAT} \\ \midrule
			             & 71.34                            & 71.22                                  & 71.22                         & 69.59                              & 70.59                               & 69.78                        & 68.88                           & 69.41                     & 67.28                              & 67.03                    \\\hdashline[0.5pt/1pt]
			PGD          & 71.31                            & 71.16                                  & 71.16                         & 69.47                              & 70.47                               & 69.69                        & 68.69                           & 69.19                     & 39.91                              & 39.13                    \\
			             & 69.38                            & 65.69                                  & 33.78                         & 47.41                              & 29.12                               & 38.00                        & 14.31                           & 13.94                     & 36.12                              & 36.06                    \\
			MetaGIA      & 71.03                            & 71.22                                  & 70.53                         & 69.59                              & 70.59                               & 69.78                        & 68.84                           & 69.28                     & 42.56                              & 41.81                    \\
			             & 42.56                            & 48.06                                  & 33.94                         & 31.84                              & 34.94                               & 26.75                        & 20.34                           & 18.28                     & 38.66                              & 38.44                    \\
			AGIA         & 71.06                            & 70.94                                  & 70.19                         & 69.25                              & 67.72                               & 69.38                        & 64.38                           & 63.66                     & 39.94                              & 39.47                    \\
			             & 38.56                            & 37.22                                  & 35.06                         & 24.63                              & 35.31                               & 22.09                        & 16.19                           & 14.09                     & 42.53                              & 42.56                    \\
			TDIGA        & 71.00                            & 71.16                                  & 69.78                         & 68.97                              & 68.22                               & 69.41                        & 66.09                           & 66.12                     & 41.25                              & 41.31                    \\
			             & 38.72                            & 34.19                                  & 38.78                         & 23.41                              & 33.94                               & 20.78                        & 17.66                           & 16.06                     & 38.38                              & 38.28                    \\
			ATDGIA       & 71.06                            & 70.88                                  & 70.56                         & 69.19                              & 69.03                               & 69.56                        & 66.09                           & 66.19                     & 44.06                              & 43.75                    \\
			             & 68.97                            & 61.03                                  & 37.88                         & 41.69                              & 33.69                               & 34.25                        & 19.16                           & 17.28                     & 39.03                              & 38.84                    \\\hdashline[0.5pt/1pt]
			\textbf{AVG} & 62.27                            & 61.16                                  & 54.81                         & 53.19                              & 53.06                               & 50.86                        & 44.60                           & 43.95                     & 42.70                              & 42.43                    \\\bottomrule
		\end{tabular}}
\end{table}
\egroup

\bgroup
\def\arraystretch{1.5}
\begin{table}[t]
	\caption{Detailed results of targeted attacks on Arxiv (2)}
	\label{tab:eval_target_detailed_arxiv2}
	\resizebox{\textwidth}{!}{
		\begin{tabular}{l*{10}{>{$}c<{$}}}
			\toprule
			             & \multicolumn{1}{l}{RobustGCN} & \multicolumn{1}{l}{RGAT+LN} & \multicolumn{1}{l}{RGAT+FLAG+LN} & \multicolumn{1}{l}{GCN+LNi+FLAG} & \multicolumn{1}{l}{RGAT+FLAG} & \multicolumn{1}{l}{GCN+LNi+LN} & \multicolumn{1}{l}{GCN+LNi} & \multicolumn{1}{l}{GCN+LNi+FLAG+LN} & \multicolumn{1}{l}{GAT+LN} & \multicolumn{1}{l}{GAT+FLAG+LN} \\ \midrule
			             & 67.69                         & 72.06                       & 71.41                            & 71.34                            & 71.16                         & 71.97                          & 71.59                       & 71.75                               & 69.94                      & 69.94                           \\\hdashline[0.5pt/1pt]
			PGD          & 38.66                         & 40.31                       & 38.06                            & 32.19                            & 37.78                         & 29.09                          & 29.97                       & 29.72                               & 36.34                      & 38.84                           \\
			             & 37.22                         & 37.06                       & 34.28                            & 32.75                            & 23.69                         & 28.91                          & 29.56                       & 29.28                               & 28.88                      & 30.47                           \\
			MetaGIA      & 35.00                         & 42.56                       & 41.28                            & 30.28                            & 41.03                         & 28.91                          & 28.59                       & 28.50                               & 16.00                      & 14.84                           \\
			             & 33.22                         & 34.09                       & 32.53                            & 30.03                            & 27.81                         & 27.50                          & 27.97                       & 27.47                               & 19.44                      & 21.50                           \\
			AGIA         & 41.06                         & 42.12                       & 42.06                            & 32.53                            & 39.75                         & 33.09                          & 32.56                       & 31.84                               & 23.84                      & 21.12                           \\
			             & 41.97                         & 23.84                       & 23.66                            & 35.19                            & 23.03                         & 34.03                          & 34.47                       & 34.25                               & 16.97                      & 14.94                           \\
			TDIGA        & 44.28                         & 43.84                       & 43.91                            & 36.31                            & 42.12                         & 36.34                          & 35.12                       & 36.16                               & 27.38                      & 24.50                           \\
			             & 40.81                         & 32.38                       & 31.50                            & 39.47                            & 28.31                         & 38.50                          & 38.62                       & 37.91                               & 27.56                      & 29.28                           \\
			ATDGIA       & 43.12                         & 44.34                       & 44.22                            & 34.47                            & 41.91                         & 33.53                          & 33.44                       & 33.28                               & 31.06                      & 24.19                           \\
			             & 37.97                         & 39.00                       & 37.84                            & 33.84                            & 30.19                         & 30.53                          & 30.47                       & 30.59                               & 30.28                      & 33.69                           \\\hdashline[0.5pt/1pt]
			\textbf{AVG} & 41.91                         & 41.05                       & 40.07                            & 37.13                            & 36.98                         & 35.67                          & 35.67                       & 35.52                               & 29.79                      & 29.39                           \\\bottomrule
		\end{tabular}}
\end{table}
\egroup


\bgroup
\def\arraystretch{1.5}
\begin{table}[t]
	\caption{Detailed results of targeted attacks on Aminer (1)}
	\label{tab:eval_target_detailed_aminer1}
	\resizebox{\textwidth}{!}{
		\begin{tabular}{l*{10}{>{$}c<{$}}}
			\toprule
			             & \text{\scriptsize EGuard+LNi+FLAG} & \text{\scriptsize EGuard+LNi+FLAG+LN} & \text{\scriptsize Guard+LNi} & \text{\scriptsize Guard+LNi+LN} & \text{\scriptsize EGuard+FLAG} & \text{\scriptsize Guard} & \text{\scriptsize RGAT+FLAG} & \text{\scriptsize Guard+LN} & \text{\scriptsize EGuard+FLAG+LN} & \text{\scriptsize RGAT} \\ \midrule
			             & 59.03                              & 58.06                                 & 60.72                        & 60.85                           & 57.06                          & 57.25                    & 61.75                        & 58.50                       & 58.81                             & 62.78                   \\\hdashline[0.5pt/1pt]
			PGD          & 55.25                              & 48.47                                 & 56.31                        & 49.40                           & 53.03                          & 53.16                    & 41.84                        & 49.72                       & 48.31                             & 40.72                   \\
			             & 39.06                              & 39.47                                 & 37.03                        & 39.40                           & 35.16                          & 34.62                    & 33.53                        & 29.69                       & 29.97                             & 31.75                   \\
			MetaGIA      & 52.09                              & 50.66                                 & 52.35                        & 49.81                           & 49.03                          & 48.97                    & 46.19                        & 48.34                       & 47.59                             & 45.81                   \\
			             & 42.09                              & 45.16                                 & 40.26                        & 43.42                           & 37.00                          & 37.09                    & 41.47                        & 36.88                       & 36.62                             & 41.12                   \\
			AGIA         & 54.06                              & 48.00                                 & 54.82                        & 48.17                           & 51.28                          & 51.34                    & 48.72                        & 48.78                       & 47.59                             & 48.25                   \\
			             & 26.44                              & 29.94                                 & 23.25                        & 28.08                           & 19.84                          & 18.97                    & 26.50                        & 23.19                       & 24.06                             & 25.78                   \\
			TDIGA        & 52.75                              & 46.72                                 & 53.68                        & 46.92                           & 50.75                          & 50.87                    & 42.50                        & 47.66                       & 46.28                             & 40.81                   \\
			             & 24.31                              & 28.91                                 & 18.54                        & 26.07                           & 16.12                          & 15.06                    & 24.00                        & 19.69                       & 20.66                             & 22.5                    \\
			ATDGIA       & 53.44                              & 51.00                                 & 53.69                        & 49.32                           & 50.34                          & 50.50                    & 45.44                        & 49.97                       & 49.59                             & 45.25                   \\
			             & 38.19                              & 42.66                                 & 35.93                        & 41.07                           & 33.72                          & 33.72                    & 36.72                        & 31.91                       & 31.69                             & 35.94                   \\\hdashline[0.5pt/1pt]
			\textbf{AVG} & 45.16                              & 44.46                                 & 44.23                        & 43.86                           & 41.21                          & 41.05                    & 40.79                        & 40.39                       & 40.11                             & 40.06                   \\\bottomrule
		\end{tabular}}
\end{table}
\egroup

\bgroup
\def\arraystretch{1.5}
\begin{table}[t]
	\caption{Detailed results of targeted attacks on Aminer (2)}
	\label{tab:eval_target_detailed_aminer2}
	\resizebox{\textwidth}{!}{
		\begin{tabular}{l*{10}{>{$}c<{$}}}
			\toprule
			             & \text{\scriptsize RGAT+FLAG+LN} & \text{\scriptsize GCN+LNi+FLAG+LN} & \text{\scriptsize RGAT+LN} & \text{\scriptsize Sage+LNi+FLAG+LN} & \text{\scriptsize GCN+LNi+FLAG} & \text{\scriptsize GCN+LNi+LN} & \text{\scriptsize Sage+LNi+LN} & \text{\scriptsize GAT+LNi+LN} & \text{\scriptsize GAT+LNi+FLAG+LN} & \text{\scriptsize Sage+LNi+FLAG} \\ \midrule
			             & 62.66                           & 64.41                              & 63.78                      & 65.56                               & 63.91                           & 66.88                         & 65.44                          & 66.97                         & 65.78                              & 64.34                            \\\hdashline[0.5pt/1pt]
			PGD          & 31.97                           & 28.03                              & 29.75                      & 26.22                               & 26.81                           & 22.65                         & 23.78                          & 17.00                         & 16.66                              & 22.03                            \\
			             & 29.06                           & 28.16                              & 27.06                      & 26.44                               & 26.81                           & 23.17                         & 23.88                          & 17.58                         & 16.53                              & 22.06                            \\
			MetaGIA      & 41.38                           & 41.12                              & 40.78                      & 37.56                               & 36.72                           & 38.17                         & 36.56                          & 38.40                         & 37.31                              & 31.25                            \\
			             & 39.62                           & 42.16                              & 38.03                      & 37.38                               & 36.03                           & 37.89                         & 36.03                          & 37.60                         & 37.31                              & 31.12                            \\
			AGIA         & 38.34                           & 34.62                              & 37.47                      & 31.94                               & 33.97                           & 31.21                         & 31.31                          & 29.96                         & 29.62                              & 29.50                            \\
			             & 28.19                           & 29.03                              & 27.06                      & 27.19                               & 28.00                           & 27.14                         & 26.31                          & 22.00                         & 21.09                              & 25.25                            \\
			TDIGA        & 30.47                           & 28.44                              & 28.25                      & 24.41                               & 24.97                           & 20.85                         & 22.19                          & 15.39                         & 15.16                              & 20.56                            \\
			             & 27.12                           & 27.53                              & 24.97                      & 24.56                               & 24.84                           & 22.19                         & 22.22                          & 15.75                         & 14.03                              & 20.16                            \\
			ATDGIA       & 39.28                           & 36.62                              & 38.03                      & 33.38                               & 32.09                           & 32.44                         & 32.47                          & 34.83                         & 35.12                              & 27.62                            \\
			             & 32.66                           & 37.72                              & 31.50                      & 31.87                               & 31.78                           & 32.00                         & 30.72                          & 33.97                         & 33.06                              & 26.12                            \\\hdashline[0.5pt/1pt]
			\textbf{AVG} & 36.43                           & 36.17                              & 35.15                      & 33.32                               & 33.27                           & 32.24                         & 31.90                          & 29.95                         & 29.24                              & 29.09                            \\\bottomrule
		\end{tabular}}
\end{table}
\egroup

\bgroup
\def\arraystretch{1.5}
\begin{table}[t]
	\caption{Detailed results of targeted attacks on Reddit (1)}
	\label{tab:eval_target_detailed_reddit1}
	\resizebox{\textwidth}{!}{
		\begin{tabular}{l*{10}{>{$}c<{$}}}
			\toprule
			             & \text{\scriptsize Guard+LNi+LN} & \text{\scriptsize RobustGCN} & \text{\scriptsize RobustGCN+FLAG} & \text{\scriptsize Guard+LNi} & \text{\scriptsize Guard+LN} & \text{\scriptsize EGuard+LNi+FLAG+LN} & \text{\scriptsize EGuard+FLAG+LN} & \text{\scriptsize Sage+LNi+FLAG+LN} & \text{\scriptsize Guard} & \text{\scriptsize EGuard+FLAG} \\ \midrule
			             & 94.47                           & 95.08                        & 95.30                             & 94.42                        & 94.61                       & 94.61                                 & 94.60                             & 97.10                               & 94.05                    & 94.08                          \\\hdashline[0.5pt/1pt]
			PGD          & 92.91                           & 84.81                        & 83.84                             & 93.03                        & 92.69                       & 92.69                                 & 92.53                             & 76.25                               & 92.44                    & 92.72                          \\
			             & 80.03                           & 86.12                        & 84.94                             & 75.53                        & 68.53                       & 69.31                                 & 69.34                             & 75.25                               & 56.44                    & 58.03                          \\
			MetaGIA      & 93.53                           & 88.25                        & 87.22                             & 93.28                        & 93.38                       & 93.66                                 & 93.59                             & 80.72                               & 92.40                    & 92.88                          \\
			             & 77.47                           & 90.06                        & 90.44                             & 69.91                        & 65.28                       & 68.00                                 & 68.34                             & 83.62                               & 46.75                    & 48.59                          \\
			AGIA         & 93.62                           & 86.09                        & 87.84                             & 92.84                        & 93.16                       & 92.78                                 & 92.69                             & 81.59                               & 92.19                    & 91.31                          \\
			             & 88.66                           & 85.06                        & 87.84                             & 85.34                        & 83.09                       & 77.06                                 & 77.31                             & 72.19                               & 78.16                    & 67.06                          \\
			TDIGA        & 93.03                           & 90.19                        & 89.91                             & 92.25                        & 92.59                       & 92.91                                 & 92.53                             & 80.94                               & 91.25                    & 91.59                          \\
			             & 86.03                           & 89.06                        & 88.91                             & 80.38                        & 78.69                       & 81.56                                 & 81.25                             & 79.78                               & 64.09                    & 66.62                          \\
			ATDGIA       & 93.34                           & 87.34                        & 84.91                             & 92.38                        & 92.69                       & 93.97                                 & 93.81                             & 76.53                               & 91.62                    & 93.00                          \\
			             & 90.78                           & 88.84                        & 88.38                             & 87.94                        & 88.06                       & 79.44                                 & 79.25                             & 78.66                               & 80.69                    & 63.22                          \\\hdashline[0.5pt/1pt]
			\textbf{AVG} & 89.44                           & 88.26                        & 88.14                             & 87.03                        & 85.71                       & 85.09                                 & 85.02                             & 80.24                               & 80.01                    & 78.10                          \\\bottomrule
		\end{tabular}}
\end{table}
\egroup

\bgroup
\def\arraystretch{1.5}
\begin{table}[t]
	\caption{Detailed results of targeted attacks on Reddit (2)}
	\label{tab:eval_target_detailed_reddit2}
	\resizebox{\textwidth}{!}{
		\begin{tabular}{l*{10}{>{$}c<{$}}}
			\toprule
			             & \text{\scriptsize EGuard+LNi+FLAG} & \text{\scriptsize Sage+LNi+LN} & \text{\scriptsize GAT+LNi+FLAG+LN} & \text{\scriptsize Sage+FLAG+LN} & \text{\scriptsize Sage+LN} & \text{\scriptsize GAT+LNi+LN} & \text{\scriptsize GAT+FLAG+LN} & \text{\scriptsize GAT+LN} & \text{\scriptsize Sage+LNi+FLAG} & \text{\scriptsize GCN+LNi+FLAG+LN} \\ \midrule
			             & 94.07                              & 97.10                          & 95.19                              & 97.13                           & 97.11                      & 95.37                         & 94.49                          & 94.77                     & 97.09                            & 95.84                              \\\hdashline[0.5pt/1pt]
			PGD          & 92.69                              & 74.94                          & 75.91                              & 67.47                           & 63.75                      & 70.38                         & 73.53                          & 78.12                     & 57.16                            & 71.28                              \\
			             & 58.12                              & 73.91                          & 79.59                              & 67.72                           & 64.72                      & 72.91                         & 78.16                          & 76.47                     & 56.62                            & 70.91                              \\
			MetaGIA      & 92.84                              & 78.63                          & 68.16                              & 84.03                           & 82.53                      & 67.28                         & 59.91                          & 62.94                     & 65.69                            & 62.13                              \\
			             & 48.69                              & 80.56                          & 78.84                              & 80.06                           & 76.59                      & 75.22                         & 74.34                          & 66.12                     & 69.59                            & 59.66                              \\
			AGIA         & 91.31                              & 69.50                          & 59.53                              & 62.66                           & 57.19                      & 51.75                         & 43.22                          & 50.28                     & 67.88                            & 59.28                              \\
			             & 66.97                              & 58.47                          & 74.19                              & 51.16                           & 49.19                      & 51.12                         & 72.91                          & 46.19                     & 55.75                            & 52.53                              \\
			TDIGA        & 91.59                              & 78.09                          & 73.12                              & 74.00                           & 68.62                      & 70.34                         & 64.81                          & 73.00                     & 65.28                            & 58.84                              \\
			             & 66.41                              & 77.22                          & 73.91                              & 75.72                           & 71.75                      & 69.72                         & 64.75                          & 67.97                     & 65.44                            & 58.09                              \\
			ATDGIA       & 93.03                              & 73.31                          & 64.25                              & 68.44                           & 63.59                      & 64.53                         & 53.66                          & 57.91                     & 65.12                            & 62.34                              \\
			             & 63.34                              & 73.78                          & 72.53                              & 69.62                           & 65.00                      & 65.22                         & 62.97                          & 65.50                     & 63.66                            & 57.97                              \\\hdashline[0.5pt/1pt]
			\textbf{AVG} & 78.10                              & 75.96                          & 74.11                              & 72.55                           & 69.09                      & 68.53                         & 67.52                          & 67.21                     & 66.30                            & 64.44                              \\\bottomrule
		\end{tabular}}
\end{table}
\egroup
